# Supplementary material for: Topological and disorder corrections to the transverse Wiedemann-Franz law and Mott relation in kagome magnets
Source: arXiv:2303.06939 source file (2023-03-13)
Supplement: Supplementary file 1 [file Supplemental_Material.pdf]

# Supplemental Material for "Topological and disorder corrections to the transverse Wiedemann-Franz law and Mott relation in kagome magnets"

Xiao-Bin Qiang,[1,2,3,4] Z. Z. Du,[1,3,4] Hai-Zhou Lu,[1,2,3,4,*] and X. C. Xie[5,6,7]

[1] *Shenzhen Institute for Quantum Science and Engineering and Department of Physics, Southern University of Science and Technology (SUSTech), Shenzhen 518055, China*
[2] *Quantum Science Center of Guangdong-Hong Kong-Macao Greater Bay Area (Guangdong), Shenzhen 518045, China*
[3] *Shenzhen Key Laboratory of Quantum Science and Engineering, Shenzhen 518055, China*
[4] *International Quantum Academy, Shenzhen 518048, China*
[5] *International Center for Quantum Materials, School of Physics, Peking University, Beijing 100871, China*
[6] *Collaborative Innovation Center of Quantum Matter, Beijing 100871, China*
[7] *CAS Center for Excellence in Topological Quantum Computation, University of Chinese Academy of Sciences, Beijing 100190, China*

(Dated: March 13, 2023)

In this Supplemental Material, we present the detailed calculations. For a self-contained presentation, the calculations of the disorder corrections to the electric and thermoelectric Hall conductivities in [1–3] (Refs. [32], [45], [46] in the main text) are also included in Secs. SII and SIII, but our approach of calculation is slightly different.

## CONTENTS

SI. Boltzmann kinetics S2
  A. Electric field S2
  B. Temperature gradient S4

SII. Anomalous electric Hall effect S5
  A. Intrinsic contribution S6
  B. Side-jump contribution S7
  C. Skew-scattering contribution S8
  D. Anomalous electric Hall conductivity S10

SIII. Anomalous thermoelectric Hall effect S11
  A. Intrinsic contribution S11
  B. Side-jump contribution S12
  C. Skew-scattering contribution S13
  D. Anomalous thermoelectric Hall conductivity S14

SIV. Anomalous Thermal Hall effect S15
  A. Intrinsic contribution S15
  B. Side-jump contribution S15
  C. Skew-scattering contribution S16
  D. Anomalous thermal Hall conductivity S16

SV. 2-Band system S16
  A. Eigen solutions S16
  B. Scattering rate S17
    1. Second-order scattering rate S19
    2. Third-order scattering rate S19
    3. Fourth-order scattering rate S20
  C. Coordinate shift S23

SVI. 2D massive Dirac model S25

* Corresponding author: luhz@sustech.edu.cn

A. Eigen solutions S25
B. Anomalous electric Hall conductivity S25
1. Intrinsic contribution S27
2. Side-jump contribution S27
3. Skew-scattering contribution S28
C. Transport coefficients S30
D. Wiedemann-Franz law S32
E. Mott relation S35

SVII. Tilted Weyl node S35
A. Eigen solutions S35
B. Anomalous Hall conductivity S36
1. Intrinsic contribution S37
2. Side-jump contribution S38
3. Skew-scattering contribution S40
C. Transport coefficients S41

References S42

## SI. BOLTZMANN KINETICS

### A. Electric field

At the steady state, i.e., $\partial f_l/\partial t = 0$, the Boltzmann equation reads

$$\dot{\mathbf{r}} \cdot \frac{\partial f_l}{\partial \mathbf{r}} + \dot{\mathbf{k}} \cdot \frac{\partial f_l}{\partial \mathbf{k}} = \mathcal{I}_{el}\{f_l\}, \tag{S1}$$

where $f_l$ is the non-equilibrium distribution function, $l = (\mathbf{k}, n)$ as the combined index (momentum, band), $f^0$ and $f_l^0$ represent Fermi-Dirac distribution function with energy dependence $\varepsilon$ and $\varepsilon_l$, respectively. We consider electric field $\mathbf{E}$ as the driving force, i.e., homogeneous case $\partial f_l/\partial \mathbf{r} = 0$, then the Boltzmann equation becomes

$$\dot{\mathbf{k}} \cdot \frac{\partial f_l}{\partial \mathbf{k}} = \mathcal{I}_{el}\{f_l\}. \tag{S2}$$

The r.h.s. is called collision term, which can be formally written as

$$\mathcal{I}_{el}\{f_l\} = -\sum_{l'} (\varpi_{l'l} f_l - \varpi_{ll'} f_{l'}), \tag{S3}$$

where $\sum_l \equiv \sum_n \int [d\mathbf{k}]$ with $[d\mathbf{k}] = d^d\mathbf{k}/(2\pi)^d$, and $\varpi_{ll'}$ is the scattering rate between state $l$ and state $l'$. According to the Fermi golden rule

$$\varpi_{ll'} \equiv \frac{2\pi}{\hbar} |T_{ll'}|^2 \delta(\varepsilon_l - \varepsilon_{l'}), \tag{S4}$$

where $T_{ll'}$ is the scattering matrix. In general, the scattering rate $\varpi_{l'l}$ is not symmetric with respect to the interchange of the initial and final states $\varpi_{ll'} \neq \varpi_{l'l}$. Therefore, $\varpi_{ll'}$ can be formally decomposed into the symmetric and antisymmetric parts as

$$\varpi_{ll'} = \varpi_{ll'}^{sy} + \varpi_{ll'}^{as}, \qquad \varpi_{ll'}^{sy} = \varpi_{l'l}^{sy}, \qquad \varpi_{ll'}^{as} = -\varpi_{l'l}^{as}. \tag{S5}$$

Accordingly, the collision term can also be decomposed as

$$\mathcal{I}_{el}\{f_l\} = \mathcal{I}_{el}^{sy}\{f_l\} + \mathcal{I}_{el}^{sk}\{f_l\}, \tag{S6}$$

where

$$\begin{aligned}
\mathcal{I}_{el}^{sy}\{f_l\} &= -\sum_{l'}(\varpi_{l'l}^{sy} f_l - \varpi_{ll'}^{sy} f_{l'}) \\
&= -\sum_{l'} \varpi_{ll'}^{sy}(f_l - f_{l'}), \\
\mathcal{I}_{el}^{sk}\{f_l\} &= -\sum_{l'}(\varpi_{l'l}^{as} f_l - \varpi_{ll'}^{as} f_{l'}) \\
&= -\sum_{l'} \varpi_{l'l}^{as}(f_l + f_{l'}).
\end{aligned} \tag{S7}$$

The antisymmetric part $\mathcal{I}_{el}^{sk}$ is responsible for the skew-scattering contribution.

If we take into account the work done by the electric field as an electron gets displaced within the unit cell during the collision, the scattering rate is modified as

$$\varpi_{ll'}^{sy} \Rightarrow \tilde{\varpi}_{ll'}^{sy} \equiv \frac{2\pi}{\hbar}|T_{ll'}|^2 \delta(\varepsilon_l - \varepsilon_{l'} + e\mathbf{E}\cdot\delta\mathbf{r}_{ll'}). \tag{S8}$$

Here we only consider the modification to the symmetric part, that is, we have neglected the mixed contribution from the skew-scattering and the coordinate shift, which can be neglected in the weak-disorder limit. The coordinate shift, usually referred to as side-jump, is given for a weak impurity potential $\hat{V}_{imp}$ as

$$\delta\mathbf{r}_{ll'} = \langle u_l | i\partial_{\mathbf{k}} u_l\rangle - \langle u_{l'} | i\partial_{\mathbf{k}'} u_{l'}\rangle - (\partial_{\mathbf{k}} + \partial_{\mathbf{k}'}) \arg\langle u_l | u_{l'}\rangle, \tag{S9}$$

where $\arg(z)$ is the phase of the complex number $z$. The last term in $\delta\mathbf{r}_{ll'}$ is essential contribution which makes the expression for the coordinate shift gauge invariant. Below we take into account contributions up to the first order

$$\begin{aligned}
\delta(\varepsilon_l - \varepsilon_{l'} + e\mathbf{E}\cdot\delta\mathbf{r}_{ll'}) &\simeq \delta(\varepsilon_l - \varepsilon_{l'}) + e\mathbf{E}\cdot\delta\mathbf{r}_{ll'}\frac{\partial}{\partial\varepsilon_l}\delta(\varepsilon_l - \varepsilon_{l'}) \\
&= \delta(\varepsilon_l - \varepsilon_{l'}) - e\mathbf{E}\cdot\delta\mathbf{r}_{ll'}\frac{\partial}{\partial\varepsilon_{l'}}\delta(\varepsilon_l - \varepsilon_{l'}).
\end{aligned} \tag{S10}$$

Thus, the symmetric collision term can be written as

$$\begin{aligned}
\mathcal{I}_{el}^{sy}\{f_l\} &= -\sum_{l'} \tilde{\varpi}_{ll'}^{sy}(f_l - f_{l'}) \\
&= -\sum_{l'} \frac{2\pi}{\hbar}|T_{ll'}|^2 \delta(\varepsilon_l - \varepsilon_{l'} + e\mathbf{E}\cdot\delta\mathbf{r}_{ll'})(f_l - f_{l'}) \\
&\simeq -\sum_{l'} \frac{2\pi}{\hbar}|T_{ll'}|^2 \left[\delta(\varepsilon_l - \varepsilon_{l'}) + e\mathbf{E}\cdot\delta\mathbf{r}_{ll'}\frac{\partial}{\partial\varepsilon_l}\delta(\varepsilon_l - \varepsilon_{l'})\right](f_l - f_{l'}) \\
&= -\sum_{l'}(\varpi_{ll'}^{sy} + e\mathbf{E}\cdot\mathbf{O}_{ll'})(f_l - f_{l'}),
\end{aligned} \tag{S11}$$

where we have defined

$$\mathbf{O}_{ll'} = \frac{2\pi}{\hbar}|T_{ll'}|^2 \delta\mathbf{r}_{ll'}\frac{\partial}{\partial\varepsilon_l}\delta(\varepsilon_l - \varepsilon_{l'}). \tag{S12}$$

One can divide the symmetric collision integral $\mathcal{I}_{el}^{sy}\{f_l\}$ into two parts (intrinsic and side-jump)

$$\mathcal{I}_{el}^{sy}\{f_l\} \equiv \mathcal{I}_{el}^{in}\{f_l\} + \mathcal{I}_{el}^{sj}\{f_l\}, \tag{S13}$$

with

$$\begin{aligned}
\mathcal{I}_{el}^{in}\{f_l\} &= -\sum_{l'} \varpi_{ll'}^{sy}(f_l - f_{l'}), \\
\mathcal{I}_{el}^{sj}\{f_l\} &= -\sum_{l'} e\mathbf{E}\cdot\mathbf{O}_{ll'}(f_l - f_{l'}).
\end{aligned} \tag{S14}$$

Eventually, the collision integral has been approximately decomposed into the intrinsic, side-jump, and skew-scattering parts as

$$\mathcal{I}_{el}\{f_l\} \equiv \mathcal{I}_{el}^{in}\{f_l\} + \mathcal{I}_{el}^{sj}\{f_l\} + \mathcal{I}_{el}^{sk}\{f_l\}, \tag{S15}$$

with

$$\mathcal{I}_{el}^{sk}\{f_l\} = -\sum_{l'} \varpi_{l'l}^{as}(f_l + f_{l'}), \tag{S16}$$

and also the distribution function

$$f_l = f_l^{in} + \delta f_l^{sj} + \delta f_l^{sk}. \tag{S17}$$

The Boltzmann equation now becomes

$$\dot{\mathbf{k}} \cdot \partial_{\mathbf{k}}(f_l^{in} + \delta f_l^{sj} + \delta f_l^{sk}) = \mathcal{I}_{el}^{in}\{f_l\} + \mathcal{I}_{el}^{sj}\{f_l\} + \mathcal{I}_{el}^{sk}\{f_l\}. \tag{S18}$$

Approximately, we can decompose it into three equations as

$$\begin{aligned} \dot{\mathbf{k}} \cdot \partial_{\mathbf{k}} f_l^{in} &= \mathcal{I}_{el}^{in}\{f_l^{in}\}, \\ \dot{\mathbf{k}} \cdot \partial_{\mathbf{k}} \delta f_l^{sj} &= \mathcal{I}_{el}^{in}\{\delta f_l^{sj}\} + \mathcal{I}_{el}^{sj}\{\delta f_l^{in}\}, \\ \dot{\mathbf{k}} \cdot \partial_{\mathbf{k}} \delta f_l^{sk} &= \mathcal{I}_{el}^{in}\{\delta f_l^{sk}\} + \mathcal{I}_{el}^{sk}\{\delta f_l^{in}\}, \end{aligned} \tag{S19}$$

where we have neglected the terms with mixed side-jump and skew-scattering contributions.

### B. Temperature gradient

We consider temperature gradient $\nabla T$ as the driving force. The Boltzmann equation at the steady state is given by

$$\dot{\mathbf{r}} \cdot \frac{\partial f_l}{\partial \mathbf{r}} = \mathcal{I}_{el}\{f_l\}. \tag{S20}$$

The collision term can be formally written as

$$\mathcal{I}_{el}\{f_l\} = -\sum_{l'} (\varpi_{l'l} f_l - \varpi_{ll'} f_{l'}). \tag{S21}$$

Similar to the electric field, the temperature gradient can also modify the scattering rate through the variation of the chemical potential

$$\varpi_{ll'}^{sy} \Rightarrow \tilde{\varpi}_{ll'}^{sy} \equiv \frac{2\pi}{\hbar} |T_{ll'}|^2 \delta\left(\varepsilon_l - \varepsilon_{l'} + \frac{\varepsilon_l - \mu}{T} \nabla T \cdot \delta \mathbf{r}_{ll'}\right). \tag{S22}$$

Here we only consider the modification to the symmetric part, that is, we have neglected the mixed contributions from the skew-scattering and the coordinate shift. Below we take into account contributions up to the first order

$$\delta\left(\varepsilon_l - \varepsilon_{l'} + \frac{\varepsilon_l - \mu}{T} \nabla T \cdot \delta \mathbf{r}_{ll'}\right) \simeq \delta(\varepsilon_l - \varepsilon_{l'}) + \frac{\varepsilon_l - \mu}{T} \nabla T \cdot \delta \mathbf{r}_{ll'} \frac{\partial}{\partial \varepsilon_l} \delta(\varepsilon_l - \varepsilon_{l'}). \tag{S23}$$

Thus, the symmetric collision term can be written as

$$\begin{aligned} \mathcal{I}_{el}^{sy}\{f_l\} &= -\sum_{l'} \tilde{\varpi}_{ll'}^{sy}(f_l - f_{l'}) \\ &= -\sum_{l'} \frac{2\pi}{\hbar} |T_{ll'}|^2 \delta\left(\varepsilon_l - \varepsilon_{l'} + \frac{\varepsilon_l - \mu}{T} \nabla T \cdot \delta \mathbf{r}_{ll'}\right) (f_l - f_{l'}) \\ &\simeq -\sum_{l'} \frac{2\pi}{\hbar} |T_{ll'}|^2 \left[\delta(\varepsilon_l - \varepsilon_{l'}) + \frac{\varepsilon_l - \mu}{T} \nabla T \cdot \delta \mathbf{r}_{ll'} \frac{\partial}{\partial \varepsilon_l} \delta(\varepsilon_l - \varepsilon_{l'})\right] (f_l - f_{l'}) \\ &= -\sum_{l'} \left(\varpi_{ll'}^{sy} + \frac{\varepsilon_l - \mu}{T} \nabla T \cdot \mathbf{O}_{ll'}\right) (f_l - f_{l'}), \end{aligned} \tag{S24}$$

with

$$\mathbf{O}_{ll'} = \frac{2\pi}{\hbar}|T_{ll'}|^2\delta\mathbf{r}_{ll'}\frac{\partial}{\partial\varepsilon_l}\delta(\varepsilon_l - \varepsilon_{l'}). \tag{S25}$$

Accordingly, the collision term can be decomposed as

$$\mathcal{I}_{el}\{f_l\} = \mathcal{I}_{el}^{sy}\{f_l\} + \mathcal{I}_{el}^{sj}\{f_l\} + \mathcal{I}_{el}^{sk}\{f_l\}, \tag{S26}$$

where

$$\begin{aligned}
\mathcal{I}_{el}^{sy}\{f_l\} &= -\sum_{l'} \varpi_{ll'}^{sy}(f_l - f_{l'}), \\
\mathcal{I}_{el}^{sj}\{f_l\} &= -\sum_{l'} \frac{\varepsilon_l - \mu}{T}\nabla T \cdot \mathbf{O}_{ll'}(f_l - f_{l'}), \\
\mathcal{I}_{el}^{sk}\{f_l\} &= -\sum_{l'} \varpi_{l'l}^{as}(f_l + f_{l'}),
\end{aligned} \tag{S27}$$

and also the distribution function

$$f_l = f_l^{in} + \delta f_l^{sj} + \delta f_l^{sk}. \tag{S28}$$

The Boltzmann equation now becomes

$$\dot{\mathbf{r}} \cdot \partial_{\mathbf{r}}(f_l^{in} + \delta f_l^{sk}) = \mathcal{I}_{el}^{in}\{f_l\} + \mathcal{I}_{el}^{sj}\{f_l\} + \mathcal{I}_{el}^{sk}\{f_l\}. \tag{S29}$$

Approximately, we can decomposed it into three equations as

$$\begin{aligned}
\dot{\mathbf{r}} \cdot \partial_{\mathbf{r}} f_l^{in} &= \mathcal{I}_{el}^{in}\{f_l^{in}\}, \\
\dot{\mathbf{r}} \cdot \partial_{\mathbf{r}} \delta f_l^{sj} &= \mathcal{I}_{el}^{in}\{\delta f_l^{sj}\} + \mathcal{I}_{el}^{sj}\{\delta f_l^{in}\}, \\
\dot{\mathbf{r}} \cdot \partial_{\mathbf{r}} \delta f_l^{sk} &= \mathcal{I}_{el}^{in}\{\delta f_l^{sk}\} + \mathcal{I}_{el}^{sk}\{\delta f_l^{in}\},
\end{aligned} \tag{S30}$$

where we have neglected the terms with mixed side-jump and skew-scattering contributions.

## SII. ANOMALOUS ELECTRIC HALL EFFECT

In the absence of the magnetic field, the semiclassical equations of motion are

$$\begin{aligned}
\dot{\mathbf{r}}_l &= \mathbf{v}_l - \dot{\mathbf{k}} \times \Omega_l + \mathbf{v}_l^{sj}, \\
\dot{\mathbf{k}} &= -\frac{e}{\hbar}\mathbf{E},
\end{aligned} \tag{S31}$$

where $\mathbf{v}_l$ and $\mathbf{v}_l^{sj}$ are the intrinsic and side-jump velocities

$$\mathbf{v}_l = \frac{1}{\hbar}\nabla_{\mathbf{k}}\varepsilon, \qquad \mathbf{v}_l^{sj} = \sum_{l'} \varpi_{ll'}^{sy}\delta\mathbf{r}_{l'l}. \tag{S32}$$

Substituting $\dot{\mathbf{k}}$ into $\dot{\mathbf{r}}$, we have

$$\dot{\mathbf{r}}_l = \mathbf{v}_l + \frac{e}{\hbar}\mathbf{E} \times \Omega_l + \mathbf{v}_l^{sj}, \tag{S33}$$

and the electric current reads

$$\mathbf{J} = -e\sum_l \dot{\mathbf{r}}_l f_l = -e\sum_l \left(\mathbf{v}_l + \frac{e}{\hbar}\mathbf{E} \times \Omega_l + \mathbf{v}_l^{sj}\right) f_l. \tag{S34}$$

With the expression of $\dot{\mathbf{k}}$, the decomposed Boltzmann equations become

$$\begin{aligned}
-\frac{e}{\hbar}\mathbf{E} \cdot \partial_{\mathbf{k}} f_l^{in} &= \mathcal{I}_{el}^{in}\{f_l^{in}\}, \\
-\frac{e}{\hbar}\mathbf{E} \cdot \partial_{\mathbf{k}} \delta f_l^{sj} &= \mathcal{I}_{el}^{in}\{\delta f_l^{sj}\} + \mathcal{I}_{el}^{sj}\{f_l^{in}\}, \\
-\frac{e}{\hbar}\mathbf{E} \cdot \partial_{\mathbf{k}} \delta f_l^{sk} &= \mathcal{I}_{el}^{in}\{\delta f_l^{sk}\} + \mathcal{I}_{el}^{sk}\{f_l^{in}\}.
\end{aligned} \tag{S35}$$

### A. Intrinsic contribution

The first line in Eq. (S35) only contains the symmetric scattering, thus we can adopt relaxation time approximation

$$\mathcal{I}_{el}^{in}\{f_l^{in}\} = -\frac{f_l^{in} - f_l^0}{\tau_l}, \tag{S36}$$

where $f_l^0$ is the Fermi-Dirac distribution function, and $\tau_l$ is the general relaxation time. Hence, we can obtain

$$\begin{aligned} &-\frac{e}{\hbar}\mathbf{E}\cdot\partial_{\mathbf{k}} f_l^{in} = -\frac{f_l^{in} - f_l^0}{\tau_l} \\ \Rightarrow\quad &\left(1 - \frac{e\tau_l}{\hbar}\mathbf{E}\cdot\partial_{\mathbf{k}}\right) f_l^{in} = f_l^0, \\ \Rightarrow\quad & f_l^{in} = \frac{1}{1-(e\tau_l/\hbar)\mathbf{E}\cdot\partial_{\mathbf{k}}} f_l^0. \end{aligned} \tag{S37}$$

We can expand $f_l^{in}$ in a series

$$\begin{aligned} f_l^{in} &= \frac{1}{1-(e\tau_l/\hbar)\mathbf{E}\cdot\partial_{\mathbf{k}}} f_l^0 \\ &= \sum_{n=0}\left(\frac{e\tau_l}{\hbar}\mathbf{E}\cdot\partial_{\mathbf{k}}\right)^n f_l^0 \\ &\equiv f_l^0 + \delta^1 f_l^{in} + \delta^2 f_l^{in}\cdots, \end{aligned} \tag{S38}$$

where $\delta^1 f_l^{in}$ is the linear-$\mathbf{E}$ part,

$$\delta^1 f_l^{in} = \frac{e\tau_l}{\hbar}\mathbf{E}\cdot\partial_{\mathbf{k}} f_l^0, \tag{S39}$$

and $\delta^2 f_l^{in}$ is the second-order part

$$\delta^2 f_l^{in} = \frac{e^2\tau_l^2}{\hbar^2}(\mathbf{E}\cdot\partial_{\mathbf{k}})(\mathbf{E}\cdot\partial_{\mathbf{k}}) f_l^0. \tag{S40}$$

Up to the second order of the electric field $\mathbf{E}$, the intrinsic distribution function is written as

$$\begin{aligned} f_l^{in} &\simeq f_l^0 + \delta^1 f_l^{in} + \delta^2 f_l^{in} \\ &= f_l^0 + \frac{e\tau_l}{\hbar}\mathbf{E}\cdot\partial_{\mathbf{k}} f_l^0 + \frac{e^2\tau_l^2}{\hbar^2}(\mathbf{E}\cdot\partial_{\mathbf{k}})(\mathbf{E}\cdot\partial_{\mathbf{k}}) f_l^0 \\ &= f_l^0 + \frac{e\tau_l}{\hbar}\mathcal{E}^d\partial_{\mathbf{k}}^d f_l^0 + \frac{e^2\tau_l^2}{\hbar^2}\mathcal{E}^d\mathcal{E}^e\partial_{\mathbf{k}}^d\partial_{\mathbf{k}}^e f_l^0, \end{aligned} \tag{S41}$$

and the corresponding electric current can be obtained as

$$\begin{aligned} J_a^{in} &= -e\sum_l \left(v_l^a + \frac{e}{\hbar}\epsilon^{abc}\mathcal{E}^b\Omega_l^c\right) f_l^{in} \\ &= -e\sum_l \left(v_l^a + \frac{e}{\hbar}\epsilon^{abc}\mathcal{E}^b\Omega_l^c\right)\left(f_l^0 + \frac{e\tau_l}{\hbar}\mathcal{E}^d\partial_{\mathbf{k}}^d f_l^0 + \frac{e^2\tau_l^2}{\hbar^2}\mathcal{E}^d\mathcal{E}^e\partial_{\mathbf{k}}^d\partial_{\mathbf{k}}^e f_l^0\right). \end{aligned} \tag{S42}$$

After dropping the trivial terms and the terms that contain higher powers of $\mathcal{E}$, we have the result

$$J_a^{in} = -\frac{e^2}{\hbar}\mathcal{E}^b\sum_l \epsilon^{abc}\Omega_l^c f_l^0 - \frac{e^3}{\hbar^2}\mathcal{E}^b\mathcal{E}^d\sum_l \tau_l\epsilon^{abc}\Omega_l^c\partial_{\mathbf{k}}^d f_l^0, \tag{S43}$$

and the intrinsic anomalous Hall current is

$$J_a^{in}[\mathcal{E}] = -\frac{e^2}{\hbar}\mathcal{E}^b\sum_l \epsilon^{abc}\Omega_l^c f_l^0. \tag{S44}$$

### B. Side-jump contribution

The side-jump part of the Boltzmann equation is

$$-\frac{e}{\hbar}\mathbf{E}\cdot\partial_{\mathbf{k}}\delta f_l^{sj}=\mathcal{I}_{el}^{in}\{\delta f_l^{sj}\}+\mathcal{I}_{el}^{sj}\{\delta f_l^{in}\}. \tag{S45}$$

For the symmetric scattering, we still adopt the relaxation time approximation. Thus, the collision integrals are given by

$$\begin{aligned}\mathcal{I}_{el}^{in}\{\delta f_l^{sj}\}&=-\frac{\delta f_l^{sj}}{\tau_l},\\ \mathcal{I}_{el}^{sj}\{f_l^{in}\}&=-\sum_{l'}e\mathbf{E}\cdot\mathbf{O}_{ll'}(f_l^{in}-f_{l'}^{in}),\end{aligned} \tag{S46}$$

now, we have

$$\begin{aligned}-\frac{e}{\hbar}\mathbf{E}\cdot\partial_{\mathbf{k}}\delta f_l^{sj}&=-\frac{\delta f_l^{sj}}{\tau_l}-\sum_{l'}e\mathbf{E}\cdot\mathbf{O}_{ll'}(f_l^{in}-f_{l'}^{in})\\ \Rightarrow\quad\left(1-\frac{e\tau_l}{\hbar}\mathbf{E}\cdot\partial_{\mathbf{k}}\right)\delta f_l^{sj}&=-\sum_{l'}e\tau_l\mathbf{E}\cdot\mathbf{O}_{ll'}(f_l^{in}-f_{l'}^{in}),\\ \Rightarrow\quad\delta f_l^{sj}&=\frac{-1}{1-(e\tau_l/\hbar)\mathbf{E}\cdot\partial_{\mathbf{k}}}\sum_{l'}e\tau_l\mathbf{E}\cdot\mathbf{O}_{ll'}(f_l^{in}-f_{l'}^{in}).\end{aligned} \tag{S47}$$

Similarly, we we can expand $\delta f_l^{sj}$ in a series

$$\begin{aligned}\delta f_l^{sj}&=\frac{-1}{1-(e\tau_l/\hbar)\mathbf{E}\cdot\partial_{\mathbf{k}}}\sum_{l'}e\tau_l\mathbf{E}\cdot\mathbf{O}_{ll'}(f_l^{in}-f_{l'}^{in})\\ &=-\sum_{n=0}\left(\frac{e\tau_l}{\hbar}\mathbf{E}\cdot\partial_{\mathbf{k}}\right)^n\sum_{l'}e\tau_l\mathbf{E}\cdot\mathbf{O}_{ll'}(f_l^{in}-f_{l'}^{in})\\ &=-\sum_{n=0}\left(\frac{e\tau_l}{\hbar}\mathbf{E}\cdot\partial_{\mathbf{k}}\right)^n\sum_{l'}e\tau_l\mathbf{E}\cdot\mathbf{O}_{ll'}\left(f_l^0-f_{l'}^0+\frac{e\tau_l}{\hbar}\mathbf{E}\cdot\partial_{\mathbf{k}}f_l^0-\frac{e\tau_{l'}}{\hbar}\mathbf{E}\cdot\partial_{\mathbf{k}'}f_{l'}^0\right)\\ &\equiv\delta^1 f_l^{sj}+\delta^2 f_l^{sj}+\cdots,\end{aligned} \tag{S48}$$

here we dropped the $\mathcal{E}^2$ term in $f_l^{in}$. The linear-$\mathbf{E}$ part reads

$$\begin{aligned}\delta^1 f_l^{sj}&=-e\tau_l\mathbf{E}\cdot\sum_{l'}\mathbf{O}_{ll'}\left(f_l^0-f_{l'}^0\right)\\ &\equiv-e\tau_l\mathcal{E}^a Q_l^a,\end{aligned} \tag{S49}$$

with

$$Q_l^a=\sum_{l'}O_{ll'}^a\left(f_l^0-f_{l'}^0\right), \tag{S50}$$

and the second-order part is

$$\begin{aligned}\delta^2 f_l^{sj}&=-\frac{e^2\tau_l^2}{\hbar}(\mathbf{E}\cdot\partial_{\mathbf{k}})\mathbf{E}\cdot\sum_{l'}\mathbf{O}_{ll'}\left(f_l^0-f_{l'}^0\right)\\ &\equiv-\frac{e^2\tau_l^2}{\hbar}\mathcal{E}^a\mathcal{E}^b\partial_{\mathbf{k}}^a Q_l^b.\end{aligned} \tag{S51}$$

The side-jump contribution to the distribution function is written as

$$\delta f_l^{sj}\simeq\delta^1 f_l^{sj}+\delta^2 f_l^{sj}. \tag{S52}$$

There are two contributions to the side-jump contribution. The first comes from the side-jump velocity, which can be obtained as

$$\begin{aligned}
J_a^{sj,1} &= -e\sum_l v_a^{sj}(\delta^1 f_l^{in} + \delta^2 f_l^{in}) \\
&= -e\sum_l v_a^{sj}\left(\frac{e\tau_l}{\hbar}\mathcal{E}^b\partial_{\mathbf{k}}^b f_l^0 + \frac{e^2\tau_l^2}{\hbar^2}\mathcal{E}^b\mathcal{E}^c\partial_{\mathbf{k}}^b\partial_{\mathbf{k}}^c f_l^0\right) \\
&= -\frac{e^2}{\hbar}\mathcal{E}^b\sum_l \tau_l v_a^{sj}\partial_{\mathbf{k}}^b f_l^0 - \frac{e^3}{\hbar^2}\mathcal{E}^b\mathcal{E}^c\sum_l \tau_l^2 v_a^{sj}\partial_{\mathbf{k}}^b\partial_{\mathbf{k}}^c f_l^0.
\end{aligned} \tag{S53}$$

The second contribution comes from the side-jump-induced modification to the distribution function, which can be obtained as

$$\begin{aligned}
J_a^{sj,2} &= -e\sum_l \left(v_l^a + \frac{e}{\hbar}\epsilon^{abc}\mathcal{E}^b\Omega_l^c\right)\delta f_l^{sj} \\
&= -e\sum_l \left(v_l^a + \frac{e}{\hbar}\epsilon^{abc}\mathcal{E}^b\Omega_l^c\right)\left(-e\tau_l\mathcal{E}^d Q_l^d - \frac{e^2\tau_l^2}{\hbar}\mathcal{E}^d\mathcal{E}^e\partial_{\mathbf{k}}^d Q_l^e\right) \\
&= e^2\mathcal{E}^d\sum_l \tau_l v_l^a Q_l^d + \frac{e^3}{\hbar}\mathcal{E}^d\mathcal{E}^e\sum_l \tau_l^2 v_l^a\partial_{\mathbf{k}}^d Q_l^e + \frac{e^3}{\hbar}\mathcal{E}^b\mathcal{E}^d\sum_l \tau_l\epsilon^{abc}\Omega_l^c Q_l^d,
\end{aligned} \tag{S54}$$

here we dropped the higher-power terms of $\mathcal{E}$.

The side-jump contribution to the anomalous Hall current is

$$\begin{aligned}
J_a^{sj,1}[\mathcal{E}] &= -\frac{e^2}{\hbar}\mathcal{E}^b\sum_l \tau_l v_a^{sj}\partial_{\mathbf{k}}^b f_l^0, \\
J_a^{sj,2}[\mathcal{E}] &= e^2\mathcal{E}^b\sum_l \tau_l v_l^a Q_l^b.
\end{aligned} \tag{S55}$$

### C. Skew-scattering contribution

The skew-scattering part of the Boltzmann equation is

$$-\frac{e}{\hbar}\mathbf{E}\cdot\partial_{\mathbf{k}}\delta f_l^{sk} = \mathcal{I}_{el}^{in}\{\delta f_l^{sk}\} + \mathcal{I}_{el}^{sk}\{f_l^{in}\}, \tag{S56}$$

the collision integrals are given by

$$\begin{aligned}
\mathcal{I}_{el}^{in}\{\delta f_l^{sk}\} &= -\frac{\delta f_l^{sk}}{\tau_l}, \\
\mathcal{I}_{el}^{sk}\{f_l^{in}\} &= -\sum_{l'}\varpi_{l'l}^{as}(f_l^{in} + f_{l'}^{in}).
\end{aligned} \tag{S57}$$

Thus, the Boltzmann equation becomes

$$\begin{aligned}
&-\frac{e}{\hbar}\mathbf{E}\cdot\partial_{\mathbf{k}}\delta f_l^{sk} = -\frac{\delta f_l^{sk}}{\tau_l} - \sum_{l'}\varpi_{l'l}^{as}(f_l^{in} + f_{l'}^{in}) \\
\Rightarrow\quad &\left(1 - \frac{e\tau_l}{\hbar}\mathbf{E}\cdot\partial_{\mathbf{k}}\right)\delta f_l^{sk} = -\sum_{l'}\tau_l\varpi_{l'l}^{as}(f_l^{in} + f_{l'}^{in}), \\
\Rightarrow\quad &\delta f_l^{sk} = \frac{-1}{1 - (e\tau_l/\hbar)\mathbf{E}\cdot\partial_{\mathbf{k}}}\sum_{l'}\tau_l\varpi_{l'l}^{as}(f_l^{in} + f_{l'}^{in}).
\end{aligned} \tag{S58}$$

Expand $\delta f_l^{sk}$ in a series

$$\begin{aligned}
\delta f_l^{sk} &= \frac{-1}{1-(e\tau_l/\hbar)\mathbf{E}\cdot\partial_{\mathbf{k}}}\sum_{l'}\tau_l\varpi_{l'l}^{as}(f_l^{in}+f_{l'}^{in}) \\
&= -\sum_{n=0}\left(\frac{e\tau_l}{\hbar}\mathbf{E}\cdot\partial_{\mathbf{k}}\right)^n\sum_{l'}\tau_l\varpi_{l'l}^{as}(f_l^{in}+f_{l'}^{in}) \\
&= -\sum_{n=0}\left(\frac{e\tau_l}{\hbar}\mathbf{E}\cdot\partial_{\mathbf{k}}\right)^n\sum_{l'}\tau_l\varpi_{l'l}^{as}\Big[f_l^0+f_{l'}^0+\frac{e\tau_l}{\hbar}\mathbf{E}\cdot\partial_{\mathbf{k}}f_l^0+\frac{e\tau_{l'}}{\hbar}\mathbf{E}\cdot\partial_{\mathbf{k}'}f_{l'}^0 \\
&\quad+\frac{e^2\tau_l^2}{\hbar^2}(\mathbf{E}\cdot\partial_{\mathbf{k}})(\mathbf{E}\cdot\partial_{\mathbf{k}})f_l^0+\frac{e^2\tau_{l'}^2}{\hbar^2}(\mathbf{E}\cdot\partial_{\mathbf{k}'})(\mathbf{E}\cdot\partial_{\mathbf{k}'})f_{l'}^0\Big] \\
&\equiv \delta^1 f_l^{sk}+\delta^2 f_l^{sk}+\cdots .
\end{aligned} \tag{S59}$$

Note that the equilibrium distribution function does not contribute to the scattering

$$\sum_{l'}\varpi_{l'l}^{as}\left(f_l^0+f_{l'}^0\right)=0. \tag{S60}$$

The linear-$\mathbf{E}$ part reads

$$\begin{aligned}
\delta^1 f_l^{sk} &= -\frac{e}{\hbar}\mathbf{E}\cdot\sum_{l'}\tau_l^2\varpi_{l'l}^{as}\partial_{\mathbf{k}}f_l^0-\frac{e}{\hbar}\mathbf{E}\cdot\sum_{l'}\tau_l\tau_{l'}\varpi_{l'l}^{as}\partial_{\mathbf{k}'}f_{l'}^0 \\
&= -\frac{e}{\hbar}\mathcal{E}^a\sum_{l'}\tau_l^2\varpi_{l'l}^{as}\partial_{\mathbf{k}}^a f_l^0-\frac{e}{\hbar}\mathcal{E}^a\sum_{l'}\tau_l\tau_{l'}\varpi_{l'l}^{as}\partial_{\mathbf{k}'}^a f_{l'}^0,
\end{aligned} \tag{S61}$$

and the second-order part is

$$\begin{aligned}
\delta^2 f_l^{sk} =& -\frac{e^2}{\hbar^2}\sum_{l'}\tau_l^3\varpi_{l'l}^{as}(\mathbf{E}\cdot\partial_{\mathbf{k}})(\mathbf{E}\cdot\partial_{\mathbf{k}})f_l^0-\frac{e^2}{\hbar^2}\sum_{l'}\tau_l\tau_{l'}^2\varpi_{l'l}^{as}(\mathbf{E}\cdot\partial_{\mathbf{k}'})(\mathbf{E}\cdot\partial_{\mathbf{k}'})f_{l'}^0 \\
&-\frac{e^2}{\hbar^2}\sum_{l'}\tau_l^3\varpi_{l'l}^{as}(\mathbf{E}\cdot\partial_{\mathbf{k}})(\mathbf{E}\cdot\partial_{\mathbf{k}})f_l^0-\frac{e^2}{\hbar^2}\sum_{l'}\tau_l^2\tau_{l'}\varpi_{l'l}^{as}(\mathbf{E}\cdot\partial_{\mathbf{k}})(\mathbf{E}\cdot\partial_{\mathbf{k}'})f_{l'}^0 \\
=& -\frac{2e^2}{\hbar^2}\mathcal{E}^a\mathcal{E}^b\sum_{l'}\tau_l^3\varpi_{l'l}^{as}\partial_{\mathbf{k}}^a\partial_{\mathbf{k}}^b f_l^0-\frac{e^2}{\hbar^2}\mathcal{E}^a\mathcal{E}^b\sum_{l'}\tau_l\tau_{l'}^2\varpi_{l'l}^{as}\partial_{\mathbf{k}'}^a\partial_{\mathbf{k}'}^b f_{l'}^0-\frac{e^2}{\hbar^2}\mathcal{E}^a\mathcal{E}^b\sum_{l'}\tau_l^2\tau_{l'}\varpi_{l'l}^{as}\partial_{\mathbf{k}}^a\partial_{\mathbf{k}'}^b f_{l'}^0.
\end{aligned} \tag{S62}$$

The skew-scattering contribution to the distribution function is written as

$$\delta f_l^{sk}\simeq\delta^1 f_l^{sk}+\delta^2 f_l^{sk}, \tag{S63}$$

then the corresponding electric current contribution can be written as

$$\begin{aligned}
J_a^{sk} =& -e\sum_l\left(v_l^a+\frac{e}{\hbar}\epsilon^{abc}\mathcal{E}^b\Omega_l^c\right)\delta f_l^{sk} \\
=& -e\sum_l\left(v_l^a+\frac{e}{\hbar}\epsilon^{ade}\mathcal{E}^d\Omega_l^e\right)\left[-\frac{e}{\hbar}\mathcal{E}^b\sum_{l'}\tau_l^2\varpi_{l'l}^{as}\partial_{\mathbf{k}}^b f_l^0-\frac{e}{\hbar}\mathcal{E}^b\sum_{l'}\tau_l\tau_{l'}\varpi_{l'l}^{as}\partial_{\mathbf{k}'}^b f_{l'}^0\right]. \\
=&\frac{e^2}{\hbar}\mathcal{E}^b\sum_{ll'}v_l^a\tau_l^2\varpi_{l'l}^{as}\partial_{\mathbf{k}}^b f_l^0+\frac{e^2}{\hbar}\mathcal{E}^b\sum_{ll'}v_l^a\tau_l\tau_{l'}\varpi_{l'l}^{as}\partial_{\mathbf{k}'}^b f_{l'}^0,
\end{aligned} \tag{S64}$$

here we have dropped higher powers of $\mathcal{E}$.

The skew-scattering contribution to the anomalous Hall current is

$$J_a^{sk}[\mathcal{E}]=\frac{e^2}{\hbar}\mathcal{E}^b\sum_{ll'}v_l^a\tau_l^2\varpi_{l'l}^{as}\partial_{\mathbf{k}}^b f_l^0+\frac{e^2}{\hbar}\mathcal{E}^b\sum_{ll'}v_l^a\tau_l\tau_{l'}\varpi_{l'l}^{as}\partial_{\mathbf{k}'}^b f_{l'}^0. \tag{S65}$$

### D. Anomalous electric Hall conductivity

The anomalous Hall conductivity can be obtained by writing that

$$J_a = \sigma_{ab}^{tot}\mathcal{E}_b. \tag{S66}$$

We obtain that

$$\sigma_{ab}^{tot} = \sigma_{ab}^{in} + \sigma_{ab}^{sj,1} + \sigma_{ab}^{sj,2} + \sigma_{ab}^{sk}, \tag{S67}$$

with

$$\begin{aligned}
\sigma_{ab}^{in} &= -\frac{e^2}{\hbar}\sum_l \epsilon^{abc}\Omega_l^c f_l^0, \\
\sigma_{ab}^{sj,1} &= -\frac{e^2}{\hbar}\sum_l \tau_l v_a^{sj}\partial_{\mathbf{k}}^b f_l^0, \\
\sigma_{ab}^{sj,2} &= e^2\sum_{ll'}\tau_l v_l^a O_{ll'}^b\left(f_l^0 - f_{l'}^0\right), \\
\sigma_{ab}^{sk} &= \frac{e^2}{\hbar}\sum_{ll'} v_l^a\tau_l^2\varpi_{l'l}^{as}\partial_{\mathbf{k}}^b f_l^0 + \frac{e^2}{\hbar}\sum_{ll'} v_l^a\tau_l\tau_{l'}\varpi_{l'l}^{as}\partial_{\mathbf{k}'}^b f_{l'}^0.
\end{aligned} \tag{S68}$$

In the isotropic limit, the general relaxation time $\tau_l$ can be considered as a constant $\tau$. Thus, the general expressions can be further simplified,

$$\begin{aligned}
\sigma_{ab}^{sj,2} &= e^2\sum_{ll'}\tau_l v_l^a O_{ll'}^b\left(f_l^0 - f_{l'}^0\right) \\
&= e^2\tau\sum_{ll'} v_l^a\left[\frac{2\pi}{\hbar}|T_{ll'}|^2\delta r_{ll'}^b\frac{\partial}{\partial\varepsilon_l}\delta(\varepsilon_l-\varepsilon_{l'})\right]\left(f_l^0 - f_{l'}^0\right) \\
&= \frac{e^2}{\hbar}\tau\sum_{ll'}\frac{2\pi}{\hbar}|T_{ll'}|^2\delta r_{ll'}^b\left[\partial_{\mathbf{k}}^a\delta(\varepsilon_l-\varepsilon_{l'})\right]\left(f_l^0 - f_{l'}^0\right) \\
&= \frac{e^2}{\hbar}\tau\sum_{ll'}\frac{2\pi}{\hbar}|T_{ll'}|^2\delta r_{ll'}^b\left\{\partial_{\mathbf{k}}^a\left[\delta(\varepsilon_l-\varepsilon_{l'})\left(f_l^0 - f_{l'}^0\right)\right] - \delta(\varepsilon_l-\varepsilon_{l'})\left[\partial_{\mathbf{k}}^a\left(f_l^0 - f_{l'}^0\right)\right]\right\} \\
&= -\frac{e^2}{\hbar}\tau\sum_{ll'}\frac{2\pi}{\hbar}|T_{ll'}|^2\delta r_{ll'}^b\delta(\varepsilon_l-\varepsilon_{l'})\partial_{\mathbf{k}}^a f_l^0 \\
&\simeq -\frac{e^2}{\hbar}\tau\sum_{ll'}\varpi_{ll'}^{sy}(-\delta r_{l'l}^b)\partial_{\mathbf{k}}^a f_l^0 \\
&= \frac{e^2}{\hbar}\tau\sum_l v_b^{sj}\partial_{\mathbf{k}}^a f_l^0,
\end{aligned} \tag{S69}$$

where we have dropped the antisymmetric part in $\varpi_{ll'}$ and

$$\begin{aligned}
\sigma_{ab}^{sk} &= \frac{e^2}{\hbar}\sum_{ll'} v_l^a\tau_l^2\varpi_{l'l}^{as}\partial_{\mathbf{k}}^b f_l^0 + \frac{e^2}{\hbar}\sum_{ll'} v_l^a\tau_l\tau_{l'}\varpi_{l'l}^{as}\partial_{\mathbf{k}'}^b f_{l'}^0 \\
&= -\frac{e^2}{\hbar}\tau^2\sum_{ll'} v_l^a\varpi_{ll'}^{as}\partial_{\mathbf{k}}^b f_l^0 + \frac{e^2}{\hbar}\tau^2\sum_{ll'} v_{l'}^a\varpi_{ll'}^{as}\partial_{\mathbf{k}}^b f_l^0 \\
&= -\frac{e^2}{\hbar}\tau^2\sum_{ll'}\varpi_{ll'}^{as}(v_l^a - v_{l'}^a)\partial_{\mathbf{k}}^b f_l^0.
\end{aligned} \tag{S70}$$

Thus, we obtain

$$\begin{aligned}
\sigma_{ab}^{in} &= -\frac{e^2}{\hbar}\sum_l \epsilon^{abc}\Omega_l^c f_l^0, \\
\sigma_{ab}^{sj,1} &= -\frac{e^2}{\hbar}\tau\sum_l v_a^{sj}\partial_{\mathbf{k}}^b f_l^0, \\
\sigma_{ab}^{sj,2} &= \frac{e^2}{\hbar}\tau\sum_l v_b^{sj}\partial_{\mathbf{k}}^a f_l^0, \\
\sigma_{ab}^{sk} &= -\frac{e^2}{\hbar}\tau^2\sum_{ll'} \varpi_{ll'}^{as}(v_l^a - v_{l'}^a)\partial_{\mathbf{k}}^b f_l^0.
\end{aligned} \tag{S71}$$

## SIII. ANOMALOUS THERMOELECTRIC HALL EFFECT

In the absence of the electric field and the magnetic field, the semiclassical equation of motion is

$$\dot{\mathbf{r}}_l = \mathbf{v}_l + \mathbf{v}_l^{sj}, \tag{S72}$$

where $\mathbf{v}_l$ and $\mathbf{v}_l^{sj}$ are the intrinsic and side-jump velocities

$$\mathbf{v}_l = \frac{1}{\hbar}\nabla_{\mathbf{k}}\varepsilon, \qquad \mathbf{v}_l^{sj} = \sum_{l'}\varpi_{ll'}^{sy}\delta\mathbf{r}_{l'l}. \tag{S73}$$

Thus, the electric current reads

$$\mathbf{J} = -e\sum_l \dot{\mathbf{r}}_l f_l = -e\sum_l(\mathbf{v}_l + \mathbf{v}_l^{sj})f_l. \tag{S74}$$

The decomposed Boltzmann equations become

$$\begin{aligned}
\mathbf{v}_l\cdot\partial_{\mathbf{r}} f_l^{in} &= \mathcal{I}_{el}^{in}\{f_l^{in}\}, \\
\mathbf{v}_l\cdot\partial_{\mathbf{r}}\delta f_l^{sj} &= \mathcal{I}_{el}^{in}\{\delta f_l^{sj}\} + \mathcal{I}_{el}^{sj}\{f_l^{in}\}. \\
\mathbf{v}_l\cdot\partial_{\mathbf{r}}\delta f_l^{sk} &= \mathcal{I}_{el}^{in}\{\delta f_l^{sk}\} + \mathcal{I}_{el}^{sk}\{f_l^{in}\}.
\end{aligned} \tag{S75}$$

### A. Intrinsic contribution

For the intrinsic contribution, we can adopt the relaxation time approximation

$$\mathcal{I}_{el}^{in}\{f_l^{in}\} = -\frac{f_l^{in} - f_l^0}{\tau_l}, \tag{S76}$$

where $f_l^0$ is the Fermi-Dirac distribution function, and $\tau_l$ is the general relaxation time. Hence, we can obtain

$$\begin{aligned}
&\mathbf{v}_l\cdot\partial_{\mathbf{r}} f_l^{in} = -\frac{f_l^{in} - f_l^0}{\tau_l} \\
\Rightarrow\quad &(1 + \tau_l\mathbf{v}_l\cdot\partial_{\mathbf{r}})\, f_l^{in} = f_l^0, \\
\Rightarrow\quad &f_l^{in} = \frac{1}{1 + \tau_l\mathbf{v}_l\cdot\partial_{\mathbf{r}}} f_l^0.
\end{aligned} \tag{S77}$$

We can expand $f_l^{in}$ in a series

$$\begin{aligned}
f_l^{in} &= \frac{1}{1 + \tau_l\mathbf{v}_l\cdot\partial_{\mathbf{r}}} f_l^0 \\
&= \sum_{n=0}(-\tau_l\mathbf{v}_l\cdot\partial_{\mathbf{r}})^n f_l^0 \\
&\equiv f_l^0 + \delta^1 f_l^{in} + \cdots,
\end{aligned} \tag{S78}$$

where $\delta^1 f_l^{in}$ refers to the linear-$\mathbf{E}$ part,

$$\delta^1 f_l^{in} = -\tau_l \mathbf{v}_l \cdot \partial_{\mathbf{r}} f_l^0. \tag{S79}$$

Up to the first order of the temperature gradient $\nabla T$, the intrinsic distribution function is written as

$$\begin{aligned} f_l^{in} &\simeq f_l^0 + \delta^1 f_l^{in} \\ &= f_l^0 - \tau_l \mathbf{v}_l \cdot \partial_{\mathbf{r}} f_l^0 \\ &= f_l^0 + \tau_l \mathbf{v}_l \cdot \frac{\varepsilon_l - \mu}{T} \frac{\partial f_l^0}{\partial \varepsilon_l} \nabla T, \\ &= f_l^0 + \frac{\tau_l}{\hbar} \frac{\varepsilon_l - \mu}{T} \partial_{\mathbf{k}} f_l^0 \cdot \nabla T, \end{aligned} \tag{S80}$$

the corresponding electric current can be obtained as

$$\begin{aligned} J_a^{in} &= -e \sum_l v_l^a f_l^{in} \\ &= -e \sum_l v_l^a \left( f_l^0 + \frac{\tau_l}{\hbar} \frac{\varepsilon_l - \mu}{T} \partial_{\mathbf{k}}^b f_l^0 \partial_{\mathbf{r}}^b T \right). \end{aligned} \tag{S81}$$

Both of them are trivial terms, which do not contribute to the anomalous thermoelectric current. The anomalous thermoelectric current induced by the Berry curvature is given by

$$J_a^{in} = -\frac{e}{\hbar} \partial_{\mathbf{r}}^b T \int d\varepsilon \frac{\varepsilon - \mu}{T} \sum_l \epsilon^{abc} \Omega_l^c f_l^0 \left( -\frac{\partial f^0}{\partial \varepsilon} \right). \tag{S82}$$

### B. Side-jump contribution

The side-jump part of the Boltzmann equation is

$$\mathbf{v}_l \cdot \partial_{\mathbf{r}} \delta f_l^{sj} = \mathcal{I}_{el}^{in}\{\delta f_l^{sj}\} + \mathcal{I}_{el}^{sj}\{\delta f_l^{in}\}. \tag{S83}$$

For the symmetric scattering, we still adopt the relaxation time approximation. Thus, the collision integrals are given by

$$\begin{aligned} \mathcal{I}_{el}^{in}\{\delta f_l^{sj}\} &= -\frac{\delta f_l^{sj}}{\tau_l}, \\ \mathcal{I}_{el}^{sj}\{f_l^{in}\} &= -\sum_{l'} \frac{\varepsilon_l - \mu}{T} \nabla T \cdot \mathbf{O}_{ll'} (f_l^{in} - f_{l'}^{in}), \end{aligned} \tag{S84}$$

now, we have

$$\begin{aligned} \mathbf{v}_l \cdot \partial_{\mathbf{r}} \delta f_l^{sj} &= -\frac{\delta f_l^{sj}}{\tau_l} - \sum_{l'} \frac{\varepsilon_l - \mu}{T} \nabla T \cdot \mathbf{O}_{ll'} (f_l^{in} - f_{l'}^{in}) \\ \Rightarrow \quad (1 + \tau_l \mathbf{v}_l \cdot \partial_{\mathbf{r}}) \delta f_l^{sj} &= -\sum_{l'} \tau_l k_B \nabla T \cdot \mathbf{O}_{ll'} (f_l^{in} - f_{l'}^{in}), \\ \Rightarrow \quad \delta f_l^{sj} &= \frac{-1}{1 + \tau_l \mathbf{v}_l \cdot \partial_{\mathbf{r}}} \sum_{l'} \tau_l \frac{\varepsilon_l - \mu}{T} \nabla T \cdot \mathbf{O}_{ll'} (f_l^{in} - f_{l'}^{in}). \end{aligned} \tag{S85}$$

Similarly, we can expand $\delta f_l^{sj}$ in a series

$$\begin{aligned} \delta f_l^{sj} &= \frac{-1}{1 + \tau_l \mathbf{v}_l \cdot \partial_{\mathbf{r}}} \sum_{l'} \tau_l \frac{\varepsilon_l - \mu}{T} \nabla T \cdot \mathbf{O}_{ll'} (f_l^{in} - f_{l'}^{in}) \\ &= -\sum_{n=0} (-\tau_l \mathbf{v}_l \cdot \partial_{\mathbf{r}})^n \sum_{l'} \tau_l \frac{\varepsilon_l - \mu}{T} \nabla T \cdot \mathbf{O}_{ll'} (f_l^{in} - f_{l'}^{in}) \\ &= -\sum_{n=0} (-\tau_l \mathbf{v}_l \cdot \partial_{\mathbf{r}})^n \sum_{l'} \tau_l \frac{\varepsilon_l - \mu}{T} \nabla T \cdot \mathbf{O}_{ll'} \left( f_l^0 - f_{l'}^0 + \frac{\tau_l}{\hbar} \frac{\varepsilon_l - \mu}{T} \partial_{\mathbf{k}} f_l^0 \cdot \nabla T - \frac{\tau_{l'}}{\hbar} \frac{\varepsilon_{l'} - \mu}{T} \partial_{\mathbf{k}'} f_{l'}^0 \cdot \nabla T \right) \\ &\equiv \delta^1 f_l^{sj} + \cdots . \end{aligned} \tag{S86}$$

The linear-$\nabla T$ part reads

$$\begin{aligned}\delta^1 f_l^{sj} &= -\tau_l \sum_{l'} \frac{\varepsilon_l - \mu}{T} \nabla T \cdot \mathbf{O}_{ll'} \left(f_l^0 - f_{l'}^0\right) \\ &= -\tau_l \partial_{\mathbf{r}}^a T \sum_{l'} \frac{\varepsilon_l - \mu}{T} O_{ll'}^a \left(f_l^0 - f_{l'}^0\right).\end{aligned} \tag{S87}$$

The side-jump contribution to the distribution function is written as

$$\delta f_l^{sj} \simeq \delta^1 f_l^{sj}. \tag{S88}$$

There are two contributions to the side-jump contribution. The first comes from the side-jump velocity, which can be obtained as

$$\begin{aligned}J_a^{sj,1} &= -e \sum_l v_a^{sj} \delta^1 f_l^{in} \\ &= -\frac{e}{\hbar} \partial_{\mathbf{r}}^b T \sum_l v_a^{sj} \tau_l \frac{\varepsilon_l - \mu}{T} \partial_{\mathbf{k}}^b f_l^0.\end{aligned} \tag{S89}$$

The second contribution comes from the side-jump-induced modification to the distribution function, which can be obtained as

$$\begin{aligned}J_a^{sj,2} &= -e \sum_l v_l^a \delta f_l^{sj} \\ &= e \partial_{\mathbf{r}}^b T \sum_{ll'} v_l^a \tau_l \frac{\varepsilon_l - \mu}{T} O_{ll'}^b \left(f_l^0 - f_{l'}^0\right).\end{aligned} \tag{S90}$$

### C. Skew-scattering contribution

The skew-scattering part of the Boltzmann equation is

$$\mathbf{v}_l \cdot \partial_{\mathbf{r}} \delta f_l^{sj} f_l^{sk} = \mathcal{I}_{el}^{in}\{\delta f_l^{sk}\} + \mathcal{I}_{el}^{sk}\{f_l^{in}\}, \tag{S91}$$

the collision integrals are given by

$$\begin{aligned}\mathcal{I}_{el}^{in}\{\delta f_l^{sk}\} &= -\frac{\delta f_l^{sk}}{\tau_l}, \\ \mathcal{I}_{el}^{sk}\{f_l^{in}\} &= -\sum_{l'} \varpi_{l'l}^{as}(f_l^{in} + f_{l'}^{in}).\end{aligned} \tag{S92}$$

Thus, the Boltzmann equation becomes

$$\begin{aligned}\mathbf{v}_l \cdot \partial_{\mathbf{r}} \delta f_l^{sk} &= -\frac{\delta f_l^{sk}}{\tau_l} - \sum_{l'} \varpi_{l'l}^{as}(f_l^{in} + f_{l'}^{in}) \\ \Rightarrow \quad \left(1 + \tau_l \mathbf{v}_l \cdot \partial_{\mathbf{r}}\right) \delta f_l^{sk} &= -\sum_{l'} \tau_l \varpi_{l'l}^{as}(f_l^{in} + f_{l'}^{in}), \\ \Rightarrow \quad \delta f_l^{sk} &= \frac{-1}{1 + \tau_l \mathbf{v}_l \cdot \partial_{\mathbf{r}}} \sum_{l'} \tau_l \varpi_{l'l}^{as}(f_l^{in} + f_{l'}^{in}).\end{aligned} \tag{S93}$$

Expand $\delta f_l^{sk}$ in a series

$$\begin{aligned}\delta f_l^{sk} &= \frac{-1}{1 + \tau_l \mathbf{v}_l \cdot \partial_{\mathbf{r}}} \sum_{l'} \tau_l \varpi_{l'l}^{as}(f_l^{in} + f_{l'}^{in}) \\ &= -\sum_{n=0} \left(-\tau_l \mathbf{v}_l \cdot \partial_{\mathbf{r}}\right)^n \sum_{l'} \tau_l \varpi_{l'l}^{as}(f_l^{in} + f_{l'}^{in}) \\ &= -\sum_{n=0} \left(-\tau_l \mathbf{v}_l \cdot \partial_{\mathbf{r}}\right)^n \sum_{l'} \tau_l \varpi_{l'l}^{as} \left[f_l^0 + f_{l'}^0 + \frac{\tau_l}{\hbar} \frac{\varepsilon_l - \mu}{T} \partial_{\mathbf{k}} f_l^0 \cdot \nabla T + \frac{\tau_{l'}}{\hbar} \frac{\varepsilon_{l'} - \mu}{T} \partial_{\mathbf{k}'} f_{l'}^0 \cdot \nabla T\right] \\ &\equiv \delta^1 f_l^{sk} + \cdots.\end{aligned} \tag{S94}$$

Note that the equilibrium distribution function does not contribute to the scattering

$$\sum_{l'} \varpi_{l'l}^{as} \left(f_l^0 + f_{l'}^0\right) = 0. \tag{S95}$$

The linear-$\nabla T$ part reads

$$\begin{aligned}\delta^1 f_l^{sk} &= \sum_{l'} \frac{\tau_l^2}{\hbar} \varpi_{l'l}^{as} \frac{\varepsilon_l - \mu}{T} \partial_{\mathbf{k}} f_l^0 \cdot \nabla T + \sum_{l'} \frac{\tau_l \tau_{l'}}{\hbar} \varpi_{l'l}^{as} \frac{\varepsilon_{l'} - \mu}{T} \partial_{\mathbf{k}'} f_{l'}^0 \cdot \nabla T \\ &= \partial_{\mathbf{r}}^a T \sum_{l'} \frac{\tau_l^2}{\hbar} \varpi_{l'l}^{as} \frac{\varepsilon_l - \mu}{T} \partial_{\mathbf{k}}^a f_l^0 + \partial_{\mathbf{r}}^a T \sum_{l'} \frac{\tau_l \tau_{l'}}{\hbar} \varpi_{l'l}^{as} \frac{\varepsilon_{l'} - \mu}{T} \partial_{\mathbf{k}'}^a f_{l'}^0.\end{aligned} \tag{S96}$$

The skew-scattering contribution to the distribution function is written as

$$\delta f_l^{sk} \simeq \delta^1 f_l^{sk}, \tag{S97}$$

then the corresponding electric current contribution can be written as

$$\begin{aligned}J_a^{sk} =& - e \sum_l v_l^a \delta f_l^{sk} \\ =& - e \sum_l v_l^a \left[\partial_{\mathbf{r}}^b T \sum_{l'} \frac{\tau_l^2}{\hbar} \varpi_{l'l}^{as} \frac{\varepsilon_l - \mu}{T} \partial_{\mathbf{k}}^b f_l^0 + \partial_{\mathbf{r}}^b T \sum_{l'} \frac{\tau_l \tau_{l'}}{\hbar} \varpi_{l'l}^{as} \frac{\varepsilon_{l'} - \mu}{T} \partial_{\mathbf{k}'}^b f_{l'}^0\right] \\ =& - \frac{e}{\hbar} \partial_{\mathbf{r}}^b T \sum_{ll'} v_l^a \tau_l^2 \varpi_{l'l}^{as} \frac{\varepsilon_l - \mu}{T} \partial_{\mathbf{k}}^b f_l^0 - \frac{e}{\hbar} \partial_{\mathbf{r}}^b T \sum_{l'} \tau_l \tau_{l'} \varpi_{l'l}^{as} \frac{\varepsilon_{l'} - \mu}{T} \partial_{\mathbf{k}'}^b f_{l'}^0.\end{aligned} \tag{S98}$$

### D. Anomalous thermoelectric Hall conductivity

The anomalous electric Hall conductivity can be obtained by writing that

$$J_a = \alpha_{ab}^{tot} (-\partial_{\mathbf{r}}^b T). \tag{S99}$$

We obtain that

$$\alpha_{ab}^{tot} = \alpha_{ab}^{in} + \alpha_{ab}^{sj,1} + \alpha_{ab}^{sj,2} + \alpha_{ab}^{sk}, \tag{S100}$$

with

$$\begin{aligned}\alpha_{ab}^{in} &= \frac{k_B e}{\hbar} \int d\varepsilon \frac{\varepsilon - \mu}{k_B T} \sum_l \epsilon^{abc} \Omega_l^c f_l^0 \left(-\frac{\partial f^0}{\partial \varepsilon}\right), \\ \alpha_{ab}^{sj,1} &= \frac{k_B e}{\hbar} \sum_l v_a^{sj} \tau_l \frac{\varepsilon_l - \mu}{k_B T} \partial_{\mathbf{k}}^b f_l^0, \\ \alpha_{ab}^{sj,2} &= -k_B e \sum_{ll'} v_l^a \tau_l \frac{\varepsilon_l - \mu}{k_B T} O_{ll'}^b \left(f_l^0 - f_{l'}^0\right), \\ \alpha_{ab}^{sk} &= -\frac{k_B e}{\hbar} \sum_{ll'} v_l^a \tau_l^2 \varpi_{l'l}^{as} \frac{\varepsilon_l - \mu}{k_B T} \partial_{\mathbf{k}}^b f_l^0 - \frac{k_B e}{\hbar} \sum_{ll'} v_l^a \tau_l \tau_{l'} \varpi_{l'l}^{as} \frac{\varepsilon_l - \mu}{k_B T} \partial_{\mathbf{k}'}^b f_{l'}^0.\end{aligned} \tag{S101}$$

In the isotropic limit, the general relaxation time $\tau_l$ can be considered as a constant $\tau$. Thus, the general expressions can be further simplified

$$\begin{aligned}\alpha_{ab}^{sj,2} &= -k_B e \sum_{ll'} \frac{\varepsilon_l - \mu}{k_B T} \tau_l v_l^a O_{ll'}^b \left(f_l^0 - f_{l'}^0\right) \\ &= -k_B e \tau \sum_{ll'} \frac{\varepsilon_l - \mu}{k_B T} v_l^a \left[\frac{2\pi}{\hbar} |T_{ll'}|^2 \delta r_{ll'}^b \frac{\partial}{\partial \varepsilon_l} \delta(\varepsilon_l - \varepsilon_{l'})\right] \left(f_l^0 - f_{l'}^0\right) \\ &\simeq \frac{k_B e}{\hbar} \tau \sum_{ll'} \frac{\varepsilon_l - \mu}{k_B T} \varpi_{ll'}^{sy} (-\delta r_{l'l}^b) \partial_{\mathbf{k}}^a f_l^0 \\ &= -\frac{k_B e}{\hbar} \tau \sum_l \frac{\varepsilon_l - \mu}{k_B T} v_b^{sj} \partial_{\mathbf{k}}^a f_l^0,\end{aligned} \tag{S102}$$

and for the skew-scattering term

$$\begin{aligned}\alpha_{ab}^{sk} &= -\frac{k_B e}{\hbar}\sum_{ll'} v_l^a \tau_l^2 \varpi_{l'l}^{as}\frac{\varepsilon_l-\mu}{k_B T}\partial_{\mathbf{k}}^b f_l^0 - \frac{k_B e}{\hbar}\sum_{ll'} v_l^a \tau_l \tau_{l'} \varpi_{l'l}^{as}\frac{\varepsilon_l-\mu}{k_B T}\partial_{\mathbf{k}'}^b f_{l'}^0 \\ &= \frac{k_B e}{\hbar}\tau^2\sum_{ll'} v_l^a \varpi_{ll'}^{as}\frac{\varepsilon_l-\mu}{k_B T}\partial_{\mathbf{k}}^b f_l^0 - \frac{k_B e}{\hbar}\sum_{ll'} v_l^a \varpi_{l'l}^{as}\frac{\varepsilon_l-\mu}{k_B T}\partial_{\mathbf{k}'}^b f_{l'}^0 \\ &= \frac{k_B e}{\hbar}\tau^2\sum_{ll'} \varpi_{ll'}^{as}(v_l^a - v_{l'}^a)\frac{\varepsilon_l-\mu}{k_B T}\partial_{\mathbf{k}}^b f_l^0 .\end{aligned} \tag{S103}$$

Thus, we obtain

$$\begin{aligned}\alpha_{ab}^{in} &= \frac{k_B e}{\hbar}\int d\varepsilon \frac{\varepsilon-\mu}{k_B T}\sum_l \epsilon^{abc}\Omega_l^c f_l^0 \left(-\frac{\partial f^0}{\partial \varepsilon}\right), \\ \alpha_{ab}^{sj,1} &= \frac{k_B e}{\hbar}\tau\int d\varepsilon \frac{\varepsilon-\mu}{k_B T}\sum_l v_a^{sj}\partial_{\mathbf{k}}^b f_l^0 \left(-\frac{\partial f^0}{\partial \varepsilon}\right), \\ \alpha_{ab}^{sj,2} &= -\frac{k_B e}{\hbar}\tau\int d\varepsilon \frac{\varepsilon-\mu}{k_B T}\sum_l v_b^{sj}\partial_{\mathbf{k}}^a f_l^0 \left(-\frac{\partial f^0}{\partial \varepsilon}\right), \\ \alpha_{ab}^{sk} &= \frac{k_B e}{\hbar}\tau^2\int d\varepsilon \frac{\varepsilon-\mu}{k_B T}\sum_{ll'} \varpi_{ll'}^{as}(v_l^a - v_{l'}^a)\partial_{\mathbf{k}}^b f_l^0 \left(-\frac{\partial f^0}{\partial \varepsilon}\right).\end{aligned} \tag{S104}$$

## SIV. ANOMALOUS THERMAL HALL EFFECT

### A. Intrinsic contribution

The anomalous thermal current induced by the Berry curvature is given by

$$J_{Q,a}^{in} = \frac{1}{\hbar}\partial_{\mathbf{r}}^b T\int d\varepsilon \frac{(\varepsilon-\mu)^2}{T}\sum_l \epsilon^{abc}\Omega_l^c f_l^0 \left(-\frac{\partial f^0}{\partial \varepsilon}\right). \tag{S105}$$

### B. Side-jump contribution

The first side-jump contribution comes from the side-jump velocity, which can be obtained as

$$\begin{aligned}J_{Q,a}^{sj,1} &= \sum_l (\varepsilon_l-\mu) v_a^{sj}\delta^1 f_l^{in} \\ &= \frac{1}{\hbar}\partial_{\mathbf{r}}^b T\sum_l v_a^{sj}\tau_l\frac{(\varepsilon_l-\mu)^2}{T}\partial_{\mathbf{k}}^b f_l^0 \partial_{\mathbf{r}}^b T.\end{aligned} \tag{S106}$$

The second contribution comes from the side-jump-induced modification to the distribution function

$$\begin{aligned}J_{Q,a}^{sj,2} &= \sum_l (\varepsilon_l-\mu) v_l^a \delta f_l^{sj} \\ &= -\partial_{\mathbf{r}}^b T\sum_{ll'}\frac{(\varepsilon_l-\mu)^2}{T} v_l^a \tau_l O_{ll'}^a \left(f_l^0 - f_{l'}^0\right).\end{aligned} \tag{S107}$$

### C. Skew-scattering contribution

The corresponding skew-scattering contribution can be written as

$$\begin{aligned} J_{Q,a}^{sk} &= \sum_l (\varepsilon_l - \mu) v_l^a \delta f_l^{sk} \\ &= \sum_l (\varepsilon_l - \mu) v_l^a \left[ -\partial_{\mathbf{r}}^b T \sum_{l'} \tau_l \varpi_{l'l}^{as} \frac{\tau_l}{\hbar} \frac{\varepsilon_l - \mu}{T} \partial_{\mathbf{k}}^b f_l^0 - \partial_{\mathbf{r}}^b T \sum_{l'} \tau_l \varpi_{l'l}^{as} \frac{\tau_{l'}}{\hbar} \frac{\varepsilon_{l'} - \mu}{T} \partial_{\mathbf{k}'}^b f_{l'}^0 \right] \\ &= -\frac{1}{\hbar} \partial_{\mathbf{r}}^b T \sum_{ll'} v_l^a \tau_l^2 \varpi_{l'l}^{as} \frac{(\varepsilon_l - \mu)^2}{T} \partial_{\mathbf{k}}^b f_l^0 - \frac{1}{\hbar} \partial_{\mathbf{r}}^b T \sum_{ll'} v_l^a \tau_l \tau_{l'} \varpi_{l'l}^{as} \frac{(\varepsilon_l - \mu)(\varepsilon_{l'} - \mu)}{T} \partial_{\mathbf{k}'}^b f_{l'}^0. \end{aligned} \tag{S108}$$

### D. Anomalous thermal Hall conductivity

The anomalous electric Hall conductivity can be obtained by writing that

$$J_{Q,a} = \kappa_{ab}^{tot} (-\partial_{\mathbf{r}}^b T). \tag{S109}$$

We obtain that

$$\kappa_{ab}^{tot} = \kappa_{ab}^{in} + \kappa_{ab}^{sj,1} + \kappa_{ab}^{sj,2} + \kappa_{ab}^{sk}, \tag{S110}$$

with

$$\begin{aligned} \kappa_{ab}^{in} &= -\frac{k_B^2 T}{\hbar} \int d\varepsilon \left( \frac{\varepsilon - \mu}{k_B T} \right)^2 \sum_l \epsilon^{abc} \Omega_l^c f_l^0 \left( -\frac{\partial f^0}{\partial \varepsilon} \right), \\ \kappa_{ab}^{sj,1} &= -\frac{k_B^2 T}{\hbar} \sum_l v_a^{sj} \tau_l \left( \frac{\varepsilon_l - \mu}{k_B T} \right)^2 \partial_{\mathbf{k}}^b f_l^0, \\ \kappa_{ab}^{sj,2} &= k_B^2 T \sum_{ll'} \left( \frac{\varepsilon - \mu}{k_B T} \right)^2 v_l^a \tau_l O_{ll'}^a \left( f_l^0 - f_{l'}^0 \right) \\ \kappa_{ab}^{sk} &= \frac{k_B^2 T}{\hbar} \sum_{ll'} v_l^a \tau_l^2 \varpi_{l'l}^{as} \left( \frac{\varepsilon_l - \mu}{k_B T} \right)^2 \partial_{\mathbf{k}}^b f_l^0 + \frac{k_B e}{\hbar} \sum_{ll'} v_l^a \tau_l \tau_{l'} \varpi_{l'l}^{as} \frac{(\varepsilon_l - \mu)(\varepsilon_{l'} - \mu)}{(k_B T)^2} \partial_{\mathbf{k}'}^b f_{l'}^0. \end{aligned} \tag{S111}$$

In the isotropic limit, the general relaxation time $\tau_l$ can be considered as a constant $\tau$. Thus, the general expressions can be further simplified,

$$\begin{aligned} \kappa_{ab}^{in} &= -\frac{k_B^2 T}{\hbar} \int d\varepsilon \left( \frac{\varepsilon - \mu}{k_B T} \right)^2 \sum_l \epsilon^{abc} \Omega_l^c f_l^0 \left( -\frac{\partial f^0}{\partial \varepsilon} \right), \\ \kappa_{ab}^{sj,1} &= -\frac{k_B^2 T}{\hbar} \tau \int d\varepsilon \left( \frac{\varepsilon - \mu}{k_B T} \right)^2 \sum_l v_a^{sj} \partial_{\mathbf{k}}^b f_l^0 \left( -\frac{\partial f^0}{\partial \varepsilon} \right), \\ \kappa_{ab}^{sj,2} &= \frac{k_B^2 T}{\hbar} \tau \int d\varepsilon \left( \frac{\varepsilon - \mu}{k_B T} \right)^2 \sum_l v_b^{sj} \partial_{\mathbf{k}}^a f_l^0 \left( -\frac{\partial f^0}{\partial \varepsilon} \right), \\ \kappa_{ab}^{sk} &= -\frac{k_B^2 T}{\hbar} \tau^2 \int d\varepsilon \left( \frac{\varepsilon - \mu}{k_B T} \right)^2 \sum_{ll'} \varpi_{ll'}^{as} (v_l^a - v_{l'}^a) \partial_{\mathbf{k}}^b f_l^0 \left( -\frac{\partial f^0}{\partial \varepsilon} \right). \end{aligned} \tag{S112}$$

## SV. 2-BAND SYSTEM

### A. Eigen solutions

To get the analytic results, we use the 2-band system as an example. For a 2-band system, a general minimal model can be always given as

$$\hat{\mathcal{H}} = \mathbf{r} \cdot \sigma, \tag{S113}$$

where $\mathbf{r} = (r_x, r_y, r_z)$ is the vector in the parameter space, $\sigma = (\sigma_x, \sigma_y, \sigma_z)$ is the Pauli matrix vector. The band dispersion reads

$$\varepsilon_{\mathbf{k}}^{\pm} = \pm r, \tag{S114}$$

with $r \equiv \sqrt{r_x^2 + r_y^2 + r_z^2}$. The chiral basis vectors that diagonalize the Hamiltonian are

$$\psi_{\mathbf{k}}^{\pm} = \frac{e^{i\mathbf{k}\cdot\mathbf{r}}}{\sqrt{\mathcal{V}}} |u_{\mathbf{k}}^{\pm}\rangle, \tag{S115}$$

where $\mathcal{V}$ refers to the general volume and

$$|u_{\mathbf{k}}^{+}\rangle = \begin{bmatrix} \cos\frac{\theta}{2} \\ \sin\frac{\theta}{2} e^{i\phi} \end{bmatrix}, \qquad |u_{\mathbf{k}}^{-}\rangle = \begin{bmatrix} \sin\frac{\theta}{2} \\ -\cos\frac{\theta}{2} e^{i\phi} \end{bmatrix} \tag{S116}$$

are the eigenstates with

$$\cos\theta = \frac{r_z}{r}, \qquad \tan\phi = \frac{r_y}{r_x}. \tag{S117}$$

### B. Scattering rate

Firstly, the scattering $T$-matrix is defined as

$$T_{ll'} = \langle \psi_l | \hat{V}_{imp} | \Psi_{l'} \rangle. \tag{S118}$$

Here $|\Psi_{l'}\rangle$ is the eigenstates of the full Hamiltonian $\hat{\mathcal{H}} = \hat{\mathcal{H}}_0 + \hat{V}_{imp}$ that satisfies the Lippman-Schwinger equation

$$|\Psi_l\rangle = |\psi_l\rangle + \frac{\hat{V}_{imp}}{\varepsilon_l - \hat{\mathcal{H}}_0 + i\delta} |\Psi_l\rangle. \tag{S119}$$

For weak disorder one can approximate the scattering state. For weak disorder one can approximate the scattering state $\Psi_l$ by a truncated series in powers of $V_{ll'} = \langle \psi_l | \hat{V}_{imp} | \psi_{l'} \rangle$ as

$$|\Psi_{l'}\rangle = |\psi_{l'}\rangle + \sum_{l''} \frac{V_{l''l'}}{\varepsilon_{l'} - \varepsilon_{l''} + i\delta} |\psi_{l''}\rangle + \sum_{l''} \sum_{l'''} \frac{V_{l''l'''} V_{l'''l'}}{(\varepsilon_{l'} - \varepsilon_{l''} + i\delta)(\varepsilon_{l'} - \varepsilon_{l'''} + i\delta)} |\psi_{l''}\rangle + \cdots . \tag{S120}$$

Thus, the $T$-matrix reads

$$T_{ll'} = V_{ll'} + \sum_{l''} \frac{V_{ll''} V_{l''l'}}{\varepsilon_{l'} - \varepsilon_{l''} + i\delta} + \sum_{l''} \sum_{l'''} \frac{V_{ll''} V_{l''l'''} V_{l'''l'}}{(\varepsilon_{l'} - \varepsilon_{l''} + i\delta)(\varepsilon_{l'} - \varepsilon_{l'''} + i\delta)} + \cdots , \tag{S121}$$

according to the Fermi golden rule, the scattering rate is given by

$$\varpi_{ll'} \equiv \frac{2\pi}{\hbar} |T_{ll'}|^2 \delta(\varepsilon_l - \varepsilon_{l'}) \equiv \varpi_{ll'}^{(2)} + \varpi_{ll'}^{(3)} + \varpi_{ll'}^{(4)} + \cdots , \tag{S122}$$

with

$$\begin{aligned}
\varpi_{ll'}^{(2)} &= \frac{2\pi}{\hbar} \langle V_{ll'}^* V_{ll'} \rangle_{dis} \delta(\varepsilon_l - \varepsilon_{l'}), \\
\varpi_{ll'}^{(3)} &= \frac{2\pi}{\hbar} \sum_{l''} \left( \frac{\langle V_{ll'}^* V_{ll''} V_{l''l'} \rangle_{dis}}{\varepsilon_{l'} - \varepsilon_{l''} + i\delta} + \frac{\langle V_{ll''}^* V_{l''l'}^* V_{ll'} \rangle_{dis}}{\varepsilon_{l'} - \varepsilon_{l''} - i\delta} \right) \delta(\varepsilon_l - \varepsilon_{l'}), \\
\varpi_{ll'}^{(4)} &= \frac{2\pi}{\hbar} \sum_{l''} \sum_{l'''} \left[ \frac{\langle V_{ll''}^* V_{l''l'}^* V_{ll''} V_{l''l'} \rangle_{dis}}{(\varepsilon_{l'} - \varepsilon_{l''} - i\delta)(\varepsilon_{l'} - \varepsilon_{l'''} + i\delta)} + \frac{\langle V_{ll'}^* V_{ll''} V_{l''l'''} V_{l'''l'} \rangle_{dis}}{(\varepsilon_{l'} - \varepsilon_{l''} + i\delta)(\varepsilon_{l'} - \varepsilon_{l'''} + i\delta)} \right. \\
&\quad \left. + \frac{\langle V_{ll''}^* V_{l''l'''}^* V_{l'''l'}^* V_{ll'} \rangle_{dis}}{(\varepsilon_{l'} - \varepsilon_{l''} - i\delta)(\varepsilon_{l'} - \varepsilon_{l'''} - i\delta)} \right] \delta(\varepsilon_l - \varepsilon_{l'}).
\end{aligned} \tag{S123}$$

We consider the model of randomly located $\delta$-function scatterers

$$\hat{V}_{imp} = \sum_i V_i \delta(\mathbf{r} - \mathbf{R}_i), \tag{S124}$$

with the random distribution $R_i$ and the disorder strength $V_i$ satisfying $\langle V_i \rangle_{dis} = 0$, $\langle V_i^2 \rangle_{dis} = V_0^2$, $\langle V_i^3 \rangle_{dis} = V_1^3$. In the eigenstate representation the operator elements of the disorder potential can be written in a general form as

$$\begin{aligned} V_{\mathbf{k}\mathbf{k}'}^{\eta\eta'} &= \langle \psi_{\mathbf{k}}^{\eta} | \hat{V}_{imp} | \psi_{\mathbf{k}'}^{\eta'} \rangle \\ &= \frac{1}{\mathcal{V}} \int d^3\mathbf{r} \langle u_{\mathbf{k}}^{\eta} | e^{-i\mathbf{k}\cdot\mathbf{r}} \left[ \sum_i V_i \delta(\mathbf{r} - \mathbf{R}_i) \right] e^{i\mathbf{k}'\cdot\mathbf{r}} | u_{\mathbf{k}'}^{\eta'} \rangle \\ &= \frac{1}{\mathcal{V}} \int d^3\mathbf{r} \langle u_{\mathbf{k}}^{\eta} | \sum_i V_i \delta(\mathbf{r} - \mathbf{R}_i) e^{i(\mathbf{k}'-\mathbf{k})\cdot\mathbf{r}} | u_{\mathbf{k}'}^{\eta'} \rangle \\ &= V_{\mathbf{k}\mathbf{k}'}^0 \langle u_{\mathbf{k}}^{\eta} | u_{\mathbf{k}'}^{\eta'} \rangle, \end{aligned} \tag{S125}$$

where $V_{\mathbf{k}\mathbf{k}'}^0$ is the orbital disorder matrix element defined as

$$V_{\mathbf{k}\mathbf{k}'}^0 = \sum_i V_i e^{i(\mathbf{k}'-\mathbf{k})R_i}. \tag{S126}$$

Thus, we can obtain

$$\begin{aligned} V_{\mathbf{k}\mathbf{k}'} &= V_{\mathbf{k}\mathbf{k}'}^0 \begin{bmatrix} \langle u_{\mathbf{k}}^{+} | u_{\mathbf{k}'}^{+} \rangle & \langle u_{\mathbf{k}}^{+} | u_{\mathbf{k}'}^{-} \rangle \\ \langle u_{\mathbf{k}}^{-} | u_{\mathbf{k}'}^{+} \rangle & \langle u_{\mathbf{k}}^{-} | u_{\mathbf{k}'}^{-} \rangle \end{bmatrix} \\ &= V_{\mathbf{k}\mathbf{k}'}^0 \begin{bmatrix} \cos\theta/2\cos\theta'/2 + \sin\theta'/2\sin\theta'/2 e^{i(\phi'-\phi)} & \cos\theta/2\sin\theta'/2 - \sin\theta'/2\cos\theta'/2 e^{i(\phi'-\phi)} \\ \sin\theta/2\cos\theta'/2 + \cos\theta'/2\sin\theta'/2 e^{i(\phi'-\phi)} & \sin\theta/2\sin\theta'/2 + \cos\theta'/2\cos\theta'/2 e^{i(\phi'-\phi)} \end{bmatrix} \\ &= V_{\mathbf{k}\mathbf{k}'}^0 \begin{bmatrix} \mathcal{U}_{11} & \mathcal{U}_{12} \\ \mathcal{U}_{21} & \mathcal{U}_{22} \end{bmatrix}, \end{aligned} \tag{S127}$$

with

$$\begin{aligned} \mathcal{U}_{11} &= \frac{1}{4} \left[ (e^{i\theta/2} + e^{i\theta/2})(e^{i\theta'/2} + e^{i\theta'/2}) - (e^{i\theta/2} - e^{i\theta/2})(e^{i\theta'/2} - e^{i\theta'/2}) e^{i(\phi'-\phi)} \right], \\ \mathcal{U}_{12} &= \frac{1}{4i} \left[ (e^{i\theta/2} + e^{i\theta/2})(e^{i\theta'/2} - e^{i\theta'/2}) - (e^{i\theta/2} - e^{i\theta/2})(e^{i\theta'/2} + e^{i\theta'/2}) e^{i(\phi'-\phi)} \right], \\ \mathcal{U}_{21} &= \frac{1}{4i} \left[ (e^{i\theta/2} - e^{i\theta/2})(e^{i\theta'/2} + e^{i\theta'/2}) + (e^{i\theta/2} - e^{i\theta/2})(e^{i\theta'/2} + e^{i\theta'/2}) e^{i(\phi'-\phi)} \right], \\ \mathcal{U}_{22} &= -\frac{1}{4} \left[ (e^{i\theta/2} - e^{i\theta/2})(e^{i\theta'/2} - e^{i\theta'/2}) - (e^{i\theta/2} + e^{i\theta/2})(e^{i\theta'/2} + e^{i\theta'/2}) e^{i(\phi'-\phi)} \right]. \end{aligned} \tag{S128}$$

One can rewrite this expression in a compact style

$$\begin{aligned} V_{\mathbf{k}\mathbf{k}'}^{\eta\eta'} &= V_{\mathbf{k},\mathbf{k}'}^0 \frac{i^{(\eta+\eta')/2-1}}{4} \left[ (e^{i\theta/2} + \eta e^{-i\theta/2})(e^{i\theta'/2} + \eta' e^{-i\theta'/2}) - (e^{i\theta/2} - \eta e^{-i\theta/2})(e^{i\theta'/2} - \eta' e^{-i\theta'/2}) e^{i(\phi'-\phi)} \right] \\ &= V_{\mathbf{k},\mathbf{k}'}^0 \frac{i^{\left(\eta+\eta'\right)/2-1}}{4} \left\{ \left[ e^{i(\theta+\theta')/2} + \eta\eta' e^{-i(\theta+\theta')/2} \right] \left[ 1 - e^{i(\phi'-\phi)} \right] + \left[ \eta e^{-i(\theta-\theta')/2} + \eta' e^{i(\theta-\theta')/2} \right] \left[ 1 + e^{i(\phi'-\phi)} \right] \right\} \\ &\equiv V_{\mathbf{k},\mathbf{k}'}^0 \Xi_{\varphi\varphi'}^{\eta\eta'}, \end{aligned} \tag{S129}$$

with

$$\Xi_{\varphi\varphi'}^{\eta\eta'} = \frac{i^{\left(\eta+\eta'\right)/2-1}}{4} \left\{ \left[ e^{i(\theta+\theta')/2} + \eta\eta' e^{-i(\theta+\theta')/2} \right] \left[ 1 - e^{i(\phi'-\phi)} \right] + \left[ \eta e^{-i(\theta-\theta')/2} + \eta' e^{i(\theta-\theta')/2} \right] \left[ 1 + e^{i(\phi'-\phi)} \right] \right\}, \tag{S130}$$

where $\eta, \eta' \in \pm$ are the band indexes, $\varphi \in (\theta, \phi)$ represents the combined angular index. For its complex conjugate, we have

$$(V_{\mathbf{k}\mathbf{k}'}^{\eta\eta'})^* = (V_{\mathbf{k},\mathbf{k}'}^0)^* \tilde{\Xi}_{\varphi\varphi'}^{\eta\eta'}, \tag{S131}$$

where we have denoted $\tilde{\Xi}_{\varphi\varphi'}^{\eta\eta'} = (\Xi_{\varphi\varphi'}^{\eta\eta'})^*$.

### 1. Second-order scattering rate

Assume that the Fermi energy lies in the upper band, thus we have

$$\begin{aligned}\varpi^{(2)}_{\mathbf{k}\mathbf{k}'} &= \frac{2\pi}{\hbar}\langle V^*_{ll'}V_{ll'}\rangle_{dis}\delta(\varepsilon_l-\varepsilon_{l'})\\ &= \frac{2\pi}{\hbar}\langle (V^{++}_{\mathbf{k},\mathbf{k}'})^* V^{++}_{\mathbf{k},\mathbf{k}'}\rangle_{dis}\delta(\varepsilon^+_{\mathbf{k}}-\varepsilon^+_{\mathbf{k}'})\\ &= \frac{2\pi}{\hbar}\langle (V^{0}_{\mathbf{k},\mathbf{k}'})^* V^{0}_{\mathbf{k},\mathbf{k}'}\rangle_{dis}\tilde{\Xi}^{++}_{\varphi\varphi'}\Xi^{++}_{\varphi\varphi'}\delta(\varepsilon^+_{\mathbf{k}}-\varepsilon^+_{\mathbf{k}'})\\ &= \frac{\pi}{\hbar}n_iV_0^2\left[1+\cos\theta\cos\theta'+\sin\theta\sin\theta'\cos(\phi-\phi')\right]\delta(\varepsilon^+_{\mathbf{k}}-\varepsilon^+_{\mathbf{k}'}),\end{aligned} \tag{S132}$$

where we have used

$$\langle (V^{0}_{\mathbf{k},\mathbf{k}'})^* V^{0}_{\mathbf{k},\mathbf{k}'}\rangle_{dis} \simeq n_iV_0^2. \tag{S133}$$

### 2. Third-order scattering rate

The third-order scattering term for the upper band is

$$\begin{aligned}\varpi^{(3)}_{\mathbf{k}\mathbf{k}'} &= \frac{2\pi}{\hbar}\sum_{l''}\left(\frac{\langle V^*_{ll'}V_{ll''}V_{l''l'}\rangle_{dis}}{\varepsilon_{l'}-\varepsilon_{l''}+i\delta}+c.c.\right)\delta(\varepsilon_l-\varepsilon_{l'}),\\ &= \frac{2\pi}{\hbar}\int[d\mathbf{k}'']\left(\frac{\langle (V^{++}_{\mathbf{k}\mathbf{k}'})^*V^{+\eta}_{\mathbf{k}\mathbf{k}''}V^{\eta+}_{\mathbf{k}''\mathbf{k}'}\rangle_{dis}}{\varepsilon^+_{\mathbf{k}}-\varepsilon^\eta_{\mathbf{k}''}+i\delta}+c.c.\right)\delta(\varepsilon^+_{\mathbf{k}}-\varepsilon^+_{\mathbf{k}'}).\end{aligned} \tag{S134}$$

For $\eta=+$, we have

$$\begin{aligned}\varpi^{(3-1)}_{\mathbf{k}\mathbf{k}'} &= \frac{2\pi}{\hbar}\int[d\mathbf{k}'']\left(\frac{\langle (V^{++}_{\mathbf{k}\mathbf{k}'})^*V^{++}_{\mathbf{k}\mathbf{k}''}V^{++}_{\mathbf{k}''\mathbf{k}'}\rangle_{dis}}{\varepsilon^+_{\mathbf{k}}-\varepsilon^+_{\mathbf{k}''}+i\delta}+c.c.\right)\delta(\varepsilon^+_{\mathbf{k}}-\varepsilon^+_{\mathbf{k}'})\\ &= \frac{2\pi}{\hbar}\int[d\mathbf{k}'']\left[\mathcal{P}\left(\frac{\langle (V^{++}_{\mathbf{k}\mathbf{k}'})^*V^{++}_{\mathbf{k}\mathbf{k}''}V^{++}_{\mathbf{k}''\mathbf{k}'}\rangle_{dis}}{\varepsilon^+_{\mathbf{k}}-\varepsilon^+_{\mathbf{k}''}+i\delta}\right)+2\pi\mathrm{Im}\langle (V^{++}_{\mathbf{k}\mathbf{k}'})^*V^{++}_{\mathbf{k}\mathbf{k}''}V^{++}_{\mathbf{k}''\mathbf{k}'}\rangle_{dis}\delta(\varepsilon^+_{\mathbf{k}}-\varepsilon^+_{\mathbf{k}''})\right]\delta(\varepsilon^+_{\mathbf{k}}-\varepsilon^+_{\mathbf{k}'}),\end{aligned} \tag{S135}$$

where we have used the identity

$$\frac{z}{x+i\delta}+\frac{z^*}{x-i\delta}=\mathcal{P}\left(\frac{z}{x}\right)-i\pi z\delta(x)+\mathcal{P}\left(\frac{z^*}{x}\right)+i\pi z^*\delta(x)=\mathcal{P}\left(\frac{2\mathrm{Re}z}{x}\right)+2\pi\mathrm{Im}z\delta(x). \tag{S136}$$

The $\varpi^{(3)}_{ll'}$ has the symmetric and antisymmetric parts, the symmetric part is not essential since it only renormalizes the second-order result ($\varpi^{(2)}_{ll'}$ is symmetric). The antisymmetric part can be written as

$$\begin{aligned}\varpi^{(3a-1)}_{\mathbf{k}\mathbf{k}'} &= \frac{2\pi}{\hbar}\int[d\mathbf{k}'']2\pi\mathrm{Im}\langle (V^{++}_{\mathbf{k}\mathbf{k}'})^*V^{++}_{\mathbf{k}\mathbf{k}''}V^{++}_{\mathbf{k}''\mathbf{k}'}\rangle_{dis}\delta(\varepsilon^+_{\mathbf{k}}-\varepsilon^+_{\mathbf{k}''})\delta(\varepsilon^+_{\mathbf{k}}-\varepsilon^+_{\mathbf{k}'})\\ &= \frac{4\pi^2}{\hbar}n_iV_1^3\int[d\mathbf{k}'']\mathrm{Im}\left[\tilde{\Xi}^{++}_{\varphi\varphi'}\Xi^{++}_{\varphi\varphi''}\Xi^{++}_{\varphi''\varphi'}\right]\delta(\varepsilon^+_{\mathbf{k}}-\varepsilon^+_{\mathbf{k}''})\delta(\varepsilon^+_{\mathbf{k}}-\varepsilon^+_{\mathbf{k}'})\\ &= \frac{\pi^2n_iV_1^3}{\hbar}\int[d\mathbf{k}'']\left[\sin\theta\sin\theta'\cos\theta''\sin(\phi-\phi')+\sin\theta'\sin\theta''\cos\theta\sin(\phi'-\phi'')\right.\\ &\quad\left.+\sin\theta\sin\theta''\cos\theta'\sin(\phi''-\phi)\right]\delta(\varepsilon^+_{\mathbf{k}}-\varepsilon^+_{\mathbf{k}''})\delta(\varepsilon^+_{\mathbf{k}}-\varepsilon^+_{\mathbf{k}'}),\end{aligned} \tag{S137}$$

where we have used

$$\langle (V^{0}_{\mathbf{k}\mathbf{k}'})^*V^{0}_{\mathbf{k}\mathbf{k}''}V^{0}_{\mathbf{k}''\mathbf{k}'}\rangle_{dis}\simeq n_iV_1^3. \tag{S138}$$

For $\eta=-$, we have

$$\begin{aligned}\varpi^{(3a-2)}_{\mathbf{k}\mathbf{k}'} &= \frac{2\pi}{\hbar}\int[d\mathbf{k}'']2\pi\mathrm{Im}\langle (V^{++}_{\mathbf{k}\mathbf{k}'})^*V^{+-}_{\mathbf{k}\mathbf{k}''}V^{-+}_{\mathbf{k}''\mathbf{k}'}\rangle_{dis}\delta(\varepsilon^+_{\mathbf{k}}-\varepsilon^-_{\mathbf{k}''})\delta(\varepsilon^+_{\mathbf{k}}-\varepsilon^+_{\mathbf{k}'})\\ &= \frac{4\pi^2}{\hbar}n_iV_1^3\int[d\mathbf{k}'']\mathrm{Im}\left[\tilde{\Xi}^{++}_{\varphi\varphi'}\Xi^{+-}_{\varphi\varphi''}\Xi^{-+}_{\varphi''\varphi'}\right]\delta(\varepsilon^+_{\mathbf{k}}-\varepsilon^-_{\mathbf{k}''})\delta(\varepsilon^+_{\mathbf{k}}-\varepsilon^+_{\mathbf{k}'})\\ &= 0.\end{aligned} \tag{S139}$$

Except for the degenerate case, which is out of our consideration, we all have $\delta(\varepsilon^{+}_{\mathbf{k}} - \varepsilon^{-}_{\mathbf{k}''}) = 0$. Therefore, the third-order scattering rate is

$$\varpi^{(3a)}_{\mathbf{k}\mathbf{k}'} = \frac{\pi^2 n_i V_1^3}{\hbar} \int [d\mathbf{k}''] \left[\sin\theta \sin\theta' \cos\theta'' \sin(\phi - \phi') + \sin\theta' \sin\theta'' \cos\theta \sin(\phi' - \phi'') \right. \\ \left. + \sin\theta \sin\theta'' \cos\theta' \sin(\phi'' - \phi)\right] \delta(\varepsilon^{+}_{\mathbf{k}} - \varepsilon^{+}_{\mathbf{k}''}) \delta(\varepsilon^{+}_{\mathbf{k}} - \varepsilon^{+}_{\mathbf{k}'}). \tag{S140}$$

### *3. Fourth-order scattering rate*

The forth-order scattering terms for the upper band are

$$\varpi^{(4)}_{\mathbf{k}\mathbf{k}'} = \frac{2\pi}{\hbar} \int [d\mathbf{k}''] \int [d\mathbf{k}'''] \left[ \frac{\langle (V^{+\eta}_{\mathbf{k}\mathbf{k}''})^* (V^{\eta +}_{\mathbf{k}''\mathbf{k}'})^* V^{+\eta'}_{\mathbf{k}\mathbf{k}''} V^{\eta' +}_{\mathbf{k}''\mathbf{k}'} \rangle_{dis}}{(\varepsilon^{+}_{\mathbf{k}'} - \varepsilon^{\eta}_{\mathbf{k}''} - i\delta)(\varepsilon^{+}_{\mathbf{k}'} - \varepsilon^{\eta'}_{\mathbf{k}'''} + i\delta)} + \frac{\langle (V^{++}_{\mathbf{k}\mathbf{k}'})^* V^{+\eta}_{\mathbf{k}\mathbf{k}''} V^{\eta\eta'}_{\mathbf{k}''\mathbf{k}'''} V^{\eta' +}_{\mathbf{k}'''\mathbf{k}'} \rangle_{dis}}{(\varepsilon^{+}_{\mathbf{k}'} - \varepsilon^{\eta}_{\mathbf{k}''} + i\delta)(\varepsilon^{+}_{\mathbf{k}'} - \varepsilon^{\eta'}_{\mathbf{k}'''} + i\delta)} \right. \\ \left. + \frac{\langle V^{++}_{\mathbf{k}\mathbf{k}'} (V^{+\eta}_{\mathbf{k}\mathbf{k}''})^* (V^{\eta\eta'}_{\mathbf{k}''\mathbf{k}'''})^* (V^{\eta' +}_{\mathbf{k}'''\mathbf{k}'})^* \rangle_{dis}}{(\varepsilon^{+}_{\mathbf{k}'} - \varepsilon^{+}_{\mathbf{k}''} - i\delta)(\varepsilon^{+}_{\mathbf{k}'} - \varepsilon^{+}_{\mathbf{k}'''} - i\delta)} \right] \delta(\varepsilon^{+}_{\mathbf{k}} - \varepsilon^{+}_{\mathbf{k}'}). \tag{S141}$$

Note that we did not take into account the fourth-order correlations, thus the disorder average in the above equality have to be decomposed into the products of the second-order correlations. According to the Wick's theorem, the numerator of the first term reads

$$\begin{aligned} \langle (V^{+\eta}_{\mathbf{k}\mathbf{k}''})^* (V^{\eta +}_{\mathbf{k}''\mathbf{k}'})^* V^{+\eta'}_{\mathbf{k}\mathbf{k}'''} V^{\eta' +}_{\mathbf{k}'''\mathbf{k}'} \rangle_{dis} =& \langle (V^{+\eta}_{\mathbf{k}\mathbf{k}''})^* (V^{\eta +}_{\mathbf{k}''\mathbf{k}'})^* \rangle_{dis} \langle V^{+\eta'}_{\mathbf{k}\mathbf{k}'''} V^{\eta' +}_{\mathbf{k}'''\mathbf{k}'} \rangle_{dis} \\ &+ \langle (V^{+\eta}_{\mathbf{k}\mathbf{k}''})^* V^{+\eta'}_{\mathbf{k}\mathbf{k}'''} \rangle_{dis} \langle V^{\eta' +}_{\mathbf{k}'''\mathbf{k}'} (V^{\eta +}_{\mathbf{k}''\mathbf{k}'})^* \rangle_{dis} \\ &+ \langle (V^{+\eta}_{\mathbf{k}\mathbf{k}''})^* V^{\eta' +}_{\mathbf{k}'''\mathbf{k}'} \rangle_{dis} \langle V^{+\eta'}_{\mathbf{k}\mathbf{k}'''} (V^{\eta +}_{\mathbf{k}''\mathbf{k}'})^* \rangle_{dis}, \end{aligned} \tag{S142}$$

the numerator of the second term

$$\begin{aligned} \langle (V^{++}_{\mathbf{k}\mathbf{k}'})^* V^{+\eta}_{\mathbf{k}\mathbf{k}''} V^{\eta\eta'}_{\mathbf{k}''\mathbf{k}'''} V^{\eta' +}_{\mathbf{k}'''\mathbf{k}'} \rangle_{dis} =& \langle (V^{++}_{\mathbf{k}\mathbf{k}'})^* V^{+\eta}_{\mathbf{k}\mathbf{k}''} \rangle_{dis} \langle V^{\eta\eta'}_{\mathbf{k}''\mathbf{k}'''} V^{\eta' +}_{\mathbf{k}'''\mathbf{k}'} \rangle_{dis} \\ &+ \langle (V^{++}_{\mathbf{k}\mathbf{k}'})^* V^{\eta' +}_{\mathbf{k}'''\mathbf{k}'} \rangle_{dis} \langle V^{+\eta}_{\mathbf{k}\mathbf{k}''} V^{\eta\eta'}_{\mathbf{k}''\mathbf{k}'''} \rangle_{dis} \\ &+ \langle (V^{++}_{\mathbf{k}\mathbf{k}'})^* V^{\eta\eta'}_{\mathbf{k}''\mathbf{k}'''} \rangle_{dis} \langle V^{+\eta}_{\mathbf{k}\mathbf{k}''} V^{\eta' +}_{\mathbf{k}'''\mathbf{k}'} \rangle_{dis}, \end{aligned} \tag{S143}$$

and the numerator of the third term

$$\begin{aligned} \langle V^{++}_{\mathbf{k}\mathbf{k}'} (V^{+\eta}_{\mathbf{k}\mathbf{k}''})^* (V^{\eta\eta'}_{\mathbf{k}''\mathbf{k}'''})^* (V^{\eta' +}_{\mathbf{k}'''\mathbf{k}'})^* \rangle_{dis} =& \langle V^{+}_{\mathbf{k}\mathbf{k}'} (V^{+\eta}_{\mathbf{k}\mathbf{k}''})^* \rangle_{dis} \langle (V^{\eta\eta'}_{\mathbf{k}''\mathbf{k}'''})^* (V^{\eta' +}_{\mathbf{k}'''\mathbf{k}'})^* \rangle_{dis} \\ &+ \langle V^{++}_{\mathbf{k}\mathbf{k}'} (V^{\eta' +}_{\mathbf{k}'''\mathbf{k}'})^* \rangle_{dis} \langle (V^{+\eta}_{\mathbf{k}\mathbf{k}''})^* (V^{\eta\eta'}_{\mathbf{k}''\mathbf{k}'''})^* \rangle_{dis} \\ &+ \langle V^{++}_{\mathbf{k}\mathbf{k}'} (V^{\eta\eta'}_{\mathbf{k}''\mathbf{k}'''})^* \rangle_{dis} \langle (V^{+\eta}_{\mathbf{k}\mathbf{k}''})^* (V^{\eta' +}_{\mathbf{k}'''\mathbf{k}'})^* \rangle_{dis}. \end{aligned} \tag{S144}$$

Within the non-crossing approximation, only three independent terms contributes

$$\varpi^{(4)}_{\mathbf{k}\mathbf{k}'} = \varpi^{(4-1)}_{\mathbf{k}\mathbf{k}'} + \varpi^{(4-2)}_{\mathbf{k}\mathbf{k}'} + \varpi^{(4-3)}_{\mathbf{k}\mathbf{k}'}, \tag{S145}$$

with

$$
\begin{aligned}
\varpi_{\mathbf{k}\mathbf{k}'}^{(4-1)} &= \frac{2\pi}{\hbar}\int[d\mathbf{k}'']\int[d\mathbf{k}''']\left[\frac{\langle (V_{\mathbf{k}\mathbf{k}''}^{+\eta})^* V_{\mathbf{k}\mathbf{k}'''}^{+\eta'}\rangle_{dis}\langle V_{\mathbf{k}'''\mathbf{k}'}^{\eta'+}(V_{\mathbf{k}''\mathbf{k}'}^{\eta+})^*\rangle_{dis}}{(\varepsilon_{\mathbf{k}'}^{+}-\varepsilon_{\mathbf{k}''}^{\eta}-i\delta)(\varepsilon_{\mathbf{k}'}^{+}-\varepsilon_{\mathbf{k}'''}^{\eta'}+i\delta)}\right]\delta(\varepsilon_{\mathbf{k}}^{+}-\varepsilon_{\mathbf{k}'}^{+}) \\
&= \frac{2\pi n_i^2 V_0^4}{\hbar}\int[d\mathbf{k}'']\frac{\tilde{\Xi}_{\varphi\varphi''}^{+\eta}\Xi_{\varphi\varphi''}^{+\eta'}\Xi_{\varphi''\varphi'}^{\eta'+}\tilde{\Xi}_{\varphi''\varphi'}^{\eta+}}{(\varepsilon_{\mathbf{k}'}^{+}-\varepsilon_{\mathbf{k}''}^{\eta}-i\delta)(\varepsilon_{\mathbf{k}'}^{+}-\varepsilon_{\mathbf{k}''}^{\eta'}+i\delta)}\delta(\varepsilon_{\mathbf{k}}^{+}-\varepsilon_{\mathbf{k}'}^{+}), \\
\varpi_{\mathbf{k}\mathbf{k}'}^{(4-2)} &= \frac{2\pi}{\hbar}\int[d\mathbf{k}'']\int[d\mathbf{k}''']\left[\frac{\langle (V_{\mathbf{k}\mathbf{k}'}^{++})^* V_{\mathbf{k}\mathbf{k}''}^{+\eta}\rangle_{dis}\langle V_{\mathbf{k}''\mathbf{k}'''}^{\eta\eta'}V_{\mathbf{k}'''\mathbf{k}'}^{\eta'+}\rangle_{dis}}{(\varepsilon_{\mathbf{k}'}^{+}-\varepsilon_{\mathbf{k}''}^{\eta}+i\delta)(\varepsilon_{\mathbf{k}'}^{+}-\varepsilon_{\mathbf{k}'''}^{\eta'}+i\delta)}+c.c.\right]\delta(\varepsilon_{\mathbf{k}}^{+}-\varepsilon_{\mathbf{k}'}^{+}) \\
&= \frac{2\pi n_i^2 V_0^4}{\hbar}\int[d\mathbf{k}'']\left[\frac{\tilde{\Xi}_{\varphi\varphi'}^{++}\Xi_{\varphi\varphi'}^{+\eta}\Xi_{\varphi'\varphi''}^{\eta\eta'}\Xi_{\varphi''\varphi'}^{\eta'+}}{(\varepsilon_{\mathbf{k}'}^{+}-\varepsilon_{\mathbf{k}'}^{\eta}+i\delta)(\varepsilon_{\mathbf{k}'}^{+}-\varepsilon_{\mathbf{k}''}^{\eta'}+i\delta)}+c.c.\right]\delta(\varepsilon_{\mathbf{k}}^{+}-\varepsilon_{\mathbf{k}'}^{+}), \\
\varpi_{\mathbf{k}\mathbf{k}'}^{(4-3)} &= \frac{2\pi}{\hbar}\int[d\mathbf{k}'']\int[d\mathbf{k}''']\left[\frac{\langle (V_{\mathbf{k}\mathbf{k}'}^{++})^* V_{\mathbf{k}'''\mathbf{k}'}^{\eta'+}\rangle_{dis}\langle V_{\mathbf{k}\mathbf{k}''}^{+\eta}V_{\mathbf{k}''\mathbf{k}'''}^{\eta\eta'}\rangle_{dis}}{(\varepsilon_{\mathbf{k}'}^{+}-\varepsilon_{\mathbf{k}''}^{\eta}+i\delta)(\varepsilon_{\mathbf{k}'}^{+}-\varepsilon_{\mathbf{k}'''}^{\eta'}+i\delta)}+c.c.\right]\delta(\varepsilon_{\mathbf{k}}^{+}-\varepsilon_{\mathbf{k}'}^{+}) \\
&= \frac{2\pi n_i^2 V_0^4}{\hbar}\int[d\mathbf{k}'']\left[\frac{\tilde{\Xi}_{\varphi\varphi'}^{++}\Xi_{\varphi\varphi'}^{\eta'+}\Xi_{\varphi\varphi''}^{+\eta}\Xi_{\varphi''\varphi}^{\eta\eta'}}{(\varepsilon_{\mathbf{k}'}^{+}-\varepsilon_{\mathbf{k}''}^{\eta}+i\delta)(\varepsilon_{\mathbf{k}'}^{+}-\varepsilon_{\mathbf{k}}^{\eta'}+i\delta)}+c.c.\right]\delta(\varepsilon_{\mathbf{k}}^{+}-\varepsilon_{\mathbf{k}'}^{+}).
\end{aligned}
\tag{S146}
$$

Similar to the third order, we only need consider the antisymmetric part $\varpi_{\mathbf{k}\mathbf{k}'}^{(4a-n)} = (\varpi_{\mathbf{k}\mathbf{k}'}^{(4a-n)} - \varpi_{\mathbf{k}'\mathbf{k}}^{(4a-n)})/2$. Thus, we have

$$
\begin{aligned}
\varpi_{\mathbf{k}\mathbf{k}'}^{(4a-1)} &= \frac{\pi n_i^2 V_0^4}{\hbar}\int[d\mathbf{k}'']\frac{\tilde{\Xi}_{\varphi\varphi''}^{+\eta}\Xi_{\varphi\varphi''}^{+\eta'}\Xi_{\varphi''\varphi'}^{\eta'+}\tilde{\Xi}_{\varphi''\varphi'}^{\eta+}-\tilde{\Xi}_{\varphi'\varphi''}^{+\eta}\Xi_{\varphi'\varphi''}^{+\eta'}\Xi_{\varphi''\varphi}^{\eta'+}\tilde{\Xi}_{\varphi''\varphi}^{\eta+}}{(\varepsilon_{\mathbf{k}'}^{+}-\varepsilon_{\mathbf{k}''}^{\eta}-i\delta)(\varepsilon_{\mathbf{k}'}^{+}-\varepsilon_{\mathbf{k}''}^{\eta'}+i\delta)}\delta(\varepsilon_{\mathbf{k}}^{+}-\varepsilon_{\mathbf{k}'}^{+}), \\
\varpi_{\mathbf{k}\mathbf{k}'}^{(4a-2)} &= \frac{\pi n_i^2 V_0^4}{\hbar}\int[d\mathbf{k}'']\left\{\left[\frac{\tilde{\Xi}_{\varphi\varphi'}^{++}\Xi_{\varphi\varphi'}^{+\eta}\Xi_{\varphi'\varphi''}^{\eta\eta'}\Xi_{\varphi''\varphi'}^{\eta'+}}{(\varepsilon_{\mathbf{k}'}^{+}-\varepsilon_{\mathbf{k}'}^{\eta}+i\delta)(\varepsilon_{\mathbf{k}'}^{+}-\varepsilon_{\mathbf{k}''}^{\eta'}+i\delta)}+c.c.\right]\right. \\
&\quad\left.-\left[\frac{\tilde{\Xi}_{\varphi'\varphi}^{++}\Xi_{\varphi'\varphi}^{+\eta}\Xi_{\varphi\varphi''}^{\eta\eta'}\Xi_{\varphi''\varphi}^{\eta'+}}{(\varepsilon_{\mathbf{k}'}^{+}-\varepsilon_{\mathbf{k}}^{\eta}+i\delta)(\varepsilon_{\mathbf{k}'}^{+}-\varepsilon_{\mathbf{k}''}^{\eta'}+i\delta)}+c.c.\right]\right\}\delta(\varepsilon_{\mathbf{k}}^{+}-\varepsilon_{\mathbf{k}'}^{+}), \\
\varpi_{\mathbf{k}\mathbf{k}'}^{(4a-3)} &= \frac{\pi n_i^2 V_0^4}{\hbar}\int[d\mathbf{k}'']\left\{\left[\frac{\tilde{\Xi}_{\varphi\varphi'}^{++}\Xi_{\varphi\varphi'}^{\eta'+}\Xi_{\varphi\varphi''}^{+\eta}\Xi_{\varphi''\varphi}^{\eta\eta'}}{(\varepsilon_{\mathbf{k}'}^{+}-\varepsilon_{\mathbf{k}''}^{\eta}+i\delta)(\varepsilon_{\mathbf{k}'}^{+}-\varepsilon_{\mathbf{k}}^{\eta'}+i\delta)}+c.c.\right]\right. \\
&\quad\left.-\left[\frac{\tilde{\Xi}_{\varphi'\varphi}^{++}\Xi_{\varphi'\varphi}^{\eta'+}\Xi_{\varphi'\varphi''}^{+\eta}\Xi_{\varphi''\varphi'}^{\eta\eta'}}{(\varepsilon_{\mathbf{k}'}^{+}-\varepsilon_{\mathbf{k}''}^{\eta}+i\delta)(\varepsilon_{\mathbf{k}'}^{+}-\varepsilon_{\mathbf{k}'}^{\eta'}+i\delta)}+c.c.\right]\right\}\delta(\varepsilon_{\mathbf{k}}^{+}-\varepsilon_{\mathbf{k}'}^{+}).
\end{aligned}
\tag{S147}
$$

The last two contributions can be rewritten within a more compact style as

$$
\begin{aligned}
\varpi_{\mathbf{k}\mathbf{k}'}^{(4a-2)} &= \frac{\pi n_i^2 V_0^4}{\hbar}\int[d\mathbf{k}'']\mathrm{Re}\left[\frac{\tilde{\Xi}_{\varphi\varphi'}^{++}\Xi_{\varphi\varphi'}^{+\eta}\Xi_{\varphi'\varphi''}^{\eta\eta'}\Xi_{\varphi''\varphi'}^{\eta'+}-\tilde{\Xi}_{\varphi'\varphi}^{++}\Xi_{\varphi'\varphi}^{+\eta}\Xi_{\varphi\varphi''}^{\eta\eta'}\Xi_{\varphi''\varphi}^{\eta'+}}{(\varepsilon_{\mathbf{k}'}^{+}-\varepsilon_{\mathbf{k}'}^{\eta}+i\delta)(\varepsilon_{\mathbf{k}'}^{+}-\varepsilon_{\mathbf{k}''}^{\eta'}+i\delta)}\right]\delta(\varepsilon_{\mathbf{k}}^{+}-\varepsilon_{\mathbf{k}'}^{+}), \\
\varpi_{\mathbf{k}\mathbf{k}'}^{(4a-3)} &= \frac{\pi n_i^2 V_0^4}{\hbar}\int[d\mathbf{k}'']\mathrm{Re}\left[\frac{\tilde{\Xi}_{\varphi\varphi'}^{++}\Xi_{\varphi\varphi'}^{\eta'+}\Xi_{\varphi\varphi''}^{+\eta}\Xi_{\varphi''\varphi}^{\eta\eta'}-\tilde{\Xi}_{\varphi'\varphi}^{++}\Xi_{\varphi'\varphi}^{\eta'+}\Xi_{\varphi'\varphi''}^{+\eta}\Xi_{\varphi''\varphi'}^{\eta\eta'}}{(\varepsilon_{\mathbf{k}'}^{+}-\varepsilon_{\mathbf{k}''}^{\eta}+i\delta)(\varepsilon_{\mathbf{k}'}^{+}-\varepsilon_{\mathbf{k}}^{\eta'}+i\delta)}\right]\delta(\varepsilon_{\mathbf{k}}^{+}-\varepsilon_{\mathbf{k}'}^{+}).
\end{aligned}
\tag{S148}
$$

The numerators of these three contributions read

$$
\begin{aligned}
\mathrm{Nu1} \equiv & \tilde{\Xi}^{+\eta}_{\varphi\varphi''}\Xi^{+\eta''}_{\varphi\varphi''}\Xi^{\eta''+}_{\varphi''\varphi''}\tilde{\Xi}^{\eta+}_{\varphi''\varphi''} - \tilde{\Xi}^{+\eta}_{\varphi''\varphi''}\Xi^{+\eta''}_{\varphi''\varphi''}\Xi^{\eta''+}_{\varphi''\varphi}\tilde{\Xi}^{\eta+}_{\varphi''\varphi} \\
= & i2^{-2}(-1)^{\left(\eta+\eta''\right)/2}\left(\eta-\eta''\right)\left[\sin\theta\sin\theta'\cos\theta''\sin\left(\phi'-\phi\right)+\sin\theta'\sin\theta''\cos\theta\sin\left(\phi''-\phi'\right)\right. \\
& \left.+\sin\theta\sin\theta''\cos\theta'\sin\left(\phi-\phi''\right)\right], \\
\mathrm{Nu2} \equiv & \tilde{\Xi}^{++}_{\varphi\varphi''}\Xi^{+\eta}_{\varphi\varphi''}\Xi^{\eta\Xi''}_{\varphi''\varphi''}\Xi^{\eta''+}_{\varphi''\varphi''} - \tilde{\Xi}^{++}_{\varphi''\varphi}\Xi^{\eta+}_{\varphi''\varphi}\Xi^{+\eta''}_{\varphi''\varphi''}\Xi^{\eta''\eta}_{\varphi''\varphi''} \\
= & i2^{-2}(-1)^{\left(\eta+\eta''\right)/2}(\eta-1)\left[\sin\theta\sin\theta'\cos\theta''\sin\left(\phi'-\phi\right)+\sin\theta'\sin\theta''\cos\theta\sin\left(\phi''-\phi'\right)\right. \\
& \left.+\sin\theta\sin\theta''\cos\theta'\sin\left(\phi-\phi''\right)\right], \\
\mathrm{Nu3} \equiv & \tilde{\Xi}^{++}_{\varphi\varphi''}\Xi^{\eta''+}_{\varphi\varphi''}\Xi^{+\eta}_{\varphi\varphi''}\Xi^{\eta\eta''}_{\varphi''\varphi} - \tilde{\Xi}^{++}_{\varphi''\varphi}\Xi^{+\eta''}_{\varphi''\varphi}\Xi^{\eta''\eta}_{\varphi\varphi''}\Xi^{\eta+}_{\varphi''\varphi} \\
= & i2^{-2}(-1)^{\left(\eta+\eta''\right)/2}\left(\eta''-1\right)\left[\sin\theta\sin\theta'\cos\theta''\sin\left(\phi'-\phi\right)+\sin\theta'\sin\theta''\cos\theta\sin\left(\phi''-\phi'\right)\right. \\
& \left.+\sin\theta\sin\theta''\cos\theta'\sin\left(\phi-\phi''\right)\right].
\end{aligned}
\tag{S149}
$$

Note that the numerators are pure imaginary. For Nu1, only $\eta \neq \eta'$ can give nonzero value. The other part of integrand in $\varpi^{(4a-1)}_{\mathbf{k}\mathbf{k}'}$ is

$$
\begin{aligned}
\frac{1}{(\varepsilon^+_{\mathbf{k}'}-\varepsilon^{\eta}_{\mathbf{k}''}-i\delta)(\varepsilon^+_{\mathbf{k}'}-\varepsilon^{\eta'}_{\mathbf{k}''}+i\delta)} &= \frac{1}{(\varepsilon^+_{\mathbf{k}'}-\varepsilon^{\eta}_{\mathbf{k}''})(\varepsilon^+_{\mathbf{k}'}-\varepsilon^{\eta'}_{\mathbf{k}''})-i(\varepsilon^{\eta}_{\mathbf{k}'}-\varepsilon^{\eta'}_{\mathbf{k}''})\delta} \\
&= \frac{1}{(\varepsilon^+_{\mathbf{k}'}-\varepsilon^{+}_{\mathbf{k}''})(\varepsilon^+_{\mathbf{k}'}-\varepsilon^{-}_{\mathbf{k}''})-i\delta} \\
&= \mathcal{P}\left[\frac{1}{(\varepsilon^+_{\mathbf{k}'}-\varepsilon^{+}_{\mathbf{k}''})(\varepsilon^+_{\mathbf{k}'}-\varepsilon^{-}_{\mathbf{k}''})}\right] + i\pi\delta[(\varepsilon^+_{\mathbf{k}'}-\varepsilon^{+}_{\mathbf{k}''})(\varepsilon^+_{\mathbf{k}'}-\varepsilon^{-}_{\mathbf{k}''})] \\
&= \mathcal{P}\left[\frac{1}{(\varepsilon^+_{\mathbf{k}'}-\varepsilon^{+}_{\mathbf{k}''})(\varepsilon^+_{\mathbf{k}'}-\varepsilon^{-}_{\mathbf{k}''})}\right] + \frac{i\pi}{\varepsilon^+_{\mathbf{k}''}-\varepsilon^-_{\mathbf{k}''}}\delta(\varepsilon^+_{\mathbf{k}'}-\varepsilon^{+}_{\mathbf{k}''}) - \frac{i\pi}{\varepsilon^+_{\mathbf{k}''}-\varepsilon^-_{\mathbf{k}''}}\delta(\varepsilon^+_{\mathbf{k}'}-\varepsilon^{-}_{\mathbf{k}''}),
\end{aligned}
\tag{S150}
$$

where we have assumed $\eta = +, \eta' = -$ for the first case. For the second case $\eta = -, \eta' = +$, we have

$$
\begin{aligned}
\frac{1}{(\varepsilon^+_{\mathbf{k}'}-\varepsilon^{\eta}_{\mathbf{k}''}-i\delta)(\varepsilon^+_{\mathbf{k}'}-\varepsilon^{\eta'}_{\mathbf{k}''}+i\delta)} &= \frac{1}{(\varepsilon^+_{\mathbf{k}'}-\varepsilon^{\eta}_{\mathbf{k}''})(\varepsilon^+_{\mathbf{k}'}-\varepsilon^{\eta'}_{\mathbf{k}''})-i(\varepsilon^{\eta}_{\mathbf{k}'}-\varepsilon^{\eta'}_{\mathbf{k}''})\delta} \\
&= \frac{1}{(\varepsilon^+_{\mathbf{k}'}-\varepsilon^{-}_{\mathbf{k}''})(\varepsilon^+_{\mathbf{k}'}-\varepsilon^{+}_{\mathbf{k}''})+i\delta} \\
&= \mathcal{P}\left[\frac{1}{(\varepsilon^+_{\mathbf{k}'}-\varepsilon^{-}_{\mathbf{k}''})(\varepsilon^+_{\mathbf{k}'}-\varepsilon^{+}_{\mathbf{k}''})}\right] - i\pi\delta[(\varepsilon^+_{\mathbf{k}'}-\varepsilon^{-}_{\mathbf{k}''})(\varepsilon^+_{\mathbf{k}'}-\varepsilon^{+}_{\mathbf{k}''})] \\
&= \mathcal{P}\left[\frac{1}{(\varepsilon^+_{\mathbf{k}'}-\varepsilon^{-}_{\mathbf{k}''})(\varepsilon^+_{\mathbf{k}'}-\varepsilon^{+}_{\mathbf{k}''})}\right] + \frac{i\pi}{\varepsilon^+_{\mathbf{k}''}-\varepsilon^-_{\mathbf{k}''}}\delta(\varepsilon^+_{\mathbf{k}'}-\varepsilon^{-}_{\mathbf{k}''}) - \frac{i\pi}{\varepsilon^+_{\mathbf{k}''}-\varepsilon^-_{\mathbf{k}''}}\delta(\varepsilon^+_{\mathbf{k}'}-\varepsilon^{+}_{\mathbf{k}''}).
\end{aligned}
\tag{S151}
$$

For the non-degenerate case, we have $\delta(\varepsilon^+_{\mathbf{k}'}-\varepsilon^-_{\mathbf{k}''}) = 0$. Since the principal part is pure real, the real part of $\varpi^{(4a-1)}_{\mathbf{k}\mathbf{k}'}$ is

$$
\begin{aligned}
\varpi^{(4a-1)}_{\mathbf{k}\mathbf{k}'} = & \frac{\pi^2 n_i^2 V_0^4}{\hbar}\int[d\mathbf{k}'']\frac{1}{\varepsilon^+_{\mathbf{k}''}-\varepsilon^-_{\mathbf{k}''}}\left[\sin\theta\sin\theta'\cos\theta''\sin\left(\phi-\phi'\right)+\sin\theta'\sin\theta''\cos\theta\sin\left(\phi'-\phi''\right)\right. \\
& \left.+\sin\theta\sin\theta''\cos\theta'\sin\left(\phi''-\phi\right)\right]\delta(\varepsilon^+_{\mathbf{k}'}-\varepsilon^+_{\mathbf{k}''})\delta(\varepsilon^+_{\mathbf{k}}-\varepsilon^+_{\mathbf{k}'}).
\end{aligned}
\tag{S152}
$$

Following the similar process, we have

$$
\begin{aligned}
\varpi^{(4a-2)}_{\mathbf{k}\mathbf{k}'} = & \frac{\pi^2 n_i^2 V_0^4}{\hbar}\int[d\mathbf{k}'']\frac{1}{\varepsilon^+_{\mathbf{k}'}-\varepsilon^-_{\mathbf{k}'}}\left[\sin\theta\sin\theta'\cos\theta''\sin\left(\phi-\phi'\right)+\sin\theta'\sin\theta''\cos\theta\sin\left(\phi'-\phi''\right)\right. \\
& \left.+\sin\theta\sin\theta''\cos\theta'\sin\left(\phi''-\phi\right)\right]\delta(\varepsilon^+_{\mathbf{k}'}-\varepsilon^+_{\mathbf{k}''})\delta(\varepsilon^+_{\mathbf{k}}-\varepsilon^+_{\mathbf{k}'}), \\
\varpi^{(4a-3)}_{\mathbf{k}\mathbf{k}'} = & \frac{\pi^2 n_i^2 V_0^4}{\hbar}\int[d\mathbf{k}'']\frac{1}{\varepsilon^+_{\mathbf{k}}-\varepsilon^-_{\mathbf{k}}}\left[\sin\theta\sin\theta'\cos\theta''\sin\left(\phi-\phi'\right)+\sin\theta'\sin\theta''\cos\theta\sin\left(\phi'-\phi''\right)\right. \\
& \left.+\sin\theta\sin\theta''\cos\theta'\sin\left(\phi''-\phi\right)\right]\delta(\varepsilon^+_{\mathbf{k}'}-\varepsilon^+_{\mathbf{k}''})\delta(\varepsilon^+_{\mathbf{k}}-\varepsilon^+_{\mathbf{k}'}).
\end{aligned}
\tag{S153}
$$

Thus, the antisymmetric fourth-order scattering rate within the noncrossing approximation reads

$$\varpi_{\mathbf{kk}'}^{(4a)} = \frac{\pi^2 n_i^2 V_0^4}{\hbar} \int [d\mathbf{k}''] \left( \frac{1}{\varepsilon_{\mathbf{k}}^+ - \varepsilon_{\mathbf{k}}^-} + \frac{1}{\varepsilon_{\mathbf{k}'}^+ - \varepsilon_{\mathbf{k}'}^-} + \frac{1}{\varepsilon_{\mathbf{k}''}^+ - \varepsilon_{\mathbf{k}''}^-} \right) [\sin\theta \sin\theta' \cos\theta'' \sin(\phi - \phi') \\ + \sin\theta' \sin\theta'' \cos\theta \sin(\phi' - \phi'') + \sin\theta \sin\theta'' \cos\theta' \sin(\phi'' - \phi)]\, \delta(\varepsilon_{\mathbf{k}'}^+ - \varepsilon_{\mathbf{k}''}^+) \delta(\varepsilon_{\mathbf{k}}^+ - \varepsilon_{\mathbf{k}'}^+). \tag{S154}$$

### C. Coordinate shift

Assume that the Fermi energy lies in the upper band, the coordinate shift of the 2D Dirac model with a $\delta$-correlated spin independent random potential is given by

$$\delta \mathbf{r}_{\mathbf{kk}'} = \langle u_{\mathbf{k}}^+ | i\partial_{\mathbf{k}} u_{\mathbf{k}}^+ \rangle - \langle u_{\mathbf{k}'}^+ | i\partial_{\mathbf{k}'} u_{\mathbf{k}'}^+ \rangle - (\partial_{\mathbf{k}} + \partial_{\mathbf{k}'}) \arg\langle u_{\mathbf{k}}^+ | u_{\mathbf{k}'}^+ \rangle, \tag{S155}$$

In components, we have

$$\begin{aligned} \langle u_{\mathbf{k}}^+ | \partial_k u_{\mathbf{k}}^+ \rangle &= \begin{bmatrix} \cos\frac{\theta}{2} \\ \sin\frac{\theta}{2} e^{i\phi} \end{bmatrix}^\dagger \partial_k \begin{bmatrix} \cos\frac{\theta}{2} \\ \sin\frac{\theta}{2} e^{i\phi} \end{bmatrix} = \begin{bmatrix} \cos\frac{\theta}{2} \\ \sin\frac{\theta}{2} e^{i\phi} \end{bmatrix}^\dagger \begin{bmatrix} -\frac{1}{2}\partial_k\theta \sin\frac{\theta}{2} \\ \frac{1}{2}\partial_k\theta \cos\frac{\theta}{2} e^{i\phi} \end{bmatrix} = 0, \\ \langle u_{\mathbf{k}}^+ | \partial_\phi u_{\mathbf{k}}^+ \rangle &= \begin{bmatrix} \cos\frac{\theta}{2} \\ \sin\frac{\theta}{2} e^{i\phi} \end{bmatrix}^\dagger \partial_\phi \begin{bmatrix} \cos\frac{\theta}{2} \\ \sin\frac{\theta}{2} e^{i\phi} \end{bmatrix} = i\frac{1-\cos\theta}{2}, \end{aligned} \tag{S156}$$

thus we obtain that

$$\begin{aligned} i\langle u_{\mathbf{k}}^+ | \partial_{k_x} u_{\mathbf{k}}^+ \rangle &= i\cos\phi \langle u_{\mathbf{k}}^+ | \partial_k u_{\mathbf{k}}^+ \rangle - i\frac{\sin\phi}{k} \langle u_{\mathbf{k}}^+ | \partial_\phi u_{\mathbf{k}}^+ \rangle = \frac{1-\cos\theta}{2k} \sin\phi, \\ i\langle u_{\mathbf{k}}^+ | \partial_{k_y} u_{\mathbf{k}}^+ \rangle &= i\sin\phi \langle u_{\mathbf{k}}^+ | \partial_k u_{\mathbf{k}}^+ \rangle + i\frac{\cos\phi}{k} \langle u_{\mathbf{k}}^+ | \partial_\phi u_{\mathbf{k}}^+ \rangle = \frac{\cos\theta - 1}{2k} \cos\phi, \end{aligned} \tag{S157}$$

where we have used

$$\begin{aligned} \partial_{k_x} &= \cos\phi \partial_k - \frac{\sin\phi}{k} \partial_\phi, \\ \partial_{k_y} &= \sin\phi \partial_k + \frac{\cos\phi}{k} \partial_\phi. \end{aligned} \tag{S158}$$

For the last term, by using the definition of complex number $z = |z| e^{i\arg(z)}$, we have

$$\arg\langle u_{\mathbf{k}}^+ | u_{\mathbf{k}'}^+ \rangle = -i \ln \frac{\langle u_{\mathbf{k}}^+ | u_{\mathbf{k}'}^+ \rangle}{|\langle u_{\mathbf{k}}^+ | u_{\mathbf{k}'}^+ \rangle|}, \tag{S159}$$

with

$$\begin{aligned} \langle u_{\mathbf{k}}^+ | u_{\mathbf{k}'}^+ \rangle &= \cos\frac{\theta}{2} \cos\frac{\theta'}{2} + \sin\frac{\theta}{2} \sin\frac{\theta'}{2} e^{i(\phi' - \phi)}, \\ |\langle u_{\mathbf{k}}^+ | u_{\mathbf{k}'}^+ \rangle|^2 &= \frac{1}{2} \left[ 1 + \cos\theta \cos\theta' + \sin\theta \sin\theta' \cos(\phi' - \phi) \right]. \end{aligned} \tag{S160}$$

The components of the partial derivative read

$$\begin{aligned} \partial_{k_x} \arg(z) &= \cos\phi \partial_k \arg(z) - \frac{\sin\phi}{k} \partial_\phi \arg(z), \\ \partial_{k_y} \arg(z) &= \sin\phi \partial_k \arg(z) + \frac{\cos\phi}{k} \partial_\phi \arg(z), \end{aligned} \tag{S161}$$

with $z \equiv \langle u_{\mathbf{k}}^+ | u_{\mathbf{k}'}^+ \rangle$. Note that for a general complex function $z(x)$, we have

$$\begin{aligned} \partial_x \arg(z) &= \partial_x \left( -i \ln \frac{z}{|z|} \right) \\ &= -i \frac{|z|}{z} \frac{|z| \partial_x z - z \partial_x |z|}{|z|^2} \\ &= \frac{-i}{|z|^2} \left( \frac{z^2}{z} \partial_x z - |z| \partial_x |z| \right) \\ &= \frac{-i}{|z|^2} \left( z^* \partial_x z - \frac{1}{2} \partial_x |z|^2 \right), \end{aligned} \tag{S162}$$

thus we can obtain

$$
\begin{aligned}
\partial_k \arg(z) &= \frac{1}{4|z|^2}\frac{\sin\theta\cos\theta}{k}\sin\theta'\sin(\phi'-\phi),\\
\partial_{k'} \arg(z) &= \frac{1}{4|z|^2}\frac{\sin\theta'\cos\theta'}{k'}\sin\theta\sin(\phi'-\phi),\\
\partial_{\phi} \arg(z) &= \frac{-1}{4|z|^2}\left[\sin\theta\sin\theta'\cos\left(\phi'-\phi\right)+\left(1-\cos\theta\right)\left(1-\cos\theta'\right)\right],\\
\partial_{\phi'} \arg(z) &= \frac{1}{4|z|^2}\left[\sin\theta\sin\theta'\cos\left(\phi'-\phi\right)+\left(1-\cos\theta\right)\left(1-\cos\theta'\right)\right],
\end{aligned}
\tag{S163}
$$

where we have used

$$
\partial_k\theta = \frac{\sin\theta\cos\theta}{k}. \tag{S164}
$$

Their combination gives

$$
\begin{aligned}
\partial_{k_x}\arg(z) &= \cos\phi\partial_k\arg(z) - \frac{\sin\phi}{k}\partial_\phi\arg(z)\\
&= \frac{1}{4k|z|^2}\left[\sin\theta\cos\theta\sin\theta'\sin\left(\phi'-\phi\right)\cos\phi+\sin\theta\sin\theta'\cos\left(\phi'-\phi\right)\sin\phi+\left(1-\cos\theta\right)\left(1-\cos\theta'\right)\sin\phi\right],\\
\partial_{k'_x}\arg(z) &= \cos\phi'\partial_{k'}\arg(z) - \frac{\sin\phi'}{k'}\partial_{\phi'}\arg(z)\\
&= \frac{1}{4k'|z|^2}\left[\sin\theta'\cos\theta'\sin\theta\sin\left(\phi'-\phi\right)\cos\phi'-\sin\theta\sin\theta'\cos\left(\phi'-\phi\right)\sin\phi'-\left(1-\cos\theta\right)\left(1-\cos\theta'\right)\sin\phi'\right],\\
\partial_{k_y}\arg(z) &= \sin\phi\partial_k\arg(z) + \frac{\cos\phi}{k}\partial_\phi\arg(z)\\
&= \frac{1}{4k|z|^2}\left[\sin\theta\cos\theta\sin\theta'\sin\left(\phi'-\phi\right)\sin\phi-\sin\theta\sin\theta'\cos\left(\phi'-\phi\right)\cos\phi-\left(1-\cos\theta\right)\left(1-\cos\theta'\right)\cos\phi\right],\\
\partial_{k'_y}\arg(z) &= \sin\phi'\partial_{k'}\arg(z) + \frac{\cos\phi'}{k'}\partial_{\phi'}\arg(z)\\
&= \frac{1}{4k'|z|^2}\left[\sin\theta'\cos\theta'\sin\theta\sin\left(\phi'-\phi\right)\sin\phi'+\sin\theta\sin\theta'\cos\left(\phi'-\phi\right)\cos\phi'+\left(1-\cos\theta\right)\left(1-\cos\theta'\right)\cos\phi'\right].
\end{aligned}
\tag{S165}
$$

Then the contributions read

$$
\begin{aligned}
\langle u^+_{\mathbf{k}}|i\partial_{k_x}u^+_{\mathbf{k}}\rangle - \partial_{k_x}\arg(z) &= \frac{\sin\theta}{4k|z|^2}(\sin\theta\cos\theta'\sin\phi-\cos\theta\sin\theta'\sin\phi'),\\
-\langle u^+_{\mathbf{k}'}|i\partial_{k'_x}u^+_{\mathbf{k}'}\rangle - \partial_{k'_x}\arg(z) &= \frac{\sin\theta'}{4k'|z|^2}(\sin\theta\cos\theta'\sin\phi-\cos\theta\sin\theta'\sin\phi'),\\
\langle u^+_{\mathbf{k}}|i\partial_{k_y}u^+_{\mathbf{k}}\rangle - \partial_{k_y}\arg(z) &= \frac{\sin\theta}{4k|z|^2}(\cos\theta\sin\theta'\cos\phi'-\sin\theta\cos\theta'\cos\phi),\\
-\langle u^+_{\mathbf{k}'}|i\partial_{k'_y}u^+_{\mathbf{k}'}\rangle - \partial_{k'_y}\arg(z) &= \frac{\sin\theta'}{4k'|z|^2}(\cos\theta\sin\theta'\cos\phi'-\sin\theta\cos\theta'\cos\phi).
\end{aligned}
\tag{S166}
$$

Consequently, the coordinate shift for a weak impurity potential $V_{imp}$ can be written in components as

$$
\begin{aligned}
\delta r^x_{\mathbf{k}\mathbf{k}'} &= \langle u^+_{\mathbf{k}}|i\partial_{k_x}u^+_{\mathbf{k}}\rangle - \langle u^+_{\mathbf{k}'}|i\partial_{k'_x}u^+_{\mathbf{k}'}\rangle - (\partial_{k_x}+\partial_{k'_x})\arg\langle u^+_{\mathbf{k}}|u^+_{\mathbf{k}'}\rangle\\
&= \frac{1}{4|z|^2}\left(\frac{\sin\theta}{k}+\frac{\sin\theta'}{k'}\right)(\sin\theta\cos\theta'\sin\phi-\cos\theta\sin\theta'\sin\phi')\\
&= -\frac{1}{2|z|^2}\left(\frac{\varepsilon_{\mathbf{k}}}{\varepsilon'_{\mathbf{k}}}\Omega^+_{\mathbf{k}}+\frac{\varepsilon_{\mathbf{k}'}}{\varepsilon_{\mathbf{k}}}\Omega^+_{\mathbf{k}'}\right)\left(k_y-k'_y\right),
\end{aligned}
\tag{S167}
$$

and similarly,

$$\begin{aligned}\delta r^{y}_{\mathbf{k}\mathbf{k}'} &= \langle u^{+}_{\mathbf{k}}|i\partial_{k_y} u^{+}_{\mathbf{k}}\rangle - \langle u^{+}_{\mathbf{k}'}|i\partial_{k'_y} u^{+}_{\mathbf{k}'}\rangle - (\partial_{k_y} + \partial_{k'_y}) \arg\langle u^{+}_{\mathbf{k}}|u^{+}_{\mathbf{k}'}\rangle \\ &= \frac{1}{4|z|^2}\left(\frac{\sin\theta}{k} + \frac{\sin\theta'}{k'}\right)(\cos\theta\sin\theta'\cos\phi' - \sin\theta\cos\theta'\cos\phi) \\ &= \frac{1}{2|z|^2}\left(\frac{\varepsilon_{\mathbf{k}}}{\varepsilon'_{\mathbf{k}}}\Omega^{+}_{\mathbf{k}} + \frac{\varepsilon_{\mathbf{k}'}}{\varepsilon_{\mathbf{k}}}\Omega^{+}_{\mathbf{k}'}\right)(k_x - k'_x)\,.\end{aligned} \tag{S168}$$

Thus, we can formally write the coordinate shift for the upper band as

$$\delta\mathbf{r}_{\mathbf{k}\mathbf{k}'} = \frac{1}{2}\left(\frac{\varepsilon_{\mathbf{k}}}{\varepsilon_{\mathbf{k}'}}\Omega^{+}_{\mathbf{k}} + \frac{\varepsilon_{\mathbf{k}'}}{\varepsilon_{\mathbf{k}}}\Omega^{+}_{\mathbf{k}'}\right) \times \frac{(\mathbf{k}-\mathbf{k}')}{|\langle u^{+}_{\mathbf{k}}|u^{+}_{\mathbf{k}'}\rangle|^2}, \tag{S169}$$

it has the property $\delta\mathbf{r}_{\mathbf{k}\mathbf{k}'} = -\delta\mathbf{r}_{\mathbf{k}'\mathbf{k}}$.

## SVI. 2D MASSIVE DIRAC MODEL

### A. Eigen solutions

As a minimal model, we consider a 2D massive Dirac fermion

$$\hat{\mathcal{H}}_0(\mathbf{k}) = v(k_x\sigma_x + vk_y\sigma_y) + m\sigma_z. \tag{S170}$$

The band dispersion reads

$$\varepsilon^{\pm}_{\mathbf{k}} = \pm\sqrt{v^2k^2 + m^2}, \tag{S171}$$

with $k^2 \equiv k_x^2 + k_y^2$. The chiral basis vectors that diagonalize the Hamiltonian are

$$\psi^{\pm}_{\mathbf{k}} = \frac{e^{i\mathbf{k}\cdot\mathbf{r}}}{\sqrt{\mathcal{V}}}|u^{\pm}_{\mathbf{k}}\rangle, \tag{S172}$$

where $\mathcal{V}$ refers to the general volume and

$$|u^{+}_{\mathbf{k}}\rangle = \begin{bmatrix}\cos\frac{\theta}{2} \\ \sin\frac{\theta}{2}e^{i\phi}\end{bmatrix}, \qquad |u^{-}_{\mathbf{k}}\rangle = \begin{bmatrix}\sin\frac{\theta}{2} \\ -\cos\frac{\theta}{2}e^{i\phi}\end{bmatrix} \tag{S173}$$

are the eigenstates with

$$\cos\theta = \frac{m}{\sqrt{v^2k^2+m^2}}, \qquad \tan\phi = \frac{k_y}{k_x}. \tag{S174}$$

Note that $\tan\phi = k_y/k_x$ indicting that $k_y = k\sin\phi$ and $k_x = k\cos\phi$. The velocity along the two axes are

$$v^{x}_{\mathbf{k},\pm} = \pm\frac{1}{\hbar}\frac{v^2k_x}{\sqrt{v^2k^2+m^2}}, \qquad v^{y}_{\mathbf{k},\pm} = \pm\frac{1}{\hbar}\frac{v^2k_y}{\sqrt{v^2k^2+m^2}}. \tag{S175}$$

The Berry curvature for each band is

$$\Omega^{\pm}_{\mathbf{k}} = \mp\frac{mv^2}{2(v^2k^2+m^2)^{3/2}}. \tag{S176}$$

### B. Anomalous electric Hall conductivity

We consider the anomalous electric Hall conductivity in the absence of time reversal symmetry. The system is isotropic with the constant relaxation time. We only consider the upper band

$$\mathcal{I}^{in}_{el}\{f_{\mathbf{k}}\} = -\frac{f^{in}_{\mathbf{k}} - f^{0}_{\mathbf{k}}}{\tau}, \tag{S177}$$

$$\mathcal{I}_{el}^{in}\{f_{\mathbf{k}}\} = -\sum_{\mathbf{k}'} \varpi_{\mathbf{k}\mathbf{k}'}^{(2)}(f_{\mathbf{k}} - f_{\mathbf{k}'}), \tag{S178}$$

thus,

$$\begin{aligned} \frac{f_{\mathbf{k}}^{in} - f_{\mathbf{k}}^{0}}{\tau} &= \sum_{\mathbf{k}'} \varpi_{\mathbf{k}\mathbf{k}'}^{(2)}(f_{\mathbf{k}} - f_{\mathbf{k}'}) \\ \Rightarrow \quad \frac{f_{\mathbf{k}}}{\tau} &= \sum_{\mathbf{k}'} \varpi_{\mathbf{k}\mathbf{k}'}^{(2)}(f_{\mathbf{k}} - f_{\mathbf{k}'}), \\ \Rightarrow \quad \frac{1}{\tau} &= \sum_{\mathbf{k}'} \varpi_{\mathbf{k}\mathbf{k}'}^{(2)}\left(1 - f_{\mathbf{k}'}/f_{\mathbf{k}}\right), \\ \Rightarrow \quad \frac{1}{\tau} &= \sum_{\mathbf{k}'} \varpi_{\mathbf{k}\mathbf{k}'}^{(2)}\left(1 - \cos\alpha\right), \end{aligned} \tag{S179}$$

where $\alpha$ is the angle between $\mathbf{k}$ and $\mathbf{k}'$, which is exactly $\phi - \phi'$ in this case. Now, we have

$$\begin{aligned} \frac{1}{\tau} &= \int \frac{d^2\mathbf{k}'}{(2\pi)^2} \varpi_{\mathbf{k}\mathbf{k}'}^{(2)} \left[1 - \cos(\phi - \phi')\right] \\ &= \frac{n_i V_0^2}{4\pi\hbar} \int_0^{\infty} k' dk' \int_0^{2\pi} d\phi' \left[1 + \cos\theta\cos\theta' + \sin\theta\sin\theta'\cos(\phi - \phi')\right] \left[1 - \cos(\phi - \phi')\right] \delta(\varepsilon_{\mathbf{k}}^{+} - \varepsilon_{\mathbf{k}'}^{+}) \\ &= \frac{n_i V_0^2}{4\pi\hbar} \int_0^{\infty} k' dk' \int_0^{2\pi} d\phi' \left[1 + \cos\theta\cos\theta' + \sin\theta\sin\theta'\cos(\phi - \phi')\right] \left[1 - \cos(\phi - \phi')\right] \frac{\sqrt{v^2k^2 + m^2}}{v^2 k} \delta(k - k') \\ &= \frac{n_i V_0^2}{4\hbar} \frac{\varepsilon^2 + 3m^2}{v^2 \varepsilon}, \end{aligned} \tag{S180}$$

by noting that

$$\varpi_{\mathbf{k}\mathbf{k}'}^{(2)} = \frac{\pi}{\hbar} n_i V_0^2 \left[1 + \cos\theta\cos\theta' + \sin\theta\sin\theta'\cos(\phi - \phi')\right] \delta(\varepsilon_{\mathbf{k}}^{+} - \varepsilon_{\mathbf{k}'}^{+}). \tag{S181}$$

The anomalous electric Hall conductivity in the $x$-$y$ plane reads

$$\sigma_{xy}^{tot} = \sigma_{xy}^{in} + \sigma_{xy}^{sj,1} + \sigma_{xy}^{sj,2} + \sigma_{xy}^{sk}, \tag{S182}$$

with

$$\begin{aligned} \sigma_{xy}^{in} &= -\frac{e^2}{\hbar} \sum_{l} \Omega_l^z f_l^0, \\ \sigma_{xy}^{sj,1} &= -\frac{e^2}{\hbar} \tau \int [d\mathbf{k}] v_x^{sj} \partial_{\mathbf{k}}^{y} f_{\mathbf{k}}^{0}, \\ \sigma_{xy}^{sj,2} &= \frac{e^2}{\hbar} \tau \int [d\mathbf{k}] v_y^{sj} \partial_{\mathbf{k}}^{x} f_{\mathbf{k}}^{0}, \\ \sigma_{xy}^{sk} &= -\frac{e^2}{\hbar} \tau^2 \int [d\mathbf{k}] \int [d\mathbf{k}'] \varpi_{\mathbf{k}\mathbf{k}'}^{as} (v_{\mathbf{k}}^{x} - v_{\mathbf{k}'}^{x}) \partial_{\mathbf{k}}^{y} f_{\mathbf{k}}^{0}. \end{aligned} \tag{S183}$$

The index $l$ in $\sigma_{xy}^{in}$ indicates that the intrinsic contribution needs the summation over all the filled bands. We assume that the Fermi energy is in the upper band, thus the band index can be neglected in the side-jump and skew-scattering contributions.

### 1. Intrinsic contribution

Since the intrinsic contribution comes from the whole Fermi sea, both the totally filled negative energy and the partially filled positive energy bands contribute to it.

$$\begin{aligned}
\sigma_{xy}^{in} &= -\frac{e^2}{\hbar}\sum_l \Omega_l^z f_l^0 \\
&= -\frac{e^2}{\hbar}\int \frac{d^2\mathbf{k}}{(2\pi)^2} f^0(\varepsilon_{\mathbf{k}}^-)\Omega_{\mathbf{k}}^- - \frac{e^2}{\hbar}\int \frac{d^2\mathbf{k}}{(2\pi)^2} f^0(\varepsilon_{\mathbf{k}}^+)\Omega_{\mathbf{k}}^+ \\
&= -\frac{e^2}{\hbar}\frac{1}{(2\pi)^2}\int_0^\infty kdk\int_0^{2\pi} d\phi\Omega_{\mathbf{k}}^- - \frac{e^2}{\hbar}\frac{1}{(2\pi)^2}\int_0^{k_f} kdk\int_0^{2\pi} d\phi\Omega_{\mathbf{k}}^+ \\
&= -\frac{e^2}{\hbar}\frac{1}{(2\pi)^2}\int_{k_f}^\infty kdk\int_0^{2\pi} d\phi\Omega_{\mathbf{k}}^- \\
&= -\frac{e^2}{\hbar}\frac{m}{2\varepsilon},
\end{aligned} \tag{S184}$$

where we have used $\Omega_{\mathbf{k}}^+ = -\Omega_{\mathbf{k}}^-$.

### 2. Side-jump contribution

The direct interband scattering is not energetically allowed in the weak-disorder limit of our model. We consider only the coordinate shift effect of scattering in the upper band

$$\delta\mathbf{r}_{\mathbf{k}\mathbf{k}'} = \Omega_{\mathbf{k}}^+ \frac{\hat{\mathbf{z}}\times(\mathbf{k}-\mathbf{k}')}{|\langle u_{\mathbf{k}}^+|u_{\mathbf{k}'}^+\rangle|^2}, \tag{S185}$$

and the corresponding side-jump velocity components read

$$\begin{aligned}
v_x^{sj} &= \int \frac{d^2\mathbf{k}'}{(2\pi)^2}\varpi_{\mathbf{k}\mathbf{k}'}^{(2)}\delta r_{\mathbf{k}'\mathbf{k}}^x \\
&= \frac{n_i V_0^2}{4\pi\hbar}\int_0^\infty k'dk'\int_0^{2\pi} d\phi' \left[1+\cos\theta\cos\theta'+\sin\theta\sin\theta'\cos(\phi-\phi')\right]\delta(\varepsilon_{\mathbf{k}}^+ - \varepsilon_{\mathbf{k}'}^+)\Omega_{\mathbf{k}}^+ \frac{-(k_y'-k_y)}{|\langle u_{\mathbf{k}}^+|u_{\mathbf{k}'}^+\rangle|^2} \\
&= \frac{n_i V_0^2}{4\pi\hbar}\int_0^\infty k'dk'\int_0^{2\pi} d\phi' \left[1+\cos\theta\cos\theta'+\sin\theta\sin\theta'\cos(\phi-\phi')\right]\frac{\sqrt{v^2k^2+m^2}}{v^2k}\delta(k-k') \\
&\quad\times \frac{-mv^2}{2(v^2k^2+m^2)^{3/2}}\frac{-(k'\sin\phi'-k\sin\phi)}{\frac{1}{2}\left[1+\cos\theta\cos\theta'+\sin\theta\sin\theta'\cos(\phi'-\phi)\right]} \\
&= -\frac{n_i V_0^2 m}{2\hbar\varepsilon^2}k\sin\phi,
\end{aligned} \tag{S186}$$

and

$$\begin{aligned}
v_y^{sj} &= \int \frac{d^2\mathbf{k}'}{(2\pi)^2}\varpi_{\mathbf{k}\mathbf{k}'}^{(2)}\delta r_{\mathbf{k}'\mathbf{k}}^y \\
&= \frac{n_i V_0^2}{4\pi\hbar}\int_0^\infty k'dk'\int_0^{2\pi} d\phi' \left[1+\cos\theta\cos\theta'+\sin\theta\sin\theta'\cos(\phi-\phi')\right]\delta(\varepsilon_{\mathbf{k}}^+ - \varepsilon_{\mathbf{k}'}^+)\Omega_{\mathbf{k}}^+ \frac{k_x'-k_x}{|\langle u_{\mathbf{k}}^+|u_{\mathbf{k}'}^+\rangle|^2} \\
&= \frac{n_i V_0^2}{4\pi\hbar}\int_0^\infty k'dk'\int_0^{2\pi} d\phi' \left[1+\cos\theta\cos\theta'+\sin\theta\sin\theta'\cos(\phi-\phi')\right]\frac{\sqrt{v^2k^2+m^2}}{v^2k}\delta(k-k') \\
&\quad\times \frac{-mv^2}{2(v^2k^2+m^2)^{3/2}}\frac{k'\cos\phi'-k\cos\phi}{\frac{1}{2}\left[1+\cos\theta\cos\theta'+\sin\theta\sin\theta'\cos(\phi'-\phi)\right]} \\
&= \frac{n_i V_0^2 m}{2\hbar\varepsilon^2}k\cos\phi.
\end{aligned} \tag{S187}$$

Therefore, we can obtain

$$\begin{aligned}
\sigma_{xy}^{sj,1} &= -\frac{e^2}{\hbar}\tau\int[d\mathbf{k}]v_x^{sj}\partial_{\mathbf{k}}^y f_{\mathbf{k}}^0 \\
&= e^2\tau\int\frac{d^2\mathbf{k}}{(2\pi)^2}v_x^{sj}v_{\mathbf{k}}^y\left(-\frac{\partial f_{\mathbf{k}}^0}{\partial\varepsilon_{\mathbf{k}}}\right) \\
&= \frac{e^2\tau}{4\pi^2}\int_0^\infty kdk\int_0^{2\pi}d\phi\frac{n_iV_0^2m(-k\sin\phi)}{2\hbar\varepsilon^2}\frac{v^2k\sin\phi}{\hbar\varepsilon}\delta(\varepsilon-\varepsilon_f) \\
&= -\frac{n_iV_0^2me^2\tau}{8\pi^2\hbar^2}\int dk\int_0^{2\pi}d\phi\frac{v^2k^3\sin^2\phi}{\varepsilon^3}\frac{\varepsilon}{v^2k}\delta(k-k_f) \\
&= -\frac{n_iV_0^2me^2}{8\pi^2\hbar^2}\frac{4\hbar}{n_iV_0^2}\frac{v^2\varepsilon}{\varepsilon^2+3m^2}\frac{k_f^2\pi}{\varepsilon^2} \\
&= -\frac{e^2}{h}\frac{m(\varepsilon^2-m^2)}{\varepsilon(\varepsilon^2+3m^2)},
\end{aligned} \tag{S188}$$

by noting that

$$\tau = \frac{4\hbar}{n_iV_0^2}\frac{v^2\varepsilon}{\varepsilon^2+3m^2}, \tag{S189}$$

and

$$\begin{aligned}
\sigma_{xy}^{sj,2} &= \frac{e^2}{\hbar}\tau\int[d\mathbf{k}]v_y^{sj}\partial_{\mathbf{k}}^x f_{\mathbf{k}}^0 \\
&= -e^2\tau\int\frac{d^2\mathbf{k}}{(2\pi)^2}v_y^{sj}v_{\mathbf{k}}^x\left(-\frac{\partial f_{\mathbf{k}}^0}{\partial\varepsilon_{\mathbf{k}}}\right) \\
&= -\frac{e^2\tau}{4\pi^2}\int_0^\infty kdk\int_0^{2\pi}d\phi\frac{n_iV_0^2mk\cos\phi}{2\hbar\varepsilon^2}\frac{v^2k\cos\phi}{\hbar\varepsilon}\delta(\varepsilon-\varepsilon_f) \\
&= -\frac{n_iV_0^2me^2\tau}{8\pi^2\hbar^2}\int dk\int_0^{2\pi}d\phi\frac{v^2k^3\cos^2\phi}{\varepsilon^3}\frac{\sqrt{v^2k^2+m^2}}{v^2k}\delta(k-k_f) \\
&= -\frac{n_iV_0^2me^2}{8\pi^2\hbar^2}\frac{4\hbar}{n_iV_0^2}\frac{v^2\varepsilon}{\varepsilon^2+3m^2}\frac{k_f^2\pi}{\varepsilon^2} \\
&= -\frac{e^2}{h}\frac{m(\varepsilon^2-m^2)}{\varepsilon(\varepsilon^2+3m^2)}.
\end{aligned} \tag{S190}$$

Consequently, the total side-jump scattering contribution reads

$$\sigma_{xy}^{sj} = \sigma_{xy}^{sj,1}+\sigma_{xy}^{sj,2} = -\frac{e^2}{h}\frac{2m(\varepsilon^2-m^2)}{\varepsilon(\varepsilon^2+3m^2)}. \tag{S191}$$

### *3. Skew-scattering contribution*

For our model, the third antisymmetric scattering rates in the upper band can be simplified as

$$\begin{aligned}
\varpi_{\mathbf{k}\mathbf{k}'}^{(3a)} &= \frac{\pi^2n_iV_1^3}{\hbar}\int[d\mathbf{k}'']\left[\sin\theta\sin\theta'\cos\theta''\sin(\phi-\phi')+\sin\theta'\sin\theta''\cos\theta\sin(\phi'-\phi'')\right. \\
&\quad\left.+\sin\theta\sin\theta''\cos\theta'\sin(\phi''-\phi)\right]\delta(\varepsilon_{\mathbf{k}}^+-\varepsilon_{\mathbf{k}''}^+)\delta(\varepsilon_{\mathbf{k}}^+-\varepsilon_{\mathbf{k}'}^+) \\
&= \frac{n_iV_1^3}{4\hbar}\int_0^\infty k''dk''\int_0^{2\pi}d\phi''\left[\sin\theta\sin\theta'\cos\theta''\sin(\phi-\phi')+\sin\theta'\sin\theta''\cos\theta\sin(\phi'-\phi'')\right. \\
&\quad\left.+\sin\theta\sin\theta''\cos\theta'\sin(\phi''-\phi)\right]\frac{\varepsilon}{v^2k}\delta(k-k'')\delta(\varepsilon_{\mathbf{k}}-\varepsilon_{\mathbf{k}'}) \\
&= \frac{\pi n_iV_1^3}{2\hbar}\frac{mk^2}{\varepsilon^2}\sin(\phi-\phi')\delta(\varepsilon_{\mathbf{k}}-\varepsilon_{\mathbf{k}'}),
\end{aligned} \tag{S192}$$

and the fourth-order

$$\begin{aligned}
\varpi^{(4a)}_{\mathbf{k}\mathbf{k}'} =& \frac{\pi^2 n_i^2 V_0^4}{\hbar}\int [d\mathbf{k}''] \left(\frac{1}{\varepsilon^+_{\mathbf{k}}-\varepsilon^-_{\mathbf{k}}}+\frac{1}{\varepsilon^+_{\mathbf{k}'}-\varepsilon^-_{\mathbf{k}'}}+\frac{1}{\varepsilon^+_{\mathbf{k}''}-\varepsilon^-_{\mathbf{k}''}}\right)[\sin\theta\sin\theta'\cos\theta''\sin(\phi-\phi') \\
&+\sin\theta'\sin\theta''\cos\theta\sin(\phi'-\phi'')+\sin\theta\sin\theta''\cos\theta'\sin(\phi''-\phi)]\,\delta(\varepsilon^+_{\mathbf{k}'}-\varepsilon^+_{\mathbf{k}''})\delta(\varepsilon^+_{\mathbf{k}}-\varepsilon^+_{\mathbf{k}'}). \\
=& \frac{n_i^2 V_0^4}{8\hbar m}\int_0^\infty k''dk''\int_0^{2\pi} d\phi''\,(\cos\theta+\cos\theta'+\cos\theta'')\,[\sin\theta\sin\theta'\cos\theta''\sin(\phi-\phi') \\
&+\sin\theta'\sin\theta''\cos\theta\sin(\phi'-\phi'')+\sin\theta\sin\theta''\cos\theta'\sin(\phi''-\phi)]\,\delta(\varepsilon_{\mathbf{k}'}-\varepsilon_{\mathbf{k}''})\,\delta(\varepsilon_{\mathbf{k}}-\varepsilon_{\mathbf{k}'}) \\
=& \frac{n_i^2 V_0^4}{8\hbar m}\int_0^\infty k''dk''\int_0^{2\pi} d\phi''\,(\cos\theta+\cos\theta'+\cos\theta'')\,[\sin\theta\sin\theta'\cos\theta''\sin(\phi-\phi') \\
&+\sin\theta'\sin\theta''\cos\theta\sin(\phi'-\phi'')+\sin\theta\sin\theta''\cos\theta'\sin(\phi''-\phi)]\,\frac{\varepsilon}{v^2 k}\delta(k-k'')\delta(\varepsilon_{\mathbf{k}}-\varepsilon_{\mathbf{k}'}) \\
=& \frac{3\pi n_i V_0^4}{4\hbar}\frac{mk^2}{\varepsilon^3}\sin(\phi-\phi')\delta(\varepsilon_{\mathbf{k}}-\varepsilon_{\mathbf{k}'}),
\end{aligned} \tag{S193}$$

where we have used $\varepsilon^+_{\mathbf{k}}-\varepsilon^-_{\mathbf{k}}=2\varepsilon^+_{\mathbf{k}}$ and $\cos\theta=m/\varepsilon^+_{\mathbf{k}}$, and dropped the superscript + for simplicity. Thus, the skew-scattering contribution can be divided into two parts as

$$\sigma^{sk}_{xy}=\sigma^{sk,1}_{xy}+\sigma^{sk,2}_{xy}, \tag{S194}$$

with

$$\begin{aligned}
\sigma^{sk,1}_{xy} =& -\frac{e^2}{\hbar}\tau^2\int[d\mathbf{k}]\int[d\mathbf{k}']\varpi^{(3a)}_{\mathbf{k}\mathbf{k}'}(v^x_{\mathbf{k}}-v^x_{\mathbf{k}'})\partial^y_{\mathbf{k}}f^0_{\mathbf{k}} \\
=& e^2\tau^2\int\frac{d^2\mathbf{k}}{(2\pi)^2}\int\frac{d^2\mathbf{k}'}{(2\pi)^2}\varpi^{(3a)}_{\mathbf{k}\mathbf{k}'}(v^x_{\mathbf{k}}-v^x_{\mathbf{k}'})v^y_{\mathbf{k}}\left(-\frac{\partial f^0_{\mathbf{k}}}{\partial\varepsilon_{\mathbf{k}}}\right) \\
=& \frac{n_i V_1^3 e^2\tau^2}{32\pi^3\hbar}\int_0^\infty kdk\int_0^{2\pi}d\phi\int_0^\infty k'dk'\int_0^{2\pi}d\phi'\frac{mk^2}{\varepsilon^2}\sin(\phi-\phi') \\
&\times\frac{v^4 k}{\hbar^2\varepsilon^2}\sin\phi(k\cos\phi-k'\cos\phi')\frac{\varepsilon^2}{v^4k^2}\delta(k-k')\delta(k-k_f) \\
=& \frac{n_i V_1^3 e^2}{32\pi^3\hbar}\frac{16\hbar^2}{n_i^2V_0^4}\frac{v^4\varepsilon^2}{(\varepsilon^2+3m^2)^2}\frac{-k_f^4 m\pi^2}{\hbar^2\varepsilon^2} \\
=& -\frac{e^2}{h}\frac{V_1^3}{n_iV_0^4}\frac{m(\varepsilon^2-m^2)^2}{(\varepsilon^2+3m^2)^2},
\end{aligned} \tag{S195}$$

by noting that

$$\tau^2=\frac{16\hbar^2}{n_i^2V_0^4}\frac{v^4\varepsilon^2}{(\varepsilon^2+3m^2)^2}, \tag{S196}$$

and

$$\begin{aligned}
\sigma^{sk,2}_{xy} =& -\frac{e^2}{\hbar}\tau^2\int[d\mathbf{k}]\int[d\mathbf{k}']\varpi^{(4a)}_{\mathbf{k}\mathbf{k}'}(v^x_{\mathbf{k}}-v^x_{\mathbf{k}'})\partial^y_{\mathbf{k}}f^0_{\mathbf{k}} \\
=& e^2\tau^2\int\frac{d^2\mathbf{k}}{(2\pi)^2}\int\frac{d^2\mathbf{k}'}{(2\pi)^2}\varpi^{(4a)}_{\mathbf{k}\mathbf{k}'}(v^x_{\mathbf{k}}-v^x_{\mathbf{k}'})v^y_{\mathbf{k}}\left(-\frac{\partial f^0_{\mathbf{k}}}{\partial\varepsilon_{\mathbf{k}}}\right) \\
=& \frac{3n_i^2 V_0^4 e^2\tau^2}{64\pi^3\hbar}\int_0^\infty kdk\int_0^{2\pi}d\phi\int_0^\infty k'dk'\int_0^{2\pi}d\phi'\frac{mk^2}{\varepsilon^3}\sin(\phi-\phi') \\
&\times\frac{v^4 k}{\hbar^2\varepsilon^2}\sin\phi(k\cos\phi-k'\cos\phi')\frac{\varepsilon^2}{v^4k^2}\delta(k-k')\delta(k-k_f) \\
=& \frac{3n_i^2 V_0^4 e^2\tau^2}{64\pi^3\hbar}\frac{16\hbar^2}{n_i^2V_0^4}\frac{v^4\varepsilon^2}{(\varepsilon^2+3m^2)^2}\frac{-k_f^4 m\pi^2}{\hbar^2\varepsilon^3} \\
=& -\frac{e^2}{h}\frac{3m(\varepsilon^2-m^2)^2}{2\varepsilon(\varepsilon^2+3m^2)^2}.
\end{aligned} \tag{S197}$$

Accordingly, the total skew-scattering contribution reads

$$\sigma_{xy}^{sk} = \sigma_{xy}^{sk,1} + \sigma_{xy}^{sk,2} = -\frac{e^2}{h}\frac{V_1^3}{n_i V_0^4}\frac{m(\varepsilon^2 - m^2)^2}{(\varepsilon^2 + 3m^2)^2} - \frac{e^2}{h}\frac{3m(\varepsilon^2 - m^2)^2}{2\varepsilon(\varepsilon^2 + 3m^2)^2}. \tag{S198}$$

### C. Transport coefficients

The anomalous electric Hall effect, anomalous thermoelectric Hall effect, and anomalous thermal Hall effect have similar mechanisms. One can write the anomalous electric Hall conductivities at finite temperatures as

$$\begin{aligned}
\sigma_{xy}^{in} &= -\frac{e^2}{\hbar}\int d\varepsilon \sum_l \Omega_l^z f_l^0 \left(-\frac{\partial f^0}{\partial \varepsilon}\right), \\
\sigma_{xy}^{sj,1} &= -\frac{e^2}{\hbar}\tau \int d\varepsilon \int [d\mathbf{k}] v_x^{sj} \partial_{\mathbf{k}}^y f_{\mathbf{k}}^0 \left(-\frac{\partial f^0}{\partial \varepsilon}\right), \\
\sigma_{xy}^{sj,2} &= \frac{e^2}{\hbar}\tau \int d\varepsilon \int [d\mathbf{k}] v_y^{sj} \partial_{\mathbf{k}}^x f_{\mathbf{k}}^0 \left(-\frac{\partial f^0}{\partial \varepsilon}\right), \\
\sigma_{xy}^{sk} &= -\frac{e^2}{\hbar}\tau^2 \int d\varepsilon \int [d\mathbf{k}] \int [d\mathbf{k}'] \varpi_{\mathbf{k}\mathbf{k}'}^{as} (v_{\mathbf{k}}^x - v_{\mathbf{k}'}^x) \partial_{\mathbf{k}}^y f_{\mathbf{k}}^0 \left(-\frac{\partial f^0}{\partial \varepsilon}\right).
\end{aligned} \tag{S199}$$

while the anomalous thermoelectric Hall conductivities are

$$\begin{aligned}
\alpha_{xy}^{in} &= \frac{k_B e}{\hbar}\int d\varepsilon \frac{\varepsilon - \mu}{k_B T} \sum_l \Omega_l^z f_l^0 \left(-\frac{\partial f^0}{\partial \varepsilon}\right), \\
\alpha_{xy}^{sj,1} &= \frac{k_B e}{\hbar}\tau \int d\varepsilon \frac{\varepsilon - \mu}{k_B T} \sum_l v_x^{sj} \partial_{\mathbf{k}}^y f_l^0 \left(-\frac{\partial f^0}{\partial \varepsilon}\right), \\
\alpha_{xy}^{sj,2} &= -\frac{k_B e}{\hbar}\tau \int d\varepsilon \frac{\varepsilon - \mu}{k_B T} \sum_l v_y^{sj} \partial_{\mathbf{k}}^x f_l^0 \left(-\frac{\partial f^0}{\partial \varepsilon}\right), \\
\alpha_{xy}^{sk} &= \frac{k_B e}{\hbar}\tau^2 \int d\varepsilon \frac{\varepsilon - \mu}{k_B T} \sum_{ll'} \varpi_{ll'}^{as} (v_l^x - v_{l'}^x) \partial_{\mathbf{k}}^y f_l^0 \left(-\frac{\partial f^0}{\partial \varepsilon}\right),
\end{aligned} \tag{S200}$$

and the anomalous thermal Hall conductivities

$$\begin{aligned}
\kappa_{xy}^{in} &= -\frac{k_B^2 T}{\hbar}\int d\varepsilon \left(\frac{\varepsilon - \mu}{k_B T}\right)^2 \sum_l \Omega_l^z f_l^0 \left(-\frac{\partial f^0}{\partial \varepsilon}\right), \\
\kappa_{xy}^{sj,1} &= -\frac{k_B^2 T}{\hbar}\tau \int d\varepsilon \left(\frac{\varepsilon - \mu}{k_B T}\right)^2 \sum_l v_x^{sj} \partial_{\mathbf{k}}^y f_l^0 \left(-\frac{\partial f^0}{\partial \varepsilon}\right), \\
\kappa_{xy}^{sj,2} &= \frac{k_B^2 T}{\hbar}\tau \int d\varepsilon \left(\frac{\varepsilon - \mu}{k_B T}\right)^2 \sum_l v_y^{sj} \partial_{\mathbf{k}}^x f_l^0 \left(-\frac{\partial f^0}{\partial \varepsilon}\right), \\
\kappa_{xy}^{sk} &= -\frac{k_B^2 T}{\hbar}\tau^2 \int d\varepsilon \left(\frac{\varepsilon - \mu}{k_B T}\right)^2 \sum_{ll'} \varpi_{ll'}^{as} (v_l^x - v_{l'}^x) \partial_{\mathbf{k}}^y f_l^0 \left(-\frac{\partial f^0}{\partial \varepsilon}\right).
\end{aligned} \tag{S201}$$

Thus, we can rewrite all coefficients within an organized style

$$\mathcal{C}_n^{\chi} = \int d\varepsilon [\chi] \left(\frac{\varepsilon - \mu}{k_B T}\right)^n \left(-\frac{\partial f^0}{\partial \varepsilon}\right), \tag{S202}$$

with

$$
\begin{aligned}
\chi^{in} &= 2\pi \sum_{l} \Omega_l^z f_l^0 = \frac{m}{2\varepsilon},\\
\chi^{sj} &= 2\pi\tau \int [d\mathbf{k}] v_x^{sj} \partial_{\mathbf{k}}^y f_{\mathbf{k}}^0 = \frac{2m(\varepsilon^2 - m^2)}{\varepsilon(\varepsilon^2 + 3m^2)},\\
\chi^{sk,1} &= 2\pi\tau^2 \int [d\mathbf{k}] \int [d\mathbf{k}'] \varpi_{\mathbf{k}\mathbf{k}'}^{(3a)} (v_{\mathbf{k}}^x - v_{\mathbf{k}'}^x) \partial_{\mathbf{k}}^y f_{\mathbf{k}}^0 = \frac{V_1^3}{n_i V_0^4} \frac{m(\varepsilon^2 - m^2)^2}{(\varepsilon^2 + 3m^2)^2},\\
\chi^{sk,2} &= 2\pi\tau^2 \int [d\mathbf{k}] \int [d\mathbf{k}'] \varpi_{\mathbf{k}\mathbf{k}'}^{(4a)} (v_{\mathbf{k}}^x - v_{\mathbf{k}'}^x) \partial_{\mathbf{k}}^y f_{\mathbf{k}}^0 = \frac{3m(\varepsilon^2 - m^2)^2}{2\varepsilon(\varepsilon^2 + 3m^2)^2},
\end{aligned}
\tag{S203}
$$

where the factor 2 in $\sigma_{xy}^{sj}$ comes from the fact that two mechanisms of side-jump contribution are identical in the absence of direct interband scatterings, and we have divided the skew-scattering into two terms according to the third- and fourth-order antisymmetric scattering rates. Notably, only $\chi^{sk,1}$ is dependent on the disorder concentration, even if $\chi^{sj}$, $\chi^{sk,1}$, and $\chi^{sk,2}$ all originate from the disorder. The reason is that $\chi^{sj}$ and $\chi^{sk,2}$ are related to the second-order disorder correlation $n_i V_0^2$ and the relaxation time $\tau(\propto 1/n_i V_0^2)$. As a result, they cancel each other. For $\chi^{sk,1}$, it is related to the third-order disorder correlation $n_i V_1^3$ and the relaxation time $\tau(\propto 1/n_i V_0^2)$, which gives rise to the disorder concentration dependence, i.e., $\chi^{sk,1} \propto \left(n_i V_0^4/V_1^3\right)^{-1}$. For this reason, $\chi^{sk,1}$ is called extrinsic skew-scattering while $\chi^{sk,2}$ intrinsic skew-scattering [3]. Consequently, the anomalous transport coefficients are given by

$$
\begin{aligned}
\sigma_{xy}^{\chi} &= -\frac{e^2}{h} \mathcal{C}_0^{\chi},\\
\alpha_{xy}^{\chi} &= \frac{k_B e}{h} \mathcal{C}_1^{\chi},\\
\kappa_{xy}^{\chi} &= -\frac{k_B^2 T}{h} \mathcal{C}_2^{\chi}.
\end{aligned}
\tag{S204}
$$

We take the intrinsic contribution as an example to show how to use the Sommerfeld expansion to obtain finite temperature case. The Sommerfeld expansion reads

$$
\int \mathcal{F}(\varepsilon) \left(-\frac{\partial f_0}{\partial \varepsilon}\right) d\varepsilon \simeq \mathcal{F}(\mu) + \frac{\pi^2}{6} (k_B T)^2 \mathcal{F}''(\varepsilon)\Big|_{\varepsilon=\mu} + \frac{7\pi^4}{360} (k_B T)^4 \mathcal{F}^{(4)}(\varepsilon)\Big|_{\varepsilon=\mu} + \mathcal{O}(T^6).
\tag{S205}
$$

where $\mathcal{F}(\varepsilon)$ is an arbitrary function of $\varepsilon$. Thus, the intrinsic contribution of the anomalous electric Hall conductivity can be written as

$$
\begin{aligned}
\sigma_{xy}^{in} &= \frac{-e^2}{\hbar} \int d\varepsilon \mathcal{F}(\varepsilon) \left(-\frac{\partial f_0}{\partial \varepsilon}\right)\\
&\simeq \frac{-e^2}{\hbar} \left[\mathcal{F}(\mu) + \frac{\pi^2}{6} (k_B T)^2 \mathcal{F}''(\mu) + \frac{7\pi^4}{360} (k_B T)^4 \mathcal{F}^{(4)}(\mu)\right] + \mathcal{O}(T^6)\\
&= -\frac{e^2}{h} \left[\frac{m}{2\mu} + \frac{\pi^2 m}{6\mu^3} (k_B T)^2 + \frac{7\pi^4 m}{30\mu^5} (k_B T)^4\right],
\end{aligned}
\tag{S206}
$$

here $\mathcal{F}(\varepsilon)$ is nothing but the kernel function for the intrinsic contribution, i.e., $\mathcal{F}(\varepsilon) = m/2\varepsilon$. Similarly, we can obtain the anomalous electric Hall conductivities for all contributions

$$
\begin{aligned}
\sigma_{xy}^{in} &= -\frac{e^2}{h} \left[\frac{m}{2\mu} + \frac{\pi^2 m}{6\mu^3} (k_B T)^2 + \frac{7\pi^4 m}{30\mu^5} (k_B T)^4\right],\\
\sigma_{xy}^{sj} &= -\frac{e^2}{h} \frac{2m(\mu^2 - m^2)}{\mu(\mu^2 + 3m^2)},\\
\sigma_{xy}^{sk,1} &= -\frac{e^2}{h} \frac{V_1^3}{n_i V_0^4} \frac{m(\mu^2 - m^2)^2}{(\mu^2 + 3m^2)^2},\\
\sigma_{xy}^{sk,2} &= -\frac{e^2}{h} \frac{3m(\mu^2 - m^2)^2}{2\mu(\mu^2 + 3m^2)^2}.
\end{aligned}
\tag{S207}
$$

The anomalous thermoelectric Hall conductivities are given as

$$\begin{aligned}
\alpha_{xy}^{in} &= -\frac{k_B e}{h}\left[\frac{\pi^2 m}{6\mu^2}k_BT + \frac{7\pi^4 m}{30\mu^4}(k_BT)^3\right],\\
\alpha_{xy}^{sj} &= -\frac{k_B e}{h}\frac{2\pi^2 m(\mu^4 - 6\mu^2 m^2 - 3m^4)}{3\mu^2(\mu^2+3m^2)}k_BT,\\
\alpha_{xy}^{sk,1} &= \frac{k_B e}{h}\frac{V_1^3}{n_i V_0^4}\frac{16\pi^2 m^3\mu(\mu^2-m^2)}{3(\mu^2+3m^2)^3}k_BT,\\
\alpha_{xy}^{sk,2} &= -\frac{k_B e}{h}\frac{\pi^2 m(\mu^2-m^2)(\mu^4-14\mu^2m^2-3m^4)}{2\mu^2(\mu^2+3m^2)^3}k_BT,
\end{aligned} \tag{S208}$$

and the anomalous thermal Hall conductivities

$$\begin{aligned}
\kappa_{xy}^{in} &= -\frac{k_B^2 T}{h}\left[\frac{\pi^2 m}{6\mu} + \frac{7\pi^4 m}{30\mu^3}(k_BT)^2\right],\\
\kappa_{xy}^{sj} &= -\frac{k_B^2 T}{h}\frac{2\pi^2 m(\mu^2-m^2)}{3\mu(\mu^2+3m^2)},\\
\kappa_{xy}^{sk,1} &= -\frac{k_B^2 T}{h}\frac{V_1^3}{n_i V_0^4}\frac{\pi^2 m(\mu^2-m^2)^2}{3(\mu^2+3m^2)^2},\\
\kappa_{xy}^{sk,2} &= -\frac{k_B^2 T}{h}\frac{\pi^2 m(\mu^2-m^2)^2}{2\mu(\mu^2+3m^2)^2}.
\end{aligned} \tag{S209}$$

### D. Wiedemann-Franz law

For the conventional electron gas, the Drude conductivity and thermal conductivity are

$$\sigma_0 = \frac{ne^2\tau}{m}, \qquad \kappa_0 = \frac{\pi^2 n\tau k_B^2}{3m}T, \tag{S210}$$

we can get the Wiedemann-Franz law

$$\frac{\kappa_0}{\sigma_0} = \frac{1}{3}\left(\frac{\pi k_B}{e}\right)^2 T = L_0 T, \tag{S211}$$

where $L_0 = (\pi k_B/e)^2/3$ is known as the Lorentz number.

For the intrinsic contribution, the ratio of thermal conductivity and electric conductivity reads

$$\frac{\kappa_{xy}^{in}}{\sigma_{xy}^{in}} = \frac{15\mu^2/\pi^2 + 21(k_BT)^2}{15\mu^2/\pi^2 + 5(k_BT)^2 + 7\pi^2(k_BT)^4/\mu^2}L_0T. \tag{S212}$$

We can obtain the critical chemical potential $\mu_c$ as

$$\frac{15\mu_c^2/\pi^2 + 21(k_BT)^2}{15\mu_c^2/\pi^2 + 5(k_BT)^2 + 7\pi^2(k_BT)^4/\mu_c^2}L_0 = L_0, \tag{S213}$$

thus we have

$$16(k_BT)^2 = \frac{1}{\mu_c^2}7\pi^2(k_BT)^4, \tag{S214}$$

and the critical chemical potential reads

$$\mu_c = \frac{\sqrt{7}\pi}{4}k_BT, \tag{S215}$$

here we only consider the upper band. If $\mu > \mu_c$, $\kappa_{xy}^{in}/\sigma_{xy}^{in}$ higher than $L_0T$, and if $\mu < \mu_c$, $\kappa_{xy}^{in}/\sigma_{xy}^{in}$ lower than $L_0T$. According to the relationship between $\mu$ and $\mu_c$, there are two possible limits of our result. Firstly, when the chemical potential is far away from the band edge ($\mu \gg \mu_c$), we have

$$\begin{aligned}\frac{\kappa_{xy}^{in}}{\sigma_{xy}^{in}} &= \left[1 + \frac{16(k_BT)^2 - 7\pi^2(k_BT)^4/\mu^2}{15\mu^2/\pi^2 + 5(k_BT)^2 + 7\pi^2(k_BT)^4/\mu^2}\right] L_0T \\ &\approx \left(1 + \frac{16\pi^2}{15}\frac{k_B^2T^2}{\mu^2}\right) L_0T,\end{aligned} \tag{S216}$$

secondly, when the chemical potential is near the band edge ($\mu \ll \mu_c$)

$$\begin{aligned}\frac{\kappa_{xy}^{in}}{\sigma_{xy}^{in}} &= \left[1 + \frac{-16(k_BT)^2 + 7\pi^2(k_BT)^4/\mu^2}{15\mu^2/\pi^2 + 21(k_BT)^2}\right]^{-1} L_0T \\ &\approx \left(1 + \frac{\pi^2}{3}\frac{k_B^2T^2}{\mu^2}\right)^{-1} L_0T.\end{aligned} \tag{S217}$$

One can rewrite the two expressions together

$$\frac{\kappa_{xy}^{in}}{\sigma_{xy}^{in}} = \begin{cases} \left(1 + \frac{16\pi^2}{15}\frac{k_B^2T^2}{\mu^2}\right) L_0T, & \mu \gg \mu_c; \\ \left(1 + \frac{\pi^2}{3}\frac{k_B^2T^2}{\mu^2}\right)^{-1} L_0T, & \mu \ll \mu_c. \end{cases} \tag{S218}$$

For each of the extrinsic mechanisms, we have

$$\frac{\kappa_{xy}^{sj(0)}}{\sigma_{xy}^{sj(0)}} = L_0T, \qquad \frac{\kappa_{xy}^{sk,1(0)}}{\sigma_{xy}^{sk,1(0)}} = L_0T, \qquad \frac{\kappa_{xy}^{sk,2(0)}}{\sigma_{xy}^{sk,2(0)}} = L_0T. \tag{S219}$$

If we keep all contributions up to the leading order (i.e., $\sigma \propto (k_BT)^0$, $\kappa \propto (k_BT)^2$), and sum them up, we have

$$\begin{aligned}\sigma_{xy}^{tot(0)} &= \sigma_{xy}^{in(0)} + \sigma_{xy}^{sj(0)} + \sigma_{xy}^{sk,1(0)} + \sigma_{xy}^{sk,2(0)} = -\frac{e^2}{h}\frac{4n_iV_0^4\mu(\mu^2+m^2) + m(\mu^2-m^2)}{n_iV_0^4(\mu^2+3m^2)^2}, \\ \kappa_{xy}^{tot(0)} &= \kappa_{xy}^{in(0)} + \kappa_{xy}^{sj(0)} + \kappa_{xy}^{sk,1(0)} + \kappa_{xy}^{sk,2(0)} = -\frac{k_B^2T}{h}\frac{4\pi^2n_iV_0^4\mu(\mu^2+m^2) + m(\mu^2-m^2)}{3n_iV_0^4(\mu^2+3m^2)^2},\end{aligned} \tag{S220}$$

thus,

$$\frac{\kappa_{xy}^{tot(0)}}{\sigma_{xy}^{tot(0)}} = L_0T. \tag{S221}$$

which also recovers the Wiedemann-Franz law.

To see the deviation of the Wiedemann-Franz law induced by the disorder analytically, we need to expand the electric conductivities to the next leading order, i.e.,

$$\begin{aligned}\sigma_{xy}^{sj} &= \frac{e^2}{h}\left[\frac{2m(m^2-\mu^2)}{\mu\left(3m^2+\mu^2\right)} + \frac{2\pi^2m\left(9m^4\mu^2+15m^2\mu^4+9m^6-\mu^6\right)}{3\left(3m^2\mu+\mu^3\right)^3}(k_BT)^2\right], \\ \sigma_{xy}^{sk,1} &= \frac{e^2}{h}\frac{V_1^3}{n_iV_0^4}\left[-\frac{m\left(m^2-\mu^2\right)^2}{\left(3m^2+\mu^2\right)^2} + \frac{8\pi^2m^3\left(-14m^2\mu^2+3m^4+3\mu^4\right)}{3\left(3m^2+\mu^2\right)^4}(k_BT)^2\right], \\ \sigma_{xy}^{sk,2} &= -\frac{e^2}{h}\left[\frac{3m\left(m^2-\mu^2\right)^2}{2\mu\left(3m^2+\mu^2\right)^2} + \frac{\pi^2m\left(12m^6\mu^2+78m^4\mu^4-36m^2\mu^6+9m^8+\mu^8\right)}{2\mu^3\left(3m^2+\mu^2\right)^4}(k_BT)^2\right].\end{aligned} \tag{S222}$$

Accordingly, the side-jump contribution to the ratio of thermal Hall conductivity and electric Hall conductivity are

given by

$$\frac{\kappa_{xy}^{sj}}{\sigma_{xy}^{sj}} = \frac{3(m^2-\mu^2)\left(3m^2\mu+\mu^3\right)^2}{\pi^2 k_B^2 T^2\left(9m^4\mu^2+15m^2\mu^4+9m^6-\mu^6\right)+3(m^2-\mu^2)\left(3m^2\mu+\mu^3\right)^2} L_0 T$$
$$= \left[1+\frac{\pi^2 k_B^2 T^2\left(9m^4\mu^2+15m^2\mu^4+9m^6-\mu^6\right)}{3(m^2-\mu^2)\left(3m^2\mu+\mu^3\right)^2}\right]^{-1} L_0 T \tag{S223}$$
$$= \left[1+\frac{\pi^2 k_B^2 T^2}{\mu^2}\frac{9t^6+9t^4+15t^2-1}{9t^6-3t^4-5t^2-1}\right]^{-1} L_0 T,$$

where we have defined $t = m/\mu$. The skew-scattering contributions read

$$\frac{\kappa_{xy}^{sk,1}}{\sigma_{xy}^{sk,1}} = \frac{3\left(2m^2\mu^2-3m^4+\mu^4\right)^2}{-8\pi^2 k_B^2 T^2 m^2\left(-14m^2\mu^2+3m^4+3\mu^4\right)+3\left(2m^2\mu^2-3m^4+\mu^4\right)^2} L_0 T$$
$$= \left[1-\frac{8\pi^2 k_B^2 T^2 m^2\left(-14m^2\mu^2+3m^4+3\mu^4\right)}{3\left(2m^2\mu^2-3m^4+\mu^4\right)^2}\right]^{-1} L_0 T \tag{S224}$$
$$= \left[1-\frac{8\pi^2 k_B^2 T^2}{3\mu^2}\frac{3t^6-14t^4+3t^2}{\left(-3t^3+2t^2+1\right)^2}\right]^{-1} L_0 T,$$

and

$$\frac{\kappa_{xy}^{sk,2}}{\sigma_{xy}^{sk,2}} = \frac{3\left(2m^2\mu^3-3m^4\mu+\mu^5\right)^2}{\pi^2 k_B^2 T^2\left(12m^6\mu^2+78m^4\mu^4-36m^2\mu^6+9m^8+\mu^8\right)+3\left(2m^2\mu^3-3m^4\mu+\mu^5\right)^2} L_0 T$$
$$= \left[1+\frac{\pi^2 k_B^2 T^2\left(12m^6\mu^2+78m^4\mu^4-36m^2\mu^6+9m^8+\mu^8\right)}{3\left(2m^2\mu^3-3m^4\mu+\mu^5\right)^2}\right]^{-1} L_0 T \tag{S225}$$
$$= \left[1+\frac{\pi^2 k_B^2 T^2}{3\mu^2}\frac{9t^8+12t^6+78t^4-36t^2+1}{\left(-3t^4+2t^2+1\right)^2}\right]^{-1} L_0 T.$$

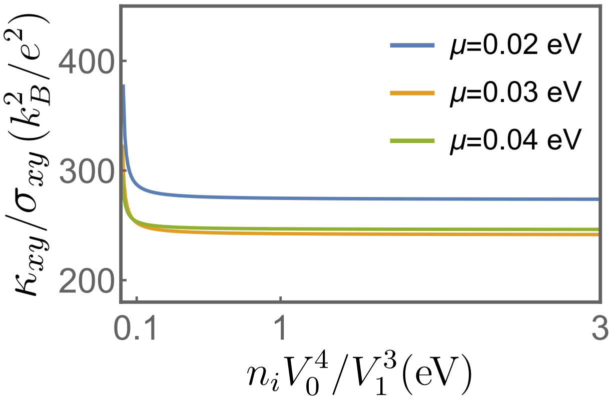


FIG. S1. The total (topological + disorder) contribution to the ratio $\kappa_{xy}/\sigma_{xy}$ as a function of the disorder concentration. The parameters are $m = 0.017$ eV, $v = 1$ eV·nm, and $T = 100$ K.

To examine the effect of the disorder concentration, we numerically evaluate $\kappa_{xy}/\sigma_{xy}$ by using $\mathcal{C}_n^{\chi}$. The disorder concentration is only reflected in the extrinsic skew-scattering contribution, i.e., the quantity $n_i V_0^4/V_1^3$, which has the dimension of energy. In Fig. S1, we present the numerical results of $\kappa_{xy}/\sigma_{xy}$ as a function of disorder concentration. Specifically, the ratio $\kappa_{xy}/\sigma_{xy}$ become divergent when $n_i V_0^4/V_1^3 \to 0$. This is consistent with $\chi^{sk,1} \propto \left(n_i V_0^4/V_1^3\right)^{-1}$. The curves then fall sharply around 0.1 eV, and they remain stable when $n_i V_0^4/V_1^3$ increases continually. The reason is that only $\chi^{sk,1}$ has the dependence of the disorder concentration, and $\chi^{sk,1} \to 0$ when $n_i V_0^4/V_1^3$ raises. In our calculation, we adopt $n_i V_0^4/V_1^3 = 1$ eV.

### E. Mott relation

The classical Mott relation is known as

$$\alpha_0 = -eL_0T\frac{\partial\sigma(\mu)}{\partial\mu}. \tag{S226}$$

For the intrinsic contribution, we have

$$\begin{aligned}\frac{\alpha_{xy}^{in}}{\sigma_{xy}^{in}} &= \frac{3e\mu}{3\mu^2+\pi^2k_B^2T^2}L_0T \\ &= \left(\frac{\mu}{e}+\frac{\pi^2}{3}\frac{k_B^2T^2}{e\mu}\right)^{-1}L_0T,\end{aligned} \tag{S227}$$

for the extrinsic mechanisms,

$$\begin{aligned}-eL_0T\frac{\partial\sigma_{xy}^{sj(0)}(\mu)}{\partial\mu} &= -\frac{k_Be}{h}\frac{2\pi^2m(\mu^4-6\mu^2m^2-3m^4)}{3\mu^2(\mu^2+3m^2)}k_BT = \alpha_{xy}^{sj(0)}, \\ -eL_0T\frac{\partial\sigma_{xy}^{sk,1(0)}(\mu)}{\partial\mu} &= \frac{k_Be}{h}\frac{V_1^3}{n_iV_0^4}\frac{16\pi^2m^3\mu(\mu^2-m^2)}{3(\mu^2+3m^2)^3}k_BT = \alpha_{xy}^{sk,1(0)}, \\ -eL_0T\frac{\partial\sigma_{xy}^{sk,2(0)}(\mu)}{\partial\mu} &= -\frac{k_Be}{h}\frac{\pi^2m(\mu^2-m^2)(\mu^4-14\mu^2m^2-3m^4)}{2\mu^2(\mu^2+3m^2)^3}k_BT = \alpha_{xy}^{sk,2(0)},\end{aligned} \tag{S228}$$

they also satisfy the Mott relation for each of the intrinsic, side-jump, and skew-scattering contributions, respectively. Like $\sigma_{xy}^{tot(0)}$ and $\kappa_{xy}^{tot(0)}$, we can sum up all contributions of anomalous thermoelectric Hall effect up to the leading order ($\alpha \propto (k_BT)^2$)

$$\alpha_{xy}^{tot(0)} = \alpha_{xy}^{in(0)}+\alpha_{xy}^{sj(0)}+\alpha_{xy}^{sk,1(0)}+\alpha_{xy}^{sk,2(0)} = -\frac{k_Be}{h}\frac{4\pi^2[n_iV_0^4m(\mu^4-6\mu^2m^2-3m^4)-4\mu m^3(\mu^2-m^2)V_1^3]}{3n_iV_0^4(\mu^2+3m^2)^3}, \tag{S229}$$

and

$$-eL_0T\frac{\partial\sigma_{xy}^{tot(0)}(\mu)}{\partial\mu} = -\frac{k_Be}{h}\frac{4\pi^2[n_iV_0^4m(\mu^4-6\mu^2m^2-3m^4)-4\mu m^3(\mu^2-m^2)V_1^3]}{3n_iV_0^4(\mu^2+3m^2)^3}, \tag{S230}$$

which can also recover the Mott relation, i.e.,

$$-eL_0T\frac{\partial\sigma_{xy}^{tot(0)}(\mu)}{\partial\mu} = \alpha_{xy}^{tot(0)}. \tag{S231}$$

## SVII. TILTED WEYL NODE

### A. Eigen solutions

A local Hamiltonian near the Weyl node can be written as

$$\mathcal{H} = s(v\mathbf{k}\cdot\sigma+tk_z), \tag{S232}$$

where $s=\pm1$ is the label that distinguishes the chirality of the Weyl node. The tilt term $tk_z$ is necessary to cover more general case, and we assume $t/v \ll 1$ to get the analytical result. The eigen energies are

$$\varepsilon_{\mathbf{k}}^{\pm} = \pm\sqrt{v^2(k_x^2+k_y^2+k_z^2)}+stk_z = \pm\varepsilon_{\mathbf{k}}^0+stk_z, \tag{S233}$$

where $\varepsilon_{\mathbf{k}}^0 = vk$ with $k=\sqrt{k_x^2+k_y^2+k_z^2}$, with the eigen states

$$|u_{\mathbf{k}}^+\rangle = \begin{bmatrix}\cos(\theta/2)\\ \sin(\theta/2)e^{i\phi}\end{bmatrix}, \qquad |u_{\mathbf{k}}^-\rangle = \begin{bmatrix}\sin(\theta/2)\\ -\cos(\theta/2)e^{i\phi}\end{bmatrix}, \tag{S234}$$

where the definition of $\theta$ and $\phi$ are

$$\cos\theta = s\frac{k_z}{k}, \qquad \tan\phi = \frac{k_y}{k_x}. \tag{S235}$$

In the spherical coordinate, $k_x = k\sin\theta\cos\phi$, $k_y = k\sin\theta\sin\phi$, $k_z = k\cos\theta$. The velocity along $\hat{x}$ and $\hat{y}$ axis are

$$v_\pm^x = \pm\frac{1}{\hbar}\frac{vk_x}{k}, \qquad v_\pm^y = \pm\frac{1}{\hbar}\frac{vk_y}{k}. \tag{S236}$$

We set the $\mathbf{k}$ space as the parameter space, i.e. $\mathbf{R} \equiv (k_x, k_y, k_z)$. The Berry curvature in the Cartesian coordinate is given by

$$\begin{aligned}
\Omega_{\mathbf{k}}^{\pm} &= \mp\left(\frac{1}{2k^2}\sin\theta\cos\phi, \frac{1}{2k^2}\sin\theta\sin\phi, \frac{1}{2k^2}\cos\theta\right)\\
&= \mp s\left(\frac{1}{2k^2}\frac{\sqrt{k_x^2+k_y^2}}{k}\frac{k_x}{\sqrt{k_x^2+k_y^2}}, \frac{1}{2k^2}\frac{\sqrt{k_x^2+k_y^2}}{k}\frac{k_y}{\sqrt{k_x^2+k_y^2}}, \frac{1}{2k^2}\frac{k_z}{k}\right)\\
&= \mp s\left(\frac{k_x}{2k^3}, \frac{k_y}{2k^3}, \frac{k_z}{2k^3}\right).
\end{aligned} \tag{S237}$$

### B. Anomalous Hall conductivity

We consider the anomalous Hall conductivity in the absence of time reversal symmetry. The system is isotropic with the constant relaxation time. We only consider the upper band. The general relaxation time is given by

$$\frac{1}{\tau} = \sum_{\mathbf{k}'}\varpi_{\mathbf{k}\mathbf{k}'}^{(2)}\left(1-\cos\alpha\right), \tag{S238}$$

where $\alpha$ is the angle between $\mathbf{k}$ and $\mathbf{k}'$, which is given by

$$\cos\alpha = \frac{\mathbf{k}\cdot\mathbf{k}'}{|\mathbf{k}||\mathbf{k}'|} = \cos\theta\cos\phi\cos\theta'\cos\phi' + \cos\theta\sin\phi\cos\theta'\sin\phi' + \sin\theta\sin\theta'. \tag{S239}$$

We can obtain

$$\begin{aligned}
\frac{1}{\tau} &= \int\frac{d^3\mathbf{k}'}{(2\pi)^3}\varpi_{\mathbf{k}\mathbf{k}'}^{(2)}\left(1-\cos\alpha\right)\\
&= \frac{n_iV_0^2}{8\pi^2\hbar}\int_0^\infty dk'\int_0^\pi d\theta'\int_0^{2\pi} d\phi' k'^2\sin\theta'\left[1+\cos\theta\cos\theta'+\sin\theta\sin\theta'\cos(\phi-\phi')\right]\\
&\quad\times\left[1-\cos\theta\cos\phi\cos\theta'\cos\phi'+\cos\theta\sin\phi\cos\theta'\sin\phi'+\sin\theta\sin\theta'\right]\delta(\varepsilon_{\mathbf{k}}-\varepsilon_{\mathbf{k}'})\\
&= \frac{n_iV_0^2}{8\pi^2\hbar}\int_0^\infty dk'\int_0^\pi d\theta'\int_0^{2\pi} d\phi' k'^2\sin\theta'\left[1+\cos\theta\cos\theta'+\sin\theta\sin\theta'\cos(\phi-\phi')\right]\\
&\quad\times\left[1-\cos\theta\cos\phi\cos\theta'\cos\phi'+\cos\theta\sin\phi\cos\theta'\sin\phi'+\sin\theta\sin\theta'\right]\frac{1}{v}\delta(k-k')\\
&= \frac{n_iV_0^2}{\hbar}\frac{\varepsilon^2}{3\pi v^3},
\end{aligned} \tag{S240}$$

by noting that

$$\varpi_{\mathbf{k}\mathbf{k}'}^{(2)} = \frac{\pi}{\hbar}n_iV_0^2\left[1+\cos\theta\cos\theta'+\sin\theta\sin\theta'\cos(\phi-\phi')\right]\delta(\varepsilon_{\mathbf{k}}-\varepsilon_{\mathbf{k}'}). \tag{S241}$$

The anomalous Hall conductivity in the $x$-$y$ plane reads

$$\sigma_{xy}^{tot} = \sigma_{xy}^{in} + \sigma_{xy}^{sj,1} + \sigma_{xy}^{sj,2} + \sigma_{xy}^{sk}, \tag{S242}$$

with

$$\begin{aligned}
\sigma_{xy}^{in} &= -\frac{e^2}{\hbar}\sum_l \Omega_l^z f_l^0, \\
\sigma_{xy}^{sj,1} &= -\frac{e^2}{\hbar}\tau\int [d\mathbf{k}] v_x^{sj}\partial_{\mathbf{k}}^y f_{\mathbf{k}}^0, \\
\sigma_{xy}^{sj,2} &= \frac{e^2}{\hbar}\tau\int [d\mathbf{k}] v_y^{sj}\partial_{\mathbf{k}}^x f_{\mathbf{k}}^0, \\
\sigma_{xy}^{sk} &= -\frac{e^2}{\hbar}\tau^2\int [d\mathbf{k}]\int [d\mathbf{k}']\varpi_{\mathbf{k}\mathbf{k}'}^{as}(v_{\mathbf{k}}^x - v_{\mathbf{k}'}^x)\partial_{\mathbf{k}}^y f_{\mathbf{k}}^0.
\end{aligned} \tag{S243}$$

We assume that the Fermi energy cuts the conduction band, thus the band index can be neglected in the side-jump and skew-scattering contributions.

### 1. *Intrinsic contribution*

Firstly, we consider the valence band which is completely filled (Fermi energy cuts the conduction band). Its intrinsic contribution can be totally characterized by the band topology. The $k_z$-dependent Chern number for the valence band is given by

$$\begin{aligned}
n_c(k_z) &= 2\pi\int \frac{d^2\mathbf{k}}{(2\pi)^2}\Omega_{\mathbf{k}}^- \\
&= 2\pi\int \frac{d^2\mathbf{k}}{(2\pi)^2} s\frac{k_z}{2\sqrt{k_\perp^2+k_z^2}^3} \\
&= s\frac{1}{4\pi}\int_0^{2\pi} d\phi\int_0^\infty k_\perp dk_\perp(-2)\frac{d\cos\theta}{dk_\perp^2} \\
&= -s\frac{1}{2}\int_0^\infty dk_\perp^2\frac{d\cos\theta}{dk_\perp^2} \\
&= s\frac{1}{2}\mathrm{sgn}(k_z),
\end{aligned} \tag{S244}$$

where $k_\perp = \sqrt{k_x^2+k_y^2}$. In the $k_x$-$k_y$ plane, the system for a given $k_z$ can be regraded as a series of 2D massive Dirac model, where $k_z$ plays the role of the mass term. We can obtain

$$\sigma_{xy}^{\mathrm{2D}} = \frac{e^2}{h}n_c(k_z) = s\frac{e^2}{2h}\mathrm{sgn}(k_z). \tag{S245}$$

We assume that the Weyl nodes are located at $(0,0,\pm k_c)$, and the topological contribution to the anomalous Hall conductivity is found as

$$\begin{aligned}
\sigma_{xy}^{in,1} &= \frac{e^2}{2h}\int_0^{k_c}\frac{dk_z}{2\pi}\mathrm{sgn}(k_z) - \frac{e^2}{2h}\int_{-k_c}^0\frac{dk_z}{2\pi}\mathrm{sgn}(k_z) \\
&= \frac{e^2}{2h}\frac{1}{2\pi}k_c + \frac{e^2}{2h}\frac{1}{2\pi}k_c \\
&= \frac{e^2}{h}\frac{Q}{4\pi},
\end{aligned} \tag{S246}$$

where $Q = 2k_c$ is the distance between two Weyl nodes. Furthermore, a 3D massless Dirac model could be regarded as an effective model nearing a single node of the Weyl semimetal. We can integrate enclosing one node to get the

topological charge

$$
\begin{aligned}
\frac{1}{2\pi}\oint \Omega_{\mathbf{k}}^{-}\cdot d\mathbf{S} &= \frac{1}{2\pi}s\int\left(\nabla\cdot\frac{\mathbf{k}}{2k^3}\right)dV \\
&= \frac{1}{4\pi}s\int dk\int_0^{\pi}d\theta\int_0^{2\pi}d\phi k^2\sin\theta\frac{1}{k^2}\left(\frac{\partial}{\partial k}\frac{k^2}{k^2}\right) \\
&= s\int dk\left(\frac{\partial}{\partial k}\frac{k^2}{k^2}\right) \\
&= s,
\end{aligned}
\tag{S247}
$$

this integration could be simplified, if we notice that $\nabla\cdot(\mathbf{r}/r^3) = 4\pi\delta(\mathbf{r})$. The result means that the topological charge is equal to $\pm1$ around the Weyl node, which could be regarded as the source or sink of the Berry curvature.

Now, we consider the conduction band,

$$
\begin{aligned}
\sigma_{xy}^{in,2} &= -\frac{e^2}{\hbar}\int\frac{d^3\mathbf{k}}{(2\pi)^3}f^0(\varepsilon_{\mathbf{k}}^0 + stk_z)\Omega_{\mathbf{k}}^{z,+} \\
&\simeq -\frac{e^2}{\hbar}\int\frac{d^3\mathbf{k}}{(2\pi)^3}stk_z\left(\frac{\partial f^0}{\partial\varepsilon_{\mathbf{k}}^0}\right)\left(-s\frac{k_z}{2k^3}\right) \\
&= -\frac{e^2}{\hbar}\frac{1}{(2\pi)^3}\int_0^{2\pi}d\phi\int_0^{\pi}d\theta\int dkk^2\sin\theta tk\cos\theta\frac{k\cos\theta}{2k^3}\delta(\varepsilon-\varepsilon_f) \\
&= -\frac{e^2}{\hbar}\frac{1}{(2\pi)^3}\int_0^{2\pi}d\phi\int_0^{\pi}d\theta\int dktk\sin\theta\cos^2\theta\frac{1}{2v}\delta(k-k_f) \\
&= -\frac{e^2}{h}\frac{t\varepsilon}{6\pi v^2},
\end{aligned}
\tag{S248}
$$

where we have used

$$
f^0(\varepsilon_{\mathbf{k}}^0 + tk_z) \simeq f^0(\varepsilon_{\mathbf{k}}^0) + tk_z\frac{\partial f^0}{\partial\varepsilon_{\mathbf{k}}^0}. \tag{S249}
$$

The contribution from the first term (depending on $s$) will vanish after the summation of two nodes, we just drop it. Therefore, the total conductivity is

$$
\sigma_{xy}^{in} = \sigma_{xy}^{in,1} + \sigma_{xy}^{in,2} = \frac{e^2}{h}\frac{Q}{4\pi} - \frac{e^2}{h}\frac{t\varepsilon}{3\pi v^2}, \tag{S250}
$$

here we have summed over both Weyl nodes in a pair ($s = \pm1$) in the second term.

### *2. Side-jump contribution*

The direct interband scattering is not energetically allowed in the weak-disorder limit of our model. We consider only the coordinate shift effect of scattering in the upper band

$$
\delta\mathbf{r}_{\mathbf{k}\mathbf{k}'} = \frac{\Omega_{\mathbf{k}}^{+}\times(\mathbf{k}-\mathbf{k}')}{|\langle u_{\mathbf{k}}^{+}|u_{\mathbf{k}'}^{+}\rangle|^2}, \tag{S251}
$$

and the corresponding side-jump velocity components read

$$\begin{aligned}
v_x^{sj} &= \int \frac{d^3\mathbf{k}'}{(2\pi)^3}\varpi^{(2)}_{\mathbf{k}\mathbf{k}'}\delta r^x_{\mathbf{k}'\mathbf{k}} \\
&= \frac{n_i V_0^2}{8\pi^2\hbar}\int_0^\infty dk' \int_0^\pi d\theta' \int_0^{2\pi} d\phi' k'^2 \sin\theta' \left[1+\cos\theta\cos\theta' + \sin\theta\sin\theta'\cos(\phi-\phi')\right]\delta(\varepsilon_{\mathbf{k}}-\varepsilon_{\mathbf{k}'})\frac{\Omega^{y,+}_{\mathbf{k}'}(k'_z-k_z)-\Omega^{z,+}_{\mathbf{k}'}(k'_y-k_y)}{|\langle u^+_{\mathbf{k}}|u^+_{\mathbf{k}'}\rangle|^2} \\
&\simeq \frac{n_i V_0^2}{8\pi^2\hbar}\int_0^\infty dk' \int_0^\pi d\theta' \int_0^{2\pi} d\phi' k'^2 \sin\theta' \left[1+\cos\theta\cos\theta' + \sin\theta\sin\theta'\cos(\phi-\phi')\right] \\
&\times \left\{ s\frac{-k'\sin\theta'\sin\phi'}{2k'^3}\frac{k'\cos\theta'-k\cos\theta}{\frac{1}{2}\left[1+\cos\theta\cos\theta'+\sin\theta\sin\theta'\cos(\phi'-\phi)\right]} - s\frac{-k'\cos\theta'}{2k'^3}\frac{k'\sin\theta'\sin\phi'-k\sin\theta\sin\phi}{\frac{1}{2}\left[1+\cos\theta\cos\theta'+\sin\theta\sin\theta'\cos(\phi'-\phi)\right]}\right\} \\
&\times \left[\frac{1}{v}\delta(k-k') + st(k\cos\theta - k'\cos\theta')\frac{1}{v^2}\frac{\partial}{\partial k'}\delta(k-k')\right] \\
&= -\frac{n_i V_0^2}{\hbar}\frac{tk}{6\pi v^2}\sin\theta\sin\phi,
\end{aligned} \tag{S252}$$

where we have used

$$\begin{aligned}
\delta(\varepsilon_{\mathbf{k}}-\varepsilon_{\mathbf{k}'}) &= \delta(\varepsilon^0_{\mathbf{k}}-\varepsilon^0_{\mathbf{k}'}+stk_z-stk'_z) \\
&\simeq \delta(\varepsilon^0_{\mathbf{k}}-\varepsilon^0_{\mathbf{k}'}) + st(k\cos\theta-k'\cos\theta')\frac{\partial}{\partial\varepsilon^0_{\mathbf{k}'}}\delta(\varepsilon^0_{\mathbf{k}}-\varepsilon^0_{\mathbf{k}'}) \\
&= \frac{1}{v}\delta(k-k') + st(k\cos\theta-k'\cos\theta')\frac{1}{v^2}\frac{\partial}{\partial k'}\delta(k-k'),
\end{aligned} \tag{S253}$$

and the integration for the derivative of the $\delta$ function

$$\int_0^\infty dx f(x)\delta'(x-x_0) = f(x)\delta(x-x_0)\Big|_0^\infty - f'(x_0), \tag{S254}$$

in our case, the first term exactly equals 0. Similarly, for $v_y^{sj}$, we have

$$v_y^{sj} = \int \frac{d^3\mathbf{k}'}{(2\pi)^3}\varpi^{(2)}_{\mathbf{k}\mathbf{k}'}\delta r^y_{\mathbf{k}'\mathbf{k}} = \frac{n_i V_0^2}{\hbar}\frac{tk}{6\pi v^2}\sin\theta\cos\phi. \tag{S255}$$

Therefore, we can obtain

$$\begin{aligned}
\sigma^{sj,1}_{xy} &= -\frac{e^2}{\hbar}\tau\int [d\mathbf{k}] v_x^{sj}\partial^y_{\mathbf{k}} f^0_{\mathbf{k}} \\
&= e^2\tau\int \frac{d^3\mathbf{k}}{(2\pi)^3} v_x^{sj} v^y_{\mathbf{k}}\left(-\frac{\partial f^0_{\mathbf{k}}}{\partial\varepsilon_{\mathbf{k}}}\right) \\
&= -\frac{e^2}{8\pi^3}\tau\int_0^\infty dk\int_0^\pi d\theta\int_0^{2\pi} d\phi k^2\sin\theta\frac{n_i V_0^2}{\hbar}\frac{tk}{6\pi v^2}\sin\theta\sin\phi\frac{vk\sin\theta\sin\phi}{\hbar k}\delta(\varepsilon-\varepsilon_f) \\
&= -\frac{n_i V_0^2 e^2}{48\pi^4\hbar^2}\frac{t}{v^2}\tau\int_0^\infty dk\int_0^\pi d\theta\int_0^{2\pi} d\phi k^3\sin^3\theta\sin^2\phi\delta(k-k_f) \\
&= -\frac{n_i V_0^2 e^2}{48\pi^4\hbar^2}\frac{t}{v^2}\frac{3\pi v^3\hbar}{n_i V_0^2\varepsilon^2}\frac{4\pi}{3}k_f^3 \\
&= -\frac{e^2}{h}\frac{t\varepsilon}{6\pi v^2},
\end{aligned} \tag{S256}$$

by noting that

$$\tau = \frac{\hbar}{n_i V_0^2}\frac{3\pi v^3}{\varepsilon^2}, \tag{S257}$$

and

$$\sigma^{sj,2}_{xy} = \frac{e^2}{\hbar}\tau\int [d\mathbf{k}] v_y^{sj}\partial^x_{\mathbf{k}} f^0_{\mathbf{k}} = -\frac{e^2}{h}\frac{t\varepsilon}{6\pi v^2}. \tag{S258}$$

Consequently, the total side-jump scattering contribution reads

$$\sigma_{xy}^{sj} = 2\left(\sigma_{xy}^{sj,1} + \sigma_{xy}^{sj,2}\right) = -\frac{e^2}{h}\frac{2t\varepsilon}{3\pi v^2}, \tag{S259}$$

where we have summed over two nodes $s = \pm 1$.

### 3. Skew-scattering contribution

For our model, the third antisymmetric scattering rates in the upper band can be simplified as

$$\begin{aligned}
\varpi_{\mathbf{k}\mathbf{k}'}^{(3a)} &= \frac{\pi^2 n_i V_1^3}{\hbar}\int [d\mathbf{k}''] \left[\sin\theta\sin\theta'\cos\theta''\sin(\phi-\phi') + \sin\theta'\sin\theta''\cos\theta\sin(\phi'-\phi'')\right. \\
&\quad \left. + \sin\theta\sin\theta''\cos\theta'\sin(\phi''-\phi)\right]\delta(\varepsilon_{\mathbf{k}}^{+} - \varepsilon_{\mathbf{k}''}^{+})\delta(\varepsilon_{\mathbf{k}}^{+} - \varepsilon_{\mathbf{k}'}^{+}) \\
&\simeq \frac{n_i V_1^3}{8\pi\hbar}\int_0^\infty dk'' \int_0^\pi d\theta'' \int_0^{2\pi} d\phi'' k''^2 \sin\theta'' \left[\sin\theta\sin\theta'\cos\theta''\sin(\phi-\phi') + \sin\theta'\sin\theta''\cos\theta\sin(\phi'-\phi'')\right. \\
&\quad \left. + \sin\theta\sin\theta''\cos\theta'\sin(\phi''-\phi)\right]\left[\frac{1}{v}\delta(k-k'') + st(k\cos\theta - k''\cos\theta'')\frac{1}{v^2}\frac{\partial}{\partial k''}\delta(k-k'')\right]\delta(\varepsilon_{\mathbf{k}} - \varepsilon_{\mathbf{k}'}) \\
&= s\frac{n_i V_1^3}{2\hbar}\frac{t\varepsilon^2}{v^4}\sin\theta\sin\theta'\sin(\phi-\phi')\delta(\varepsilon_{\mathbf{k}} - \varepsilon_{\mathbf{k}'}),
\end{aligned} \tag{S260}$$

and the fourth-order

$$\begin{aligned}
\varpi_{\mathbf{k}\mathbf{k}'}^{(4a)} &= \frac{\pi^2 n_i^2 V_0^4}{\hbar}\int [d\mathbf{k}''] \left(\frac{1}{\varepsilon_{\mathbf{k}}^{+} - \varepsilon_{\mathbf{k}}^{-}} + \frac{1}{\varepsilon_{\mathbf{k}'}^{+} - \varepsilon_{\mathbf{k}'}^{-}} + \frac{1}{\varepsilon_{\mathbf{k}''}^{+} - \varepsilon_{\mathbf{k}''}^{-}}\right)\left[\sin\theta\sin\theta'\cos\theta''\sin(\phi-\phi')\right. \\
&\quad \left. + \sin\theta'\sin\theta''\cos\theta\sin(\phi'-\phi'') + \sin\theta\sin\theta''\cos\theta'\sin(\phi''-\phi)\right]\delta(\varepsilon_{\mathbf{k}'}^{+} - \varepsilon_{\mathbf{k}''}^{+})\delta(\varepsilon_{\mathbf{k}}^{+} - \varepsilon_{\mathbf{k}'}^{+}) \\
&\simeq \frac{n_i^2 V_0^4}{16\pi v\hbar}\int_0^\infty dk'' \int_0^\pi d\theta'' \int_0^{2\pi} d\phi'' k''^2 \sin\theta'' \left(\frac{1}{k} + \frac{1}{k'} + \frac{1}{k''}\right)\left[\sin\theta\sin\theta'\cos\theta''\sin(\phi-\phi') + \sin\theta'\sin\theta''\cos\theta\sin(\phi'-\phi'')\right. \\
&\quad \left. + \sin\theta\sin\theta''\cos\theta'\sin(\phi''-\phi)\right]\left[\frac{1}{v}\delta(k-k'') + st(k\cos\theta - k''\cos\theta'')\frac{1}{v^2}\frac{\partial}{\partial k''}\delta(k-k'')\right]\delta(\varepsilon_{\mathbf{k}} - \varepsilon_{\mathbf{k}'}). \\
&= s\frac{2n_i^2 V_0^4}{3\hbar}\frac{t\varepsilon}{v^4}\sin\theta\sin\theta'\sin(\phi-\phi')\delta(\varepsilon_{\mathbf{k}} - \varepsilon_{\mathbf{k}'}),
\end{aligned} \tag{S261}$$

where we have used $\varepsilon_{\mathbf{k}}^{+} - \varepsilon_{\mathbf{k}}^{-} = 2\varepsilon_{\mathbf{k}}^{0}$ and $\varepsilon_{\mathbf{k}}^{0} = vk$. Thus, the skew-scattering contribution can be divided into two parts as

$$\sigma_{xy}^{sk} = \sigma_{xy}^{sk,1} + \sigma_{xy}^{sk,2}, \tag{S262}$$

with

$$\begin{aligned}
\sigma_{xy}^{sk,1} &= -\frac{e^2}{\hbar}\tau^2\int [d\mathbf{k}]\int [d\mathbf{k}']\varpi_{\mathbf{k}\mathbf{k}'}^{(3a)}(v_{\mathbf{k}}^{x} - v_{\mathbf{k}'}^{x})\partial_{\mathbf{k}}^{y} f_{\mathbf{k}}^{0} \\
&= e^2\tau^2\int \frac{d^3\mathbf{k}}{(2\pi)^3}\int \frac{d^3\mathbf{k}'}{(2\pi)^3}\varpi_{\mathbf{k}\mathbf{k}'}^{(3a)}(v_{\mathbf{k}}^{x} - v_{\mathbf{k}'}^{x})v_{\mathbf{k}}^{y}\left(-\frac{\partial f_{\mathbf{k}}^{0}}{\partial\varepsilon_{\mathbf{k}}}\right) \\
&= \frac{n_i V_1^3 e^2}{2^7\pi^6\hbar}\tau^2 s\int_0^\infty dk\int_0^\pi d\theta\int_0^{2\pi} d\phi\int_0^\infty dk'\int_0^\pi d\theta'\int_0^{2\pi} d\phi' k^2 k'^2 \sin^2\theta\sin^2\theta'\frac{t\varepsilon^2}{v^4}\sin(\phi-\phi') \\
&\quad \times \frac{v^2}{\hbar^2}(\sin\theta\cos\phi - \sin\theta'\cos\phi')\sin\theta\sin\phi\frac{1}{v}\delta(k-k')\frac{1}{v}\delta(k-k_f) \\
&= -s\frac{e^2}{h}\frac{V_1^3}{n_i V_0^4}\frac{t\varepsilon^2}{4\pi v^2},
\end{aligned} \tag{S263}$$

by noting that

$$\tau^2 = \frac{\hbar^2}{n_i^2 V_0^4}\frac{9\pi^2 v^6}{\varepsilon^4}. \tag{S264}$$

For the fourth-order scattering rate

$$\begin{aligned}
\sigma_{xy}^{sk,2} &= -\frac{e^2}{\hbar}\tau^2\int[d\mathbf{k}]\int[d\mathbf{k}']\varpi_{\mathbf{kk}'}^{(4a)}(v_{\mathbf{k}}^x - v_{\mathbf{k}'}^x)\partial_{\mathbf{k}}^y f_{\mathbf{k}}^0 \\
&= e^2\tau^2\int\frac{d^3\mathbf{k}}{(2\pi)^3}\int\frac{d^3\mathbf{k}'}{(2\pi)^3}\varpi_{\mathbf{kk}'}^{(4a)}(v_{\mathbf{k}}^x - v_{\mathbf{k}'}^x)v_{\mathbf{k}}^y\left(-\frac{\partial f_{\mathbf{k}}^0}{\partial\varepsilon_{\mathbf{k}}}\right) \\
&= \frac{n_i^2V_0^4e^2}{96\pi^6\hbar}\tau^2 s\int_0^\infty dk\int_0^\pi d\theta\int_0^{2\pi}d\phi\int_0^\infty dk'\int_0^\pi d\theta'\int_0^{2\pi}d\phi' k^2k'^2\sin^2\theta\sin^2\theta'\frac{t\varepsilon}{v^4}\sin(\phi-\phi') \\
&\quad\times\frac{v^2}{\hbar^2}(\sin\theta\cos\phi - \sin\theta'\cos\phi')\sin\theta\sin\phi\frac{1}{v^2}\delta(k-k')\delta(k-k_f) \\
&= -s\frac{e^2}{h}\frac{t\varepsilon}{3\pi v^2}.
\end{aligned} \tag{S265}$$

Accordingly, the skew-scattering contribution vanishes after summing over the two nodes.

### C. Transport coefficients

The total contribution to the anomalous Hall conductivity is

$$\sigma_{xy}^{tot} = \sigma_{xy}^{in} + \sigma_{xy}^{sj} = \frac{e^2}{h}\frac{Q}{4\pi} - \frac{e^2}{h}\frac{t\varepsilon}{3\pi v^2} - \frac{e^2}{h}\frac{2t\varepsilon}{3\pi v^2} = \frac{e^2}{h}\frac{Q}{4\pi} - \frac{e^2}{h}\frac{t\varepsilon}{\pi v^2}. \tag{S266}$$

Thus, the kernel reads

$$\chi^{tot} = -\frac{Q}{4\pi} + \frac{t\varepsilon}{\pi v^2}, \tag{S267}$$

and then

$$\mathcal{C}_n = \int d\varepsilon[\chi^{tot}]\left(\frac{\varepsilon-\mu}{k_BT}\right)^n\left(-\frac{\partial f^0}{\partial\varepsilon}\right). \tag{S268}$$

Therefore, we have all coefficients at finite temperatures

$$\begin{aligned}
\sigma_{xy}^{tot} &= -\frac{e^2}{h}\int d\varepsilon\left(-\frac{Q}{4\pi} + \frac{t\varepsilon}{3\pi v^2}\right)\left(-\frac{\partial f^0}{\partial\varepsilon}\right), \\
\alpha_{xy}^{tot} &= \frac{k_Be}{h}\int d\varepsilon\frac{\varepsilon-\mu}{k_BT}\left(-\frac{Q}{4\pi} + \frac{t\varepsilon}{3\pi v^2}\right)\left(-\frac{\partial f^0}{\partial\varepsilon}\right), \\
\kappa_{xy}^{tot} &= -\frac{k_B^2T}{h}\int d\varepsilon\left(\frac{\varepsilon-\mu}{k_BT}\right)^2\left(-\frac{Q}{4\pi} + \frac{t\varepsilon}{3\pi v^2}\right)\left(-\frac{\partial f^0}{\partial\varepsilon}\right).
\end{aligned} \tag{S269}$$

By using the Sommerfeld expansion, we can obtain

$$\begin{aligned}
\sigma_{xy}^{tot} &= \frac{e^2}{h}\left(\frac{Q}{4\pi} - \frac{t\mu}{\pi v^2}\right), \\
\alpha_{xy}^{tot} &= \frac{k_Be}{h}\frac{\pi tk_BT}{3v^2}, \\
\kappa_{xy}^{tot} &= \frac{k_B^2T}{h}\left(\frac{\pi Q}{12} - \frac{\pi t\mu}{3v^2}\right).
\end{aligned} \tag{S270}$$

One should notice that these results are exact. Consequently, we have

$$\frac{\kappa_{xy}^{tot}}{\sigma_{xy}^{tot}} = L_0T, \tag{S271}$$

the Wiedemann-Franz law is satisfied. Similarly, we can show that the Mott relation is also satisfied

$$-eL_0T\frac{\partial\sigma_{xy}^{tot}(\mu)}{\partial\mu} = \frac{k_Be}{h}\frac{\pi tk_BT}{3v^2} = \alpha_{xy}^{tot}. \tag{S272}$$

[1] N. A. Sinitsyn, A. H. MacDonald, T. Jungwirth, V. K. Dugaev, and J. Sinova, Anomalous Hall effect in a two-dimensional Dirac band: The link between the Kubo-Streda formula and the semiclassical Boltzmann equation approach, Phys. Rev. B **75**, 045315 (2007).
[2] M. Papaj and L. Fu, Enhanced anomalous Nernst effect in disordered Dirac and Weyl materials, Phys. Rev. B **103**, 075424 (2021).
[3] N. Nagaosa, J. Sinova, S. Onoda, A. H. MacDonald, and N. P. Ong, Anomalous Hall effect, Rev. Mod. Phys. **82**, 1539 (2010).
